# Supplementary material for: Optimal estimation of generalized causal effects in cluster-randomized trials with multiple outcomes
Source: arXiv:2601.13428 ancillary file (2026-11-03)
Supplement: Supplementary file 1 [file Supplementary_Materials.pdf]

# Supplementary Materials for
# "Optimal estimation of generalized causal effects in cluster-randomized trials with multiple outcomes"

Xinyuan Chen* and Fan Li†

Section S1 gives regularity conditions and proves intermediary theoretical results for Theorems 1 and 3.
Section S2 gives the proof of Theorem 1.
Section S3 gives the proof of Theorem 2.
Section S4 gives the proof of Theorem 3.
Section S5 gives the proof of Theorem 4.
Section S6 gives the proof of Theorem 5.
Section S7 gives the additional results of simulations.
Section S8 gives results under within-cluster subsampling.

## S1 Regularity conditions and intermediary theoretical results

In this section, we present regularity conditions and prove intermediate theoretical results for Theorems 1 and 3, as these estimators can be categorized together, with different estimating functions.

### S1.1 Regularity conditions

We give regularity conditions for Theorems 1 and 3. Let $\boldsymbol{\psi}(\mathcal{O}_i, \mathcal{O}_k; \boldsymbol{\theta})$ be a vector of U-estimating functions of observed data pair $(\mathcal{O}_i, \mathcal{O}_k)$ and parameters $\boldsymbol{\theta}$. Here, $\boldsymbol{\psi}(\mathcal{O}_i, \mathcal{O}_k; \boldsymbol{\theta})$ is symmetric in $\mathcal{O}_i$ and $\mathcal{O}_k$ such that $\boldsymbol{\psi}(\mathcal{O}_i, \mathcal{O}_k; \boldsymbol{\theta}) = \boldsymbol{\psi}(\mathcal{O}_k, \mathcal{O}_i; \boldsymbol{\theta})$. The estimator $\widehat{\boldsymbol{\theta}}$ is obtained by solving

$$\sum_{1 \leq i < k \leq m} \boldsymbol{\psi}(\mathcal{O}_i, \mathcal{O}_k; \boldsymbol{\theta}) = \mathbf{0}.$$

The estimating functions we specified are defined in (4) in the main article for the nonparametric estimator and (5) in the main article for the model-robust estimator. For the proposed triply robust estimators, we denote $\boldsymbol{\psi}(\mathcal{O}_i, \mathcal{O}_k; \boldsymbol{\theta})$ as the estimating equations for parameters $\boldsymbol{\theta} = (\boldsymbol{\vartheta}, \boldsymbol{\lambda})$. We state the following regularity conditions:

(P1) $\boldsymbol{\theta} \in \boldsymbol{\Theta}$, a compact subset of the Euclidean space.

(P2) There exists a unique solution, $\underline{\boldsymbol{\theta}}$, in the interior of $\boldsymbol{\Theta}$ to the equations (moment conditions) $\mathbb{E}\{\boldsymbol{\psi}(\mathcal{O}_i, \mathcal{O}_k; \boldsymbol{\theta})\} = \mathbf{0}$.

(P3) There exists some square-integrable function $d(\mathcal{O}_i, \mathcal{O}_k)$ such that for all $\boldsymbol{\theta}, \widetilde{\boldsymbol{\theta}} \in \boldsymbol{\Theta}$,

$$\left\| \boldsymbol{\psi}(\mathcal{O}_i, \mathcal{O}_k; \boldsymbol{\theta}) - \boldsymbol{\psi}(\mathcal{O}_i, \mathcal{O}_k; \widetilde{\boldsymbol{\theta}}) \right\| \leq d(\mathcal{O}_i, \mathcal{O}_k) \left\| \boldsymbol{\theta} - \widetilde{\boldsymbol{\theta}} \right\|.$$

*xchen@math.msstate.edu
†fan.f.li@yale.edu

(P4) $\mathbb{E}\{\|\boldsymbol{\psi}(\mathcal{O}_i, \mathcal{O}_k; \boldsymbol{\theta})\|^2\} < \infty$.

(P5) The function $\boldsymbol{\psi}(\mathcal{O}_i, \mathcal{O}_k; \boldsymbol{\theta})$ is twice continuously differentiable in the support of $\boldsymbol{\theta}$, for all $\mathcal{O}_i$ and $\mathcal{O}_k$.

(P6) Define the Jacobian $\boldsymbol{B} = \mathbb{E}\{\nabla_{\boldsymbol{\theta}}\boldsymbol{\psi}(\mathcal{O}_i, \mathcal{O}_k; \boldsymbol{\theta})\}$, and assume that $\underline{\boldsymbol{B}} = \mathbb{E}\{\nabla_{\boldsymbol{\theta}}\boldsymbol{\psi}(\mathcal{O}_i, \mathcal{O}_k; \underline{\boldsymbol{\theta}})\}$ exists and is non-singular.

(P7) There exists some square-integrable function $\dot{d}(\mathcal{O}_i, \mathcal{O}_k)$ such that for all $\boldsymbol{\theta}, \widetilde{\boldsymbol{\theta}} \in \boldsymbol{\Theta}$,

$$\left\|\nabla_{\boldsymbol{\theta}}\boldsymbol{\psi}(\mathcal{O}_i, \mathcal{O}_k; \boldsymbol{\theta}) - \nabla_{\boldsymbol{\theta}}\boldsymbol{\psi}(\mathcal{O}_i, \mathcal{O}_k; \widetilde{\boldsymbol{\theta}})\right\| \leq \dot{d}(\mathcal{O}_i, \mathcal{O}_k) \left\|\boldsymbol{\theta} - \widetilde{\boldsymbol{\theta}}\right\|.$$

## S1.2 Intermediary theoretical results

**Lemma S1.** *Let $\mathcal{O}_1, \ldots, \mathcal{O}_m$ be independent and identically distributed (i.i.d.) samples from a common distribution of $\mathcal{O}$. If the regularity conditions (P1)-(P8) hold for $\boldsymbol{\psi}(\mathcal{O}_i, \mathcal{O}_k; \boldsymbol{\theta})$, then $\widehat{\boldsymbol{\theta}} \xrightarrow{p} \underline{\boldsymbol{\theta}}$ and $m^{1/2}(\widehat{\boldsymbol{\theta}} - \underline{\boldsymbol{\theta}}) \xrightarrow{d} \mathcal{N}(\mathbf{0}, \underline{\boldsymbol{V}})$, where $\underline{\boldsymbol{V}} = \underline{\boldsymbol{B}}^{-1}\underline{\boldsymbol{\Sigma}}(\underline{\boldsymbol{B}}^{-1})^\top$, with $\underline{\boldsymbol{\Sigma}} = 4\mathbb{V}\mathrm{ar}\{\overline{\boldsymbol{\psi}}(\mathcal{O}_i; \underline{\boldsymbol{\theta}})\}$. Furthermore, the sandwich variance estimator $\widehat{\boldsymbol{V}} = \widehat{\boldsymbol{B}}^{-1}\widehat{\boldsymbol{\Sigma}}(\widehat{\boldsymbol{B}}^{-1})^\top \xrightarrow{p} \underline{\boldsymbol{V}}$, where*

$$\widehat{\boldsymbol{B}} = \binom{m}{2}^{-1} \sum_{1 \leq i < k \leq m} \nabla_{\boldsymbol{\theta}}\boldsymbol{\psi}(\mathcal{O}_i, \mathcal{O}_k; \widehat{\boldsymbol{\theta}}) \quad \text{and} \quad \widehat{\boldsymbol{\Sigma}} = \frac{4}{m-1}\sum_{i=1}^{m} \widehat{\boldsymbol{\psi}}(\mathcal{O}_i; \widehat{\boldsymbol{\theta}})\widehat{\boldsymbol{\psi}}(\mathcal{O}_i; \widehat{\boldsymbol{\theta}})^\top,$$

*with $\widehat{\boldsymbol{\psi}}(\mathcal{O}_i; \widehat{\boldsymbol{\theta}}) = (m-1)^{-1}\sum_{k:k \neq i} \boldsymbol{\psi}(\mathcal{O}_i, \mathcal{O}_k; \widehat{\boldsymbol{\theta}})$.*

*Proof of Lemma S1.* We first show that $\widehat{\boldsymbol{\theta}} \xrightarrow{p} \underline{\boldsymbol{\theta}}$. By regularity conditions (P1), (P3), and (P4), Newey (1991, Corollary 4.1) implies that

$$\sup_{\boldsymbol{\theta} \in \boldsymbol{\Theta}} \left\| \binom{m}{2}^{-1} \sum_{1 \leq i < k \leq m} \boldsymbol{\psi}(\mathcal{O}_i, \mathcal{O}_k; \boldsymbol{\theta}) - \mathbb{E}\{\boldsymbol{\psi}(\mathcal{O}_i, \mathcal{O}_k; \boldsymbol{\theta})\} \right\| \xrightarrow{p} 0, \tag{S1}$$

for all $\boldsymbol{\theta} \in \boldsymbol{\Theta}$. The function $\mathbb{E}\{\boldsymbol{\psi}(\mathcal{O}_i, \mathcal{O}_k; \boldsymbol{\theta})\}$ is continuous in $\theta$ by regularity condition (P3). Then, regularity condition (P2) implies that for every $\epsilon > 0$,

$$\inf_{\|\boldsymbol{\theta} - \underline{\boldsymbol{\theta}}\| \geq \epsilon} \|\mathbb{E}\{\boldsymbol{\psi}(\mathcal{O}_i, \mathcal{O}_k; \boldsymbol{\theta})\}\| > 0. \tag{S2}$$

(S1) and (S2) allow us to apply the standard consistency argument for Z-estimators (van der Vaart, 1998, Theorem 5.9). Suppose, for contradiction, that $\widehat{\boldsymbol{\theta}}$ does not converge to $\underline{\boldsymbol{\theta}}$. Then, there exists an $\epsilon > 0$ and a subsequence $\widehat{\boldsymbol{\theta}}^*$ such that $\|\widehat{\boldsymbol{\theta}}^* - \underline{\boldsymbol{\theta}}\| \geq \epsilon$. For this subsequence,

$$\left\| \binom{m}{2}^{-1} \sum_{1 \leq i < k \leq m} \boldsymbol{\psi}(\mathcal{O}_i, \mathcal{O}_k; \widehat{\boldsymbol{\theta}}^*) \right\| \geq \inf_{\|\boldsymbol{\theta} - \underline{\boldsymbol{\theta}}\| \geq \epsilon} \|\mathbb{E}\{\boldsymbol{\psi}(\mathcal{O}_i, \mathcal{O}_k; \boldsymbol{\theta})\}\| = \delta > 0. \tag{S3}$$

However, by (S1),

$$\left\| \binom{m}{2}^{-1} \sum_{1 \leq i < k \leq m} \boldsymbol{\psi}(\mathcal{O}_i, \mathcal{O}_k; \widehat{\boldsymbol{\theta}}^*) - \mathbb{E}\left\{\boldsymbol{\psi}(\mathcal{O}_i, \mathcal{O}_k; \widehat{\boldsymbol{\theta}}^*)\right\} \right\| \xrightarrow{p} 0.$$

Since $\binom{m}{2}^{-1}\sum_{1\le i<k\le m}\boldsymbol{\psi}(\mathcal{O}_i,\mathcal{O}_k;\widehat{\boldsymbol{\theta}}^*) = 0$ by definition, it follows that $\|\mathbb{E}\{\boldsymbol{\psi}(\mathcal{O}_i,\mathcal{O}_k;\widehat{\boldsymbol{\theta}}^*)\}\| \xrightarrow{p} 0$, which contradicts (S3). Therefore, $\widehat{\boldsymbol{\theta}} \xrightarrow{p} \underline{\boldsymbol{\theta}}$.

We then show that $m^{1/2}(\widehat{\boldsymbol{\theta}}-\underline{\boldsymbol{\theta}}) \xrightarrow{d} \mathcal{N}(\mathbf{0},\underline{\boldsymbol{V}})$. By the mean value theorem

$$
\begin{aligned}
\mathbf{0} &= m^{1/2}\binom{m}{2}^{-1}\sum_{1\le i<k\le m}\boldsymbol{\psi}(\mathcal{O}_i,\mathcal{O}_k;\widehat{\boldsymbol{\theta}})\\
&= m^{1/2}\binom{m}{2}^{-1}\sum_{1\le i<k\le m}\boldsymbol{\psi}(\mathcal{O}_i,\mathcal{O}_k;\underline{\boldsymbol{\theta}}) + \binom{m}{2}^{-1}\sum_{1\le i<k\le m}\nabla_{\boldsymbol{\theta}}\boldsymbol{\psi}(\mathcal{O}_i,\mathcal{O}_k;\widetilde{\boldsymbol{\theta}})m^{1/2}(\widehat{\boldsymbol{\theta}}-\underline{\boldsymbol{\theta}}),
\end{aligned}
$$

where $\nabla_{\boldsymbol{\theta}}\boldsymbol{\psi}(\mathcal{O}_i,\mathcal{O}_k;\widetilde{\boldsymbol{\theta}})$ is $\nabla_{\boldsymbol{\theta}}\boldsymbol{\psi}(\mathcal{O}_i,\mathcal{O}_k;\boldsymbol{\theta})$ evaluated at some $\widetilde{\boldsymbol{\theta}}$ on the line segment between $\widehat{\boldsymbol{\theta}}$ and $\underline{\boldsymbol{\theta}}$. Then,

$$
\begin{aligned}
m^{1/2}(\widehat{\boldsymbol{\theta}}-\underline{\boldsymbol{\theta}}) &= -\left\{\binom{m}{2}^{-1}\sum_{1\le i<k\le m}\nabla_{\boldsymbol{\theta}}\boldsymbol{\psi}(\mathcal{O}_i,\mathcal{O}_k;\widetilde{\boldsymbol{\theta}})\right\}^{-1} m^{1/2}\binom{m}{2}^{-1}\sum_{1\le i<k\le m}\boldsymbol{\psi}(\mathcal{O}_i,\mathcal{O}_k;\underline{\boldsymbol{\theta}})\\
&= -\left[\left\{\binom{m}{2}^{-1}\sum_{1\le i<k\le m}\nabla_{\boldsymbol{\theta}}\boldsymbol{\psi}(\mathcal{O}_i,\mathcal{O}_k;\widetilde{\boldsymbol{\theta}})\right\}^{-1} - \underline{\boldsymbol{B}}^{-1} + \underline{\boldsymbol{B}}^{-1}\right] m^{1/2}\binom{m}{2}^{-1}\sum_{1\le i<k\le m}\boldsymbol{\psi}(\mathcal{O}_i,\mathcal{O}_k;\underline{\boldsymbol{\theta}})\\
&= -\underline{\boldsymbol{B}}^{-1}m^{1/2}\binom{m}{2}^{-1}\sum_{1\le i<k\le m}\boldsymbol{\psi}(\mathcal{O}_i,\mathcal{O}_k;\underline{\boldsymbol{\theta}})\\
&\quad -\left[\left\{\binom{m}{2}^{-1}\sum_{1\le i<k\le m}\nabla_{\boldsymbol{\theta}}\boldsymbol{\psi}(\mathcal{O}_i,\mathcal{O}_k;\widetilde{\boldsymbol{\theta}})\right\}^{-1} - \underline{\boldsymbol{B}}^{-1}\right] m^{1/2}\binom{m}{2}^{-1}\sum_{1\le i<k\le m}\boldsymbol{\psi}(\mathcal{O}_i,\mathcal{O}_k;\underline{\boldsymbol{\theta}})\\
&= -\underline{\boldsymbol{B}}^{-1}m^{1/2}\binom{m}{2}^{-1}\sum_{1\le i<k\le m}\boldsymbol{\psi}(\mathcal{O}_i,\mathcal{O}_k;\underline{\boldsymbol{\theta}}) + \boldsymbol{o}_{\mathbb{P}}(1)\boldsymbol{O}_{\mathbb{P}}(1)\\
&\xrightarrow{d} \mathcal{N}(\mathbf{0},\underline{\boldsymbol{V}}),
\end{aligned}
$$

where $\underline{\boldsymbol{V}} = \underline{\boldsymbol{B}}^{-1}\underline{\boldsymbol{\Sigma}}(\underline{\boldsymbol{B}}^{-1})^\top$, with $\underline{\boldsymbol{\Sigma}} = 4\mathbb{V}\mathrm{ar}\{\overline{\boldsymbol{\psi}}(\mathcal{O}_i;\underline{\boldsymbol{\theta}})\} = 4\mathbb{V}\mathrm{ar}[\mathbb{E}\{\boldsymbol{\psi}(\mathcal{O}_i,\mathcal{O}_k;\underline{\boldsymbol{\theta}})|\mathcal{O}_i\}]$. The equality

$$
\left\{\binom{m}{2}^{-1}\sum_{1\le i<k\le m}\nabla_{\boldsymbol{\theta}}\boldsymbol{\psi}(\mathcal{O}_i,\mathcal{O}_k;\widetilde{\boldsymbol{\theta}})\right\}^{-1} - \underline{\boldsymbol{B}}^{-1} = \boldsymbol{o}_{\mathbb{P}}(1)
$$

results from regularity conditions (P5)-(P7), $\widehat{\boldsymbol{\theta}} \xrightarrow{p} \underline{\boldsymbol{\theta}}$, and the continuous mapping theorem. The asymptotic normality result is obtained using van der Vaart (1998, Theorem 12.3) and Slutsky's theorem.

Lastly, we show that the sandwich variance estimator $\widehat{\boldsymbol{V}} \xrightarrow{p} \underline{\boldsymbol{V}}$. The form of $\underline{\boldsymbol{V}}$ comes from applying the Hájek projection to $\binom{m}{2}^{-1}\sum_{1\le i<k\le m}\boldsymbol{\psi}(\mathcal{O}_i,\mathcal{O}_k;\underline{\boldsymbol{\theta}})$, where

$$
\binom{m}{2}^{-1}\sum_{1\le i<k\le m}\boldsymbol{\psi}(\mathcal{O}_i,\mathcal{O}_k;\underline{\boldsymbol{\theta}}) = \frac{2}{m}\sum_{i=1}^{m}\overline{\boldsymbol{\psi}}(\mathcal{O}_i;\underline{\boldsymbol{\theta}}) + \boldsymbol{o}_{\mathbb{P}}(m^{-1/2}),
$$

and

$$m^{1/2}\binom{m}{2}^{-1}\sum_{1\le i<k\le m}\boldsymbol{\psi}(\mathcal{O}_i,\mathcal{O}_k;\underline{\boldsymbol{\theta}})=\frac{2}{\sqrt{m}}\sum_{i=1}^{m}\overline{\boldsymbol{\psi}}(\mathcal{O}_i;\underline{\boldsymbol{\theta}})+\boldsymbol{o}_{\mathbb{P}}(1).$$

Then, by the central limit theorem (CLT) for an i.i.d. sequence, we have

$$\frac{2}{\sqrt{m}}\sum_{i=1}^{m}\overline{\boldsymbol{\psi}}(\mathcal{O}_i;\underline{\boldsymbol{\theta}})\xrightarrow{d}\mathcal{N}(\mathbf{0},\underline{\boldsymbol{\Sigma}}).$$

The above results also show that the influence function for $\widehat{\boldsymbol{\theta}}$ is

$$\boldsymbol{\varphi}(\mathcal{O}_i;\boldsymbol{\theta})=-2\boldsymbol{B}^{-1}\overline{\boldsymbol{\psi}}(\mathcal{O}_i;\boldsymbol{\theta}).\tag{S4}$$

The proposed sandwich estimator for $\underline{\boldsymbol{V}}$ is $\widehat{\boldsymbol{V}}=\widehat{\boldsymbol{B}}^{-1}\widehat{\boldsymbol{\Sigma}}(\widehat{\boldsymbol{B}}^{-1})^{\top}$, where

$$\widehat{\boldsymbol{B}}=\binom{m}{2}^{-1}\sum_{1\le i<k\le m}\nabla_{\boldsymbol{\theta}}\boldsymbol{\psi}(\mathcal{O}_i,\mathcal{O}_k;\widehat{\boldsymbol{\theta}})\quad\text{and}\quad\widehat{\boldsymbol{\Sigma}}=\frac{4}{m-1}\sum_{i=1}^{m}\widehat{\boldsymbol{\psi}}(\mathcal{O}_i;\widehat{\boldsymbol{\theta}})\widehat{\boldsymbol{\psi}}(\mathcal{O}_i;\widehat{\boldsymbol{\theta}})^{\top},$$

with

$$\widehat{\boldsymbol{\psi}}(\mathcal{O}_i;\widehat{\boldsymbol{\theta}})=\frac{1}{m-1}\sum_{k:k\neq i}\boldsymbol{\psi}(\mathcal{O}_i,\mathcal{O}_k;\widehat{\boldsymbol{\theta}}),$$

as $\sum_{i=1}^{m}\widehat{\boldsymbol{\psi}}(\mathcal{O}_i;\widehat{\boldsymbol{\theta}})=\mathbf{0}$ by definition. Since $\widehat{\boldsymbol{B}}\xrightarrow{p}\underline{\boldsymbol{B}}$ is a result of regularity conditions (P5)-(P7), and $\widehat{\boldsymbol{\theta}}\xrightarrow{p}\underline{\boldsymbol{\theta}}$, we can obtain $\widehat{\boldsymbol{V}}\xrightarrow{p}\underline{\boldsymbol{V}}$ by showing $\widehat{\boldsymbol{\Sigma}}\xrightarrow{p}\underline{\boldsymbol{\Sigma}}$. Because $\mathbb{E}\{\overline{\boldsymbol{\psi}}(\mathcal{O}_i;\underline{\boldsymbol{\theta}})\}=\mathbf{0}$, we have

$$\underline{\boldsymbol{\Sigma}}=4\mathbb{E}\left\{\overline{\boldsymbol{\psi}}(\mathcal{O}_i;\underline{\boldsymbol{\theta}})\overline{\boldsymbol{\psi}}(\mathcal{O}_i;\underline{\boldsymbol{\theta}})^{\top}\right\}.$$

Then, it suffices to show that

$$m^{-1}\sum_{i=1}^{m}\widehat{\boldsymbol{\psi}}(O_i;\widehat{\boldsymbol{\theta}})\widehat{\boldsymbol{\psi}}(O_i;\widehat{\boldsymbol{\theta}})^{\top}\xrightarrow{p}\mathbb{E}\left\{\overline{\boldsymbol{\psi}}(\mathcal{O}_i;\underline{\boldsymbol{\theta}})\overline{\boldsymbol{\psi}}(\mathcal{O}_i;\underline{\boldsymbol{\theta}})^{\top}\right\},$$

which can be achieved by showing

$$m^{-1}\sum_{i=1}^{m}\widehat{\boldsymbol{\psi}}(O_i;\widehat{\boldsymbol{\theta}})\widehat{\boldsymbol{\psi}}(O_i;\widehat{\boldsymbol{\theta}})^{\top}\xrightarrow{p}m^{-1}\sum_{i=1}^{m}\overline{\boldsymbol{\psi}}(\mathcal{O}_i;\underline{\boldsymbol{\theta}})\overline{\boldsymbol{\psi}}(\mathcal{O}_i;\underline{\boldsymbol{\theta}})^{\top},\tag{S5}$$

and

$$m^{-1}\sum_{i=1}^{m}\overline{\boldsymbol{\psi}}(\mathcal{O}_i;\underline{\boldsymbol{\theta}})\overline{\boldsymbol{\psi}}(\mathcal{O}_i;\underline{\boldsymbol{\theta}})^{\top}\xrightarrow{p}\mathbb{E}\left\{\overline{\boldsymbol{\psi}}(\mathcal{O}_i;\underline{\boldsymbol{\theta}})\overline{\boldsymbol{\psi}}(\mathcal{O}_i;\underline{\boldsymbol{\theta}})^{\top}\right\}.\tag{S6}$$

(S6) is an immediate result of the law of large numbers for i.i.d. samples. For (S5),

$$\begin{aligned}
&\left\| m^{-1}\sum_{i=1}^{m}\widehat{\boldsymbol{\psi}}(O_i;\widehat{\boldsymbol{\theta}})\widehat{\boldsymbol{\psi}}(O_i;\widehat{\boldsymbol{\theta}})^\top - m^{-1}\sum_{i=1}^{m}\overline{\boldsymbol{\psi}}(\mathcal{O}_i;\underline{\boldsymbol{\theta}})\overline{\boldsymbol{\psi}}(\mathcal{O}_i;\underline{\boldsymbol{\theta}})^\top \right\| \\
&= \left\| m^{-1}\sum_{i=1}^{m}\left\{\widehat{\boldsymbol{\psi}}(O_i;\widehat{\boldsymbol{\theta}})\widehat{\boldsymbol{\psi}}(O_i;\widehat{\boldsymbol{\theta}})^\top - \overline{\boldsymbol{\psi}}(\mathcal{O}_i;\underline{\boldsymbol{\theta}})\overline{\boldsymbol{\psi}}(\mathcal{O}_i;\underline{\boldsymbol{\theta}})^\top\right\} \right\| \\
&= \left\| m^{-1}\sum_{i=1}^{m}\left[\left\{\widehat{\boldsymbol{\psi}}(O_i;\widehat{\boldsymbol{\theta}}) - \overline{\boldsymbol{\psi}}(\mathcal{O}_i;\underline{\boldsymbol{\theta}})\right\}\widehat{\boldsymbol{\psi}}(O_i;\widehat{\boldsymbol{\theta}})^\top + \overline{\boldsymbol{\psi}}(\mathcal{O}_i;\underline{\boldsymbol{\theta}})\left\{\widehat{\boldsymbol{\psi}}(O_i;\widehat{\boldsymbol{\theta}}) - \overline{\boldsymbol{\psi}}(\mathcal{O}_i;\underline{\boldsymbol{\theta}})\right\}^\top\right] \right\| \\
&\leq 2m^{-1}\sum_{i=1}^{n}\left\|\widehat{\boldsymbol{\psi}}(O_i;\widehat{\boldsymbol{\theta}}) - \overline{\boldsymbol{\psi}}(\mathcal{O}_i;\underline{\boldsymbol{\theta}})\right\|\left\{\left\|\widehat{\boldsymbol{\psi}}(O_i;\widehat{\boldsymbol{\theta}})\right\| + \left\|\overline{\boldsymbol{\psi}}(\mathcal{O}_i;\underline{\boldsymbol{\theta}})\right\|\right\} \\
&\leq 2\left\{m^{-1}\sum_{i=1}^{m}\left\|\widehat{\boldsymbol{\psi}}(O_i;\widehat{\boldsymbol{\theta}}) - \overline{\boldsymbol{\psi}}(\mathcal{O}_i;\underline{\boldsymbol{\theta}})\right\|^2\right\}^{1/2}\left[m^{-1}\sum_{i=1}^{m}\left\{\left\|\widehat{\boldsymbol{\psi}}(O_i;\widehat{\boldsymbol{\theta}})\right\| + \left\|\overline{\boldsymbol{\psi}}(\mathcal{O}_i;\underline{\boldsymbol{\theta}})\right\|\right\}^2\right]^{1/2}, \qquad \text{(S7)}
\end{aligned}$$

where the second to the last line is by applying the triangle inequality and the submultiplicative property of the norm, and the last line is by the Cauchy-Schwarz inequality. Regularity condition (P3) and Jensen's inequality imply that there exists some square-integrable function $\overline{d}(\mathcal{O}_i)$ such that for all $\boldsymbol{\theta}, \widetilde{\boldsymbol{\theta}} \in \boldsymbol{\Theta}$,

$$\left\|\overline{\boldsymbol{\psi}}(\mathcal{O}_i;\boldsymbol{\theta}) - \overline{\boldsymbol{\psi}}(\mathcal{O}_i;\widetilde{\boldsymbol{\theta}})\right\| \leq \overline{d}(\mathcal{O}_i)\left\|\boldsymbol{\theta} - \widetilde{\boldsymbol{\theta}}\right\|. \qquad \text{(S8)}$$

Therefore, The first term in (S7) is $o_{\mathbb{P}}(1)$ because regularity conditions (P1) and (S8) implies that $\{\overline{\boldsymbol{\psi}}(\mathcal{O}_i;\boldsymbol{\theta}) : \boldsymbol{\theta} \in \boldsymbol{\Theta}\}$ is $\mathbb{P}$-Glivenko-Cantelli (van der Vaart, 1998, Example 19.8), which ensures that

$$\sup_{\boldsymbol{\theta}\in\boldsymbol{\Theta}}\left\|\widehat{\boldsymbol{\psi}}(\mathcal{O}_i;\boldsymbol{\theta}) - \overline{\boldsymbol{\psi}}(\mathcal{O}_i;\boldsymbol{\theta})\right\| \xrightarrow{p} 0.$$

The second term is $O_{\mathbb{P}}(1)$ by regularity condition (P4). The proof is therefore complete. □

## S2 The nonparametric estimators

*Proof of Theorem 1.* Recall that the nonparametric estimators are solutions to the following joint U-estimating equations:

$$\sum_{1\leq i<k\leq m}\psi_C^{\text{np}}(\mathcal{O}_i,\mathcal{O}_k;\boldsymbol{\lambda}) = \sum_{1\leq i<k\leq m}\left\{\begin{array}{c}\psi_{C,1}^{\text{np}}(\mathcal{O}_i,\mathcal{O}_k;\lambda_1)\\ \psi_{C,0}^{\text{np}}(\mathcal{O}_i,\mathcal{O}_k;\lambda_0)\end{array}\right\} = \mathbf{0}$$

and

$$\sum_{1\leq i<k\leq m}\psi_I^{\text{np}}(\mathcal{O}_i,\mathcal{O}_k;\boldsymbol{\lambda}) = \sum_{1\leq i<k\leq m}\left\{\begin{array}{c}\psi_{I,1}^{\text{np}}(\mathcal{O}_i,\mathcal{O}_k;\lambda_1)\\ \psi_{I,0}^{\text{np}}(\mathcal{O}_i,\mathcal{O}_k;\lambda_0)\end{array}\right\} = \mathbf{0},$$

where the estimating functions are

$$\psi_{C,a}^{\text{np}}(\mathcal{O}_i,\mathcal{O}_k;\lambda_a) = 2^{-1}\left[\frac{\mathbb{1}(A_i = a)\mathbb{1}(A_k = 1-a)}{N_iN_k}\sum_{j=1}^{N_i}\sum_{l=1}^{N_k}\{w(\mathbf{Y}_{ij},\mathbf{Y}_{kl}) - \lambda_a\}\right.$$

$$+\frac{\mathbb{1}(A_k=a)\mathbb{1}(A_i=1-a)}{N_iN_k}\sum_{j=1}^{N_i}\sum_{l=1}^{N_k}\{w(\boldsymbol{Y}_{kl},\boldsymbol{Y}_{ij})-\lambda_a\}\Bigg]$$

and

$$\psi_{I,a}^{\mathrm{np}}(\mathcal{O}_i,\mathcal{O}_k;\lambda_a)=2^{-1}\Bigg[\mathbb{1}(A_i=a)\mathbb{1}(A_k=1-a)\sum_{j=1}^{N_i}\sum_{l=1}^{N_k}\{w(\boldsymbol{Y}_{ij},\boldsymbol{Y}_{kl})-\lambda_a\}$$
$$+\mathbb{1}(A_k=a)\mathbb{1}(A_i=1-a)\sum_{j=1}^{N_i}\sum_{l=1}^{N_k}\{w(\boldsymbol{Y}_{kl},\boldsymbol{Y}_{ij})-\lambda_a\}\Bigg],$$

for $a\in\{0,1\}$. For the condition

$$\mathbb{E}\left\{\sum_{1\le i<k\le m}\psi_{C,a}^{\mathrm{np}}(\mathcal{O}_i,\mathcal{O}_k;\lambda_a)\right\}=0,$$

we can rearrange it into

$$\mathbb{E}\left\{\sum_{1\le i\neq k\le m}\frac{\mathbb{1}(A_i=a)\mathbb{1}(A_k=1-a)}{N_iN_k}\sum_{j=1}^{N_i}\sum_{l=1}^{N_k}w(\boldsymbol{Y}_{ij},\boldsymbol{Y}_{kl})\right\}=\lambda_a\mathbb{E}\left\{\sum_{1\le i\neq k\le m}\mathbb{1}(A_i=a)\mathbb{1}(A_k=1-a)\right\}.$$

Multiplied by $\{m(m-1)\}^{-1}$ on both sides and by Lemma S2, the left-hand side of the above equality is

$$\begin{aligned}&\frac{1}{m(m-1)}\sum_{1\le i\neq k\le m}\mathbb{E}\left\{\mathbb{1}(A_i=a)\mathbb{1}(A_k=1-a)\sum_{j=1}^{N_i}\sum_{l=1}^{N_k}\frac{w(\boldsymbol{Y}_{ij},\boldsymbol{Y}_{kl})}{N_iN_k}\right\}\\&=\frac{1}{m(m-1)}\sum_{1\le i\neq k\le m}\pi(1-\pi)\mathbb{E}\left[\sum_{j=1}^{N_i}\sum_{l=1}^{N_k}\frac{w\{\boldsymbol{Y}_{ij}(a),\boldsymbol{Y}_{kl}(1-a)\}}{N_iN_k}\right]\\&=\pi(1-\pi)\mathbb{E}\left[\sum_{j=1}^{N_i}\sum_{l=1}^{N_k}\frac{w\{\boldsymbol{Y}_{ij}(a),\boldsymbol{Y}_{kl}(1-a)\}}{N_iN_k}\right],\end{aligned}$$

and the right-hand side is

$$\frac{1}{m(m-1)}\sum_{1\le i\neq k\le m}\mathbb{E}\{\mathbb{1}(A_i=a)\mathbb{1}(A_k=1-a)\}=\frac{1}{m(m-1)}\sum_{1\le i\neq k\le m}\pi(1-\pi)=\pi(1-\pi).$$

Thus, this gives us

$$\lambda_a=\lambda_{C,a}=\mathbb{E}\left[\sum_{j=1}^{N_i}\sum_{l=1}^{N_k}\frac{w\{\boldsymbol{Y}_{ij}(a),\boldsymbol{Y}_{kl}(1-a)\}}{N_iN_k}\right].$$

By Lemma S1 and under the regularity conditions, we have the consistency and asymptotic normality for $\widehat{\boldsymbol{\lambda}}_C^{\mathrm{np}}$. The consistent estimator for the asymptotic covariance matrix of $m^{1/2}\widehat{\boldsymbol{\lambda}}_C^{\mathrm{np}}$ is $\widehat{\boldsymbol{V}}_C^{\mathrm{np}} = (\widehat{\boldsymbol{B}}_C^{\mathrm{np}})^{-1}\widehat{\boldsymbol{\Sigma}}_C^{\mathrm{np}}\{(\widehat{\boldsymbol{B}}_C^{\mathrm{np}})^{-1}\}^\top$, where

$$\widehat{\boldsymbol{B}}_C^{\mathrm{np}} = \binom{m}{2}^{-1} \sum_{1\le i<k\le m} \nabla_{\boldsymbol{\lambda}} \boldsymbol{\psi}_C^{\mathrm{np}}(\mathcal{O}_i, \mathcal{O}_k; \widehat{\boldsymbol{\lambda}}_C^{\mathrm{np}}) \quad \text{and} \quad \widehat{\boldsymbol{\Sigma}}_C^{\mathrm{np}} = \frac{4}{m-1}\sum_{i=1}^m \widehat{\boldsymbol{\psi}}_C^{\mathrm{np}}(\mathcal{O}_i; \widehat{\boldsymbol{\lambda}}_C^{\mathrm{np}}) \widehat{\boldsymbol{\psi}}_C^{\mathrm{np}}(\mathcal{O}_i; \widehat{\boldsymbol{\lambda}}_C^{\mathrm{np}})^\top,$$

with

$$\widehat{\boldsymbol{\psi}}_C^{\mathrm{np}}(\mathcal{O}_i; \widehat{\boldsymbol{\lambda}}_C^{\mathrm{np}}) = \frac{1}{m-1}\sum_{k:k\neq i} \boldsymbol{\psi}_C^{\mathrm{np}}(\mathcal{O}_i, \mathcal{O}_k; \widehat{\boldsymbol{\lambda}}_C^{\mathrm{np}}).$$

The consistency and asymptotic normality of $\widehat{\Lambda}_C^{\mathrm{np}} = f(\widehat{\lambda}_{C,1}^{\mathrm{np}}, \widehat{\lambda}_{C,0}^{\mathrm{np}})$ can be obtained via the continuous mapping theorem. The consistency of $\widehat{V}_C^{\mathrm{np}}$, the asymptotic variance estimator for $\widehat{\Lambda}_C^{\mathrm{np}}$, can be obtained by applying the Delta method to $\widehat{\boldsymbol{V}}_C^{\mathrm{np}}$, and Slutsky's theorem implies the result stated in the theorem. For $\widehat{\boldsymbol{\lambda}}_I^{\mathrm{np}}$ and $\widehat{\boldsymbol{V}}_I^{\mathrm{np}}$, it suffices to investigate the condition

$$\mathbb{E}\left\{ \sum_{1\le i<k\le m} \psi_{I,a}^{\mathrm{np}}(\mathcal{O}_i, \mathcal{O}_k; \lambda_a) \right\} = 0,$$

which is rearranged into

$$\mathbb{E}\left\{ \sum_{1\le i\neq k\le m} \mathbb{1}(A_i = a)\mathbb{1}(A_k = 1-a) \sum_{j=1}^{N_i}\sum_{l=1}^{N_k} w(\mathbf{Y}_{ij}, \mathbf{Y}_{kl}) \right\} = \lambda_a \mathbb{E}\left\{ \sum_{1\le i\neq k\le m} \mathbb{1}(A_i = a)\mathbb{1}(A_k = 1-a) N_i N_k \right\}.$$

Similar to the previous derivations for the cp-GCE, the left-hand side of the above equality can be shown to be

$$\pi(1-\pi)\mathbb{E}\left[ \sum_{j=1}^{N_i}\sum_{l=1}^{N_k} w\{\mathbf{Y}_{ij}(a), \mathbf{Y}_{kl}(1-a)\} \right],$$

and the right-hand side is $\pi(1-\pi)\mathbb{E}(N_i N_k)$, which gives us

$$\lambda_a = \lambda_{I,a} = \frac{\mathbb{E}\left[ \sum_{j=1}^{N_i}\sum_{l=1}^{N_k} w\{\mathbf{Y}_{ij}(a), \mathbf{Y}_{kl}(1-a)\} \right]}{\mathbb{E}(N_i N_k)}.$$

The desired results for $\widehat{\Lambda}_I^{\mathrm{np}}$ and $\widehat{V}_I^{\mathrm{np}}$ are obtained following the same arguments for $\widehat{\Lambda}_C^{\mathrm{np}}$ and $\widehat{V}_C^{\mathrm{np}}$. The proof is complete. □

# S3 The efficient influence functions

*Proof of Theorem 3.* We derive efficient influence functions (EIFs) for the cp- and ip-GCE. We first derive the EIF for

$$\lambda_{C,a} = \mathbb{E}\left[\overline{w}\{\mathbf{Y}_i(a), \mathbf{Y}_k(1-a)\}\right].$$

By the iterative conditional expectation,

$$
\begin{aligned}
\lambda_{C,a} &= \mathbb{E}\left[\overline{w}\{\mathbf{Y}_i(a), \mathbf{Y}_k(1-a)\}\right] \\
&= \mathbb{E}\left(\mathbb{E}\left[\overline{w}\{\mathbf{Y}_i(a), \mathbf{Y}_k(1-a)\}|N_i, N_k\right]\right) \\
&= \mathbb{E}\left(\mathbb{E}\left[\mathbb{E}\left\{\overline{w}(\mathbf{Y}_i, \mathbf{Y}_k)|A_i = a, A_k = 1-a, N_i, N_k, \boldsymbol{C}_i, \boldsymbol{C}_k\right\}|N_i, N_k\right]\right) \\
&= \mathbb{E}\left\{\mathbb{E}\left(\mathbb{E}\left[\mathbb{E}\left\{\overline{w}(\mathbf{Y}_i, \mathbf{Y}_k)\middle| \begin{array}{c} A_i, \mathbf{X}_i, N_i, \boldsymbol{C}_i, \\ A_k, \mathbf{X}_k, N_k, \boldsymbol{C}_k \end{array}\right\}\middle| \begin{array}{c} A_i, N_i, \boldsymbol{C}_i, \\ A_k, N_k, \boldsymbol{C}_k \end{array}\right]\middle| N_i, N_k\right)\right\}.
\end{aligned}
$$

We use the point contamination approach (Hines et al., 2022) to derive the EIFs, where for $\mathcal{O}$ and its density function $f(o)$, the point contaminated density $f_t(o) = t\mathbb{1}_{\tilde{\mathcal{O}}}(o)+(1-t)f(o)$. The observed data for cluster $i$ is $\mathcal{O}_i = (\mathbf{Y}_i, \mathbf{X}_i, A_i, N_i, \boldsymbol{C}_i)$, the distribution of which is

$$
\mathcal{P}(\mathcal{O}) = \mathcal{P}(\mathbf{Y}|\mathbf{X}, A, N, \boldsymbol{C})\mathcal{P}(\mathbf{X}|N, \boldsymbol{C})\mathcal{P}(\boldsymbol{C}|N)\mathcal{P}(N)\mathcal{P}(A).
$$

Define

$$
\begin{aligned}
\Psi_{C,a,a}(\mathcal{P}) = \int_n\int_{\mathbf{c}}\int_{\mathbf{x}}\int_{\mathbf{y}} &\overline{w}(\mathbf{y}_i, \mathbf{y}_k)f(\mathbf{y}_i|\mathbf{x}_i, \boldsymbol{c}_i, n_i, a)f(\mathbf{y}_k|\mathbf{x}_k, \boldsymbol{c}_k, n_k, 1-a)f(\mathbf{x}_i|\boldsymbol{c}_i, n_i)f(\mathbf{x}_k|\boldsymbol{c}_k, n_k) \\
&\times f(\boldsymbol{c}_i|n_i)f(\boldsymbol{c}_k|n_k)f(n_i)f(n_k)\mathrm{d}\mathbf{y}\mathrm{d}\mathbf{x}\mathrm{d}\boldsymbol{c}\mathrm{d}n,
\end{aligned}
$$

and

$$
\begin{aligned}
\Psi_{C,a,1-a}(\mathcal{P}) = \int_n\int_{\mathbf{c}}\int_{\mathbf{x}}\int_{\mathbf{y}} &\overline{w}(\mathbf{y}_k, \mathbf{y}_i)f(\mathbf{y}_i|\mathbf{x}_i, \boldsymbol{c}_i, n_i, 1-a)f(\mathbf{y}_k|\mathbf{x}_k, \boldsymbol{c}_k, n_k, a)f(\mathbf{x}_i|\boldsymbol{c}_i, n_i)f(\mathbf{x}_k|\boldsymbol{c}_k, n_k) \\
&\times f(\boldsymbol{c}_i|n_i)f(\boldsymbol{c}_k|n_k)f(n_i)f(n_k)\mathrm{d}\mathbf{y}\mathrm{d}\mathbf{x}\mathrm{d}\boldsymbol{c}\mathrm{d}n,
\end{aligned}
$$

with

$$
\begin{aligned}
\Psi_{C,a,a}(\mathcal{P}_t) = \int_n\int_{\mathbf{c}}\int_{\mathbf{x}}\int_{\mathbf{y}} &\overline{w}(\mathbf{y}_i, \mathbf{y}_k)f_t(\mathbf{y}_i|\mathbf{x}_i, \boldsymbol{c}_i, n_i, a)f(\mathbf{y}_k|\mathbf{x}_k, \boldsymbol{c}_k, n_k, 1-a)f_t(\mathbf{x}_i|\boldsymbol{c}_i, n_i)f(\mathbf{x}_k|\boldsymbol{c}_k, n_k) \\
&\times f_t(\boldsymbol{c}_i|n_i)f(\boldsymbol{c}_k|n_k)f_t(n_i)f(n_k)\mathrm{d}\mathbf{y}\mathrm{d}\mathbf{x}\mathrm{d}\boldsymbol{c}\mathrm{d}n,
\end{aligned}
$$

and

$$
\begin{aligned}
\Psi_{C,a,1-a}(\mathcal{P}_t) = \int_n\int_{\mathbf{c}}\int_{\mathbf{x}}\int_{\mathbf{y}} &\overline{w}(\mathbf{y}_k, \mathbf{y}_i)f_t(\mathbf{y}_i|\mathbf{x}_i, \boldsymbol{c}_i, n_i, 1-a)f(\mathbf{y}_k|\mathbf{x}_k, \boldsymbol{c}_k, n_k, a)f_t(\mathbf{x}_i|\boldsymbol{c}_i, n_i)f(\mathbf{x}_k|\boldsymbol{c}_k, n_k) \\
&\times f_t(\boldsymbol{c}_i|n_i)f(\boldsymbol{c}_k|n_k)f_t(n_i)f(n_k)\mathrm{d}\mathbf{y}\mathrm{d}\mathbf{x}\mathrm{d}\boldsymbol{c}\mathrm{d}n.
\end{aligned}
$$

The EIF, defined as the Gâteaux derivative (Hines et al., 2022), is

$$
\varphi^{\text{eff}}_{C,a}(\mathcal{O}) = \frac{\mathrm{d}}{\mathrm{d}t}\Psi_{C,a,a}(\mathcal{P}_t)\bigg|_{t=0} + \frac{\mathrm{d}}{\mathrm{d}t}\Psi_{C,a,1-a}(\mathcal{P}_t)\bigg|_{t=0}.
$$

Then, by the chain rule, we have

$$
\begin{aligned}
&\frac{\mathrm{d}}{\mathrm{d}t}\Psi_{C,a,a}(\mathcal{P}_t)\bigg|_{t=0} \\
&= \int_n \int_{\boldsymbol{c}} \int_{\mathbf{x}} \int_{\mathbf{y}} \overline{w}(\mathbf{y}_i, \mathbf{y}_k) \left\{ \frac{\mathrm{d}}{\mathrm{d}t} f_t(\mathbf{y}_i | \mathbf{x}_i, \boldsymbol{c}_i, n_i, a)\bigg|_{t=0} \right\} f(\mathbf{y}_k | \mathbf{x}_k, \boldsymbol{c}_k, n_k, 1-a) f(\mathbf{x}_i | \boldsymbol{c}_i, n_i) \\
&\qquad\qquad \times f(\mathbf{x}_k | \boldsymbol{c}_k, n_k) f(\boldsymbol{c}_i | n_i) f(\boldsymbol{c}_k | n_k) f(n_i) f(n_k) \mathrm{d}\mathbf{y} \mathrm{d}\mathbf{x} \mathrm{d}\boldsymbol{c} \mathrm{d}n \\
&\quad + \int_n \int_{\boldsymbol{c}} \int_{\mathbf{x}} \int_{\mathbf{y}} \overline{w}(\mathbf{y}_i, \mathbf{y}_k) f(\mathbf{y}_i | \mathbf{x}_i, \boldsymbol{c}_i, n_i, a) f(\mathbf{y}_k | \mathbf{x}_k, \boldsymbol{c}_k, n_k, 1-a) \left\{ \frac{\mathrm{d}}{\mathrm{d}t} f_t(\mathbf{x}_i | \boldsymbol{c}_i, n_i)\bigg|_{t=0} \right\} \\
&\qquad\qquad \times f(\mathbf{x}_k | \boldsymbol{c}_k, n_k) f(\boldsymbol{c}_i | n_i) f(\boldsymbol{c}_k | n_k) f(n_i) f(n_k) \mathrm{d}\mathbf{y} \mathrm{d}\mathbf{x} \mathrm{d}m \mathrm{d}\boldsymbol{c} \mathrm{d}n \\
&\quad + \int_n \int_{\boldsymbol{c}} \int_{\mathbf{x}} \int_{\mathbf{y}} \overline{w}(\mathbf{y}_i, \mathbf{y}_k) f(\mathbf{y}_i | \mathbf{x}_i, \boldsymbol{c}_i, n_i, a) f(\mathbf{y}_k | \mathbf{x}_k, \boldsymbol{c}_k, n_k, 1-a) f(\mathbf{x}_i | \boldsymbol{c}_i, n_i) f(\mathbf{x}_k | \boldsymbol{c}_k, n_k) \\
&\qquad\qquad \times \left\{ \frac{\mathrm{d}}{\mathrm{d}t} f_t(\boldsymbol{c}_i | n_i)\bigg|_{t=0} \right\} f(\boldsymbol{c}_k | n_k) f(n_i) f(n_k) \mathrm{d}\mathbf{y} \mathrm{d}\mathbf{x} \mathrm{d}\boldsymbol{c} \mathrm{d}n \\
&\quad + \int_n \int_{\boldsymbol{c}} \int_{\mathbf{x}} \int_{\mathbf{y}} \overline{w}(\mathbf{y}_i, \mathbf{y}_k) f(\mathbf{y}_i | \mathbf{x}_i, \boldsymbol{c}_i, n_i, a) f(\mathbf{y}_k | \mathbf{x}_k, \boldsymbol{c}_k, n_k, 1-a) f(\mathbf{x}_i | \boldsymbol{c}_i, n_i) f(\mathbf{x}_k | \boldsymbol{c}_k, n_k) \\
&\qquad\qquad \times \frac{\mathrm{d}}{\mathrm{d}t} f(\boldsymbol{c}_i | n_i) f(\boldsymbol{c}_k | n_k) \left\{ f_t(n_i)\bigg|_{t=0} \right\} f(n_k) \mathrm{d}\mathbf{y} \mathrm{d}\mathbf{x} \mathrm{d}\boldsymbol{c} \mathrm{d}n.
\end{aligned}
$$

The first term,

$$
\begin{aligned}
\frac{\mathrm{d}}{\mathrm{d}t} f_t(\mathbf{y}_i | \mathbf{x}_i, \boldsymbol{c}_i, n_i, a)\bigg|_{t=0} &= \frac{\mathrm{d}}{\mathrm{d}t} \frac{f_t(\mathbf{y}_i, \mathbf{x}_i, \boldsymbol{c}_i, n_i, a)}{f_t(\mathbf{x}_i, \boldsymbol{c}_i, n_i, a)}\bigg|_{t=0} \\
= \frac{f(\mathbf{y}_i, \mathbf{x}_i, \boldsymbol{c}_i, n_i, a)}{f(\mathbf{x}_i, \boldsymbol{c}_i, n_i, a)} &\left\{ \frac{\mathbb{1}_{\tilde{\mathbf{Y}}_i}(\mathbf{y}_i) \mathbb{1}_{\tilde{\mathbf{X}}_i}(\mathbf{x}_i) \mathbb{1}_{\tilde{\boldsymbol{C}}_i}(\boldsymbol{c}_i) \mathbb{1}_{\tilde{N}_i}(n_i) \mathbb{1}_{\tilde{A}_i}(a)}{f(\mathbf{y}_i, \mathbf{x}_i, \boldsymbol{c}_i, n_i, a)} - \frac{\mathbb{1}_{\tilde{\mathbf{X}}_i}(\mathbf{x}_i) \mathbb{1}_{\tilde{\boldsymbol{C}}_i}(\boldsymbol{c}_i) \mathbb{1}_{\tilde{N}_i}(n_i) \mathbb{1}_{\tilde{A}_i}(a)}{f(\mathbf{x}_i, \boldsymbol{c}_i, n_i, a)} \right\}.
\end{aligned}
$$

The second term,

$$
\frac{\mathrm{d}}{\mathrm{d}t} f_t(\mathbf{x}_i | \boldsymbol{c}_i, n_i)\bigg|_{t=0} = \frac{\mathrm{d}}{\mathrm{d}t} \frac{f_t(\mathbf{x}_i, \boldsymbol{c}_i, n_i)}{f_t(\boldsymbol{c}_i, n_i)}\bigg|_{t=0} = \frac{f(\mathbf{x}_i, \boldsymbol{c}_i, n_i)}{f(\boldsymbol{c}_i, n_i)} \left\{ \frac{\mathbb{1}_{\tilde{\mathbf{X}}_i}(\mathbf{x}_i) \mathbb{1}_{\tilde{\boldsymbol{C}}_i}(\boldsymbol{c}_i) \mathbb{1}_{\tilde{N}_i}(n_i)}{f(\mathbf{x}_i, \boldsymbol{c}_i, n_i)} - \frac{\mathbb{1}_{\tilde{\boldsymbol{C}}_i}(\boldsymbol{c}_i) \mathbb{1}_{\tilde{N}_i}(n_i)}{f(\boldsymbol{c}_i, n_i)} \right\}.
$$

The third term,

$$
\frac{\mathrm{d}}{\mathrm{d}t} f_t(\boldsymbol{c}_i | n_i)\bigg|_{t=0} = \frac{\mathrm{d}}{\mathrm{d}t} \frac{f_t(\boldsymbol{c}_i, n_i)}{f_t(n_i)}\bigg|_{t=0} = \frac{f(\boldsymbol{c}_i, n_i)}{f(n_i)} \left\{ \frac{\mathbb{1}_{\tilde{\boldsymbol{C}}_i}(\boldsymbol{c}_i) \mathbb{1}_{\tilde{N}_i}(n_i)}{f(\boldsymbol{c}_i, n_i)} - \frac{\mathbb{1}_{\tilde{N}_i}(n_i)}{f(n_i)} \right\}.
$$

And, the last term,

$$
\frac{\mathrm{d}}{\mathrm{d}t} f_t(n_i)\bigg|_{t=0} = \mathbb{1}_{\tilde{N}_i}(n_i) - f(n_i).
$$

Putting all things together,

$$
\begin{aligned}
\frac{\mathrm{d}}{\mathrm{d}t}\Psi_{C,a,a}(\mathcal{P}_t)\bigg|_{t=0} = \frac{\mathbb{1}(\tilde{A}_i = a)}{\pi^a (1-\pi)^{1-a}} &\left[ \mathbb{E}\left\{ \overline{w}(\tilde{\mathbf{Y}}_i, \mathbf{Y}_k) \middle| A_i = a \right\} - \mathbb{E}\left\{ \overline{w}(\mathbf{Y}_i, \mathbf{Y}_k) \middle| \tilde{\mathbf{X}}_i, \tilde{C}_i, \tilde{N}_i, A_i = a \right\} \right] \\
&+ \mathbb{E}\left\{ \overline{w}(\mathbf{Y}_i, \mathbf{Y}_k) \middle| \tilde{\mathbf{X}}_i, \tilde{\boldsymbol{C}}_i, \tilde{N}_i, A_i = a \right\} - \Psi_{C,a,a}(\mathcal{P}).
\end{aligned}
$$

Similarly,

$$\frac{\mathrm{d}}{\mathrm{d}t}\Psi_{C,a,1-a}(\mathcal{P}_t)\bigg|_{t=0} = \frac{\mathbb{1}(\tilde{A}_i = 1-a)}{\pi^{1-a}(1-\pi)^a}\left[\mathbb{E}\left\{\overline{w}(\mathbf{Y}_k, \tilde{\mathbf{Y}}_i)\Big| A_i = 1-a\right\} - \mathbb{E}\left\{\overline{w}(\mathbf{Y}_k, \mathbf{Y}_i)\Big|\tilde{\mathbf{X}}_i, \tilde{\boldsymbol{C}}_i, \tilde{N}_i, A_i = 1-a\right\}\right]$$
$$+ \mathbb{E}\left\{\overline{w}(\mathbf{Y}_k, \mathbf{Y}_i)\Big|\tilde{\mathbf{X}}_i, \tilde{\boldsymbol{C}}_i, \tilde{N}_i, A_i = 1-a\right\} - \Psi_{C,a,1-a}(\mathcal{P}).$$

Then, define

$$\mathfrak{w}_{C,a,a}(\mathbf{y}) = \mathbb{E}\left\{\overline{w}(\mathbf{y}, \mathbf{Y}_k)|A_k = 1-a\right\} \quad \text{and} \quad \mathfrak{w}_{C,a,1-a}(\mathbf{y}) = \mathbb{E}\left\{\overline{w}(\mathbf{Y}_k, \mathbf{y})|A_k = a\right\},$$

and the EIF for $\lambda_{C,a}$ is

$$\varphi^{\text{eff}}_{C,a}(\mathcal{O}) = \frac{\mathbb{1}(A=a)}{\pi^a(1-\pi)^{1-a}}\left[\mathfrak{w}_{C,a,a}(\mathbf{Y}) - \mathbb{E}\left\{\mathfrak{w}_{C,a,a}(\mathbf{Y})|\mathbf{X}, \boldsymbol{C}, N, A=a\right\}\right]$$
$$+ \frac{\mathbb{1}(A=1-a)}{\pi^{1-a}(1-\pi)^a}\left[\mathfrak{w}_{C,a,1-a}(\mathbf{Y}) - \mathbb{E}\left\{\mathfrak{w}_{C,a,1-a}(\mathbf{Y})|\mathbf{X}, \boldsymbol{C}, N, A=1-a\right\}\right]$$
$$+ \mathbb{E}\left\{\mathfrak{w}_{C,a,a}(\mathbf{Y})|\mathbf{X}, \boldsymbol{C}, N, A=a\right\} + \mathbb{E}\left\{\mathfrak{w}_{C,a,1-a}(\mathbf{Y})|\mathbf{X}, \boldsymbol{C}, N, A=1-a\right\} - 2\lambda_{C,a},$$

which reduces to the EIF in Mao (2017) as a special case when $N_i = N_k = 1$ (independent data). We then derive the EIF for the ip-GCE

$$\lambda_{I,a} = \frac{\mathbb{E}[N_i N_k \overline{w}\{\mathbf{Y}_i(a), \mathbf{Y}_k(1-a)\}]}{\mathbb{E}(N_i N_k)},$$

where $\lambda_{I,a} = \lambda^{\text{num}}_{I,a}/\lambda^{\text{den}}_{I}$, with $\lambda^{\text{num}}_{I,a} = \mathbb{E}[N_i N_k \overline{w}\{\mathbf{Y}_i(a), \mathbf{Y}_k(1-a)\}]$ and $\lambda^{\text{den}}_I = \mathbb{E}(N_i N_k)$. The EIF for $\lambda_{I,a}$ is in the form of

$$\varphi^{\text{eff}}_{I,a}(\mathcal{O}) = \frac{1}{\lambda^{\text{den}}_I}\varphi^{\text{eff-num}}_{I,a}(\mathcal{O}) - \frac{\lambda_{I,a}}{\lambda^{\text{den}}_I}\varphi^{\text{eff-den}}_I(\mathcal{O}),$$

where $\varphi^{\text{eff-num}}_{I,1}(\mathcal{O})$ is the EIF for $\lambda^{\text{num}}_{I,a}$ and $\varphi^{\text{eff-den}}_I(\mathcal{O})$ is the EIF for $\lambda^{\text{den}}_I$. Similar to the derivations for the cp-GCE, define

$$\Psi_{I,a,a}(\mathcal{P}) = \int_n\int_{\boldsymbol{c}}\int_{\mathbf{x}}\int_{\mathbf{y}} n_i n_k \overline{w}(\mathbf{y}_i, \mathbf{y}_k) f(\mathbf{y}_i|\mathbf{x}_i, \boldsymbol{c}_i, n_i, a) f(\mathbf{y}_k|\mathbf{x}_k, \boldsymbol{c}_k, n_k, 1-a) f(\mathbf{x}_i|\boldsymbol{c}_i, n_i) f(\mathbf{x}_k|\boldsymbol{c}_k, n_k)$$
$$\times f(\boldsymbol{c}_i|n_i) f(\boldsymbol{c}_k|n_k) f(n_i) f(n_k) \mathrm{d}\mathbf{y}\mathrm{d}\mathbf{x}\mathrm{d}\boldsymbol{c}\mathrm{d}n,$$

and

$$\Psi_{I,a,1-a}(\mathcal{P}) = \int_n\int_{\boldsymbol{c}}\int_{\mathbf{x}}\int_{\mathbf{y}} n_i n_k \overline{w}(\mathbf{y}_k, \mathbf{y}_i) f(\mathbf{y}_i|\mathbf{x}_i, \boldsymbol{c}_i, n_i, 1-a) f(\mathbf{y}_k|\mathbf{x}_k, \boldsymbol{c}_k, n_k, a) f(\mathbf{x}_i|\boldsymbol{c}_i, n_i) f(\mathbf{x}_k|\boldsymbol{c}_k, n_k)$$
$$\times f(\boldsymbol{c}_i|n_i) f(\boldsymbol{c}_k|n_k) f(n_i) f(n_k) \mathrm{d}\mathbf{y}\mathrm{d}\mathbf{x}\mathrm{d}\boldsymbol{c}\mathrm{d}n,$$

with

$$\Psi_{I,a,a}(\mathcal{P}_t) = \int_n\int_{\boldsymbol{c}}\int_{\mathbf{x}}\int_{\mathbf{y}} n_i n_k \overline{w}(\mathbf{y}_i, \mathbf{y}_k) f_t(\mathbf{y}_i|\mathbf{x}_i, \boldsymbol{c}_i, n_i, a) f(\mathbf{y}_k|\mathbf{x}_k, \boldsymbol{c}_k, n_k, 1-a) f_t(\mathbf{x}_i|\boldsymbol{c}_i, n_i) f(\mathbf{x}_k|\boldsymbol{c}_k, n_k)$$

$$\times f_t(\boldsymbol{c}_i|n_i)f(\boldsymbol{c}_k|n_k)f_t(n_i)f(n_k)\mathrm{d}\mathbf{y}\mathrm{d}\mathbf{x}\mathrm{d}\boldsymbol{c}\mathrm{d}n,$$

and

$$\Psi_{I,a,1-a}(\mathcal{P}_t) = \int_n\int_{\mathbf{c}}\int_{\mathbf{x}}\int_{\mathbf{y}} n_i n_k \overline{w}(\mathbf{y}_k,\mathbf{y}_i) f_t(\mathbf{y}_i|\mathbf{x}_i,\boldsymbol{c}_i,n_i,1-a)f(\mathbf{y}_k|\mathbf{x}_k,\boldsymbol{c}_k,n_k,a)f_t(\mathbf{x}_i|\boldsymbol{c}_i,n_i)f(\mathbf{x}_k|\boldsymbol{c}_k,n_k)$$
$$\times f_t(\boldsymbol{c}_i|n_i)f(\boldsymbol{c}_k|n_k)f_t(n_i)f(n_k)\mathrm{d}\mathbf{y}\mathrm{d}\mathbf{x}\mathrm{d}\boldsymbol{c}\mathrm{d}n.$$

The EIF for $\lambda_{I,a}^{\text{num}}$ is

$$\varphi_{I,a}^{\text{eff-num}}(\mathcal{O}) = \frac{\mathrm{d}}{\mathrm{d}t}\Psi_{I,a,a}(\mathcal{P}_t)\Big|_{t=0} + \frac{\mathrm{d}}{\mathrm{d}t}\Psi_{I,a,1-a}(\mathcal{P}_t)\Big|_{t=0},$$

which, via similar derivations, is

$$\begin{aligned}\varphi_{I,a}^{\text{eff-num}}(\mathcal{O}) = &\frac{\mathbb{1}(A=a)N}{\pi^a(1-\pi)^{1-a}}\left[\mathfrak{w}_{I,a,a}(\mathbf{Y}) - \mathbb{E}\left\{\mathfrak{w}_{I,a,a}(\mathbf{Y})|\mathbf{X},\boldsymbol{C},N,A=a\right\}\right] \\ &+ \frac{\mathbb{1}(A=1-a)N}{\pi^{1-a}(1-\pi)^{a}}\left[\mathfrak{w}_{I,a,1-a}(\mathbf{Y}) - \mathbb{E}\left\{\mathfrak{w}_{I,a,1-a}(\mathbf{Y})|\mathbf{X},\boldsymbol{C},N,A=1-a\right\}\right] \\ &+ N\mathbb{E}\left\{\mathfrak{w}_{I,a,a}(\mathbf{Y})|\mathbf{X},\boldsymbol{C},N,A=a\right\} + N\mathbb{E}\left\{\mathfrak{w}_{I,a,1-a}(\mathbf{Y})|\mathbf{X},\boldsymbol{C},N,A=1-a\right\} - 2\lambda_{I,a}^{\text{num}},\end{aligned}$$

with

$$\mathfrak{w}_{I,a,a}(\mathbf{y}) = \mathbb{E}\left\{N_k\overline{w}(\mathbf{y},\mathbf{Y}_k)|A_k=1-a\right\} \quad \text{and} \quad \mathfrak{w}_{I,a,1-a}(\mathbf{y}) = \mathbb{E}\left\{N_k\overline{w}(\mathbf{Y}_k,\mathbf{y})|A_k=a\right\}.$$

The EIF for $\lambda_I^{\text{den}}$ is

$$\varphi_I^{\text{eff-den}}(\mathcal{O}) = 2N\mathbb{E}(N) - 2\lambda_I^{\text{den}}.$$

Putting all things together,

$$\begin{aligned}\varphi_{I,a}^{\text{eff}}(\mathcal{O}) = &\frac{\mathbb{1}(A=a)N}{\pi^a(1-\pi)^{1-a}\{\mathbb{E}(N)\}^2}\left[\mathfrak{w}_{I,a,a}(\mathbf{Y}) - \mathbb{E}\left\{\mathfrak{w}_{I,a,a}(\mathbf{Y})|\mathbf{X},\boldsymbol{C},N,A=a\right\}\right] \\ &+ \frac{\mathbb{1}(A=1-a)N}{\pi^{1-a}(1-\pi)^{a}\{\mathbb{E}(N)\}^2}\left[\mathfrak{w}_{I,a,1-a}(\mathbf{Y}) - \mathbb{E}\left\{\mathfrak{w}_{I,a,1-a}(\mathbf{Y})|\mathbf{X},\boldsymbol{C},N,A=1-a\right\}\right] \\ &+ \frac{N}{\{\mathbb{E}(N)\}^2}\left[\mathbb{E}\left\{\mathfrak{w}_{I,a,a}(\mathbf{Y})|\mathbf{X},\boldsymbol{C},N,A=a\right\} + \mathbb{E}\left\{\mathfrak{w}_{I,a,1-a}(\mathbf{Y})|\mathbf{X},\boldsymbol{C},N,A=1-a\right\}\right] - \frac{2N\lambda_{I,a}}{\mathbb{E}(N)},\end{aligned}$$

which also reduces to the EIF in Mao (2017) as a special case when $N_i = N_k = 1$ (independent data).

After the derivations, we verify that $\varphi_{C,a}^{\text{eff}}(\mathcal{O}), \varphi_{I,a}^{\text{eff}}(\mathcal{O}) \in \mathcal{T}$, the tangent space of the observed data constrained by Assumptions 1-3 in the main article. Recall that the observed data distribution is

$$\mathcal{P}(\mathcal{O}) = \mathcal{P}(\mathbf{Y}|\mathbf{X},A,N,\boldsymbol{C})\mathcal{P}(\mathbf{X}|N,\boldsymbol{C})\mathcal{P}(\boldsymbol{C}|N)\mathcal{P}(N)\mathcal{P}(A),$$

where $\mathcal{P}(A)$ is known. Let $\mathcal{L}_{2,0}(\mathcal{O})$ denote the set of functions of a random variable $\mathcal{O}$ that have zero mean and a finite

variance, i.e.,

$$\mathcal{L}_{2,0}(\mathcal{O}) = \left\{L(\mathcal{O}) \middle| \mathbb{E}\{L(\mathcal{O})\} = 0,\ \mathbb{E}[\{L(\mathcal{O})\}^2] < \infty\right\}.$$

Then, the tangent space of the model constrained by Assumptions 1-3 is

$$\mathcal{T} = \left\{ L(\mathcal{O}) \in \mathcal{L}_{2,0}(\mathcal{O}) \;\middle|\; \begin{array}{c} L(\mathcal{O}) = L_{\mathbf{Y}}(\mathbf{Y}, \mathbf{X}, A, N, \boldsymbol{C}) + L_{\mathbf{X}}(\mathbf{X}, N, \boldsymbol{C}) \\ +L_{\boldsymbol{C}}(\boldsymbol{C}, N) + L_N(N) \end{array} \right\},$$

where

$$\mathbb{E}\{L_{\mathbf{Y}}(\mathbf{Y}, \mathbf{X}, A, N, \boldsymbol{C})|\mathbf{X}, A, N, \boldsymbol{C}\} = \mathbb{E}\{L_{\mathbf{X}}(\mathbf{X}, A, N, \boldsymbol{C})|N, \boldsymbol{C}\} = \mathbb{E}\{L_{\boldsymbol{C}}(\boldsymbol{C}, N)|N\} = \mathbb{E}\{L_N(N)\} = 0.$$

We then decompose $\varphi^{\text{eff}}_{C,a}(\mathcal{O})$ as

$$\varphi^{\text{eff}}_{C,a}(\mathcal{O}) = \varphi^{\text{eff}}_{C,a,\mathbf{Y}}(\mathbf{Y}, \mathbf{X}, A, N, \boldsymbol{C}) + \varphi^{\text{eff}}_{C,a,\mathbf{X}}(\mathbf{X}, N, \boldsymbol{C}) + \varphi^{\text{eff}}_{C,a,\boldsymbol{C}}(\boldsymbol{C}, N) + \varphi^{\text{eff}}_{C,a,N}(N),$$

where

$$\begin{aligned}
\varphi^{\text{eff}}_{C,a,\mathbf{Y}}(\mathbf{Y}, \mathbf{X}, A, N, \boldsymbol{C}) &= \frac{\mathbb{1}(A=a)}{\pi^a(1-\pi)^{1-a}}\left[\mathfrak{w}_{C,a,a}(\mathbf{Y}) - \mathbb{E}\left\{\mathfrak{w}_{C,a,a}(\mathbf{Y})|\mathbf{X}, \boldsymbol{C}, N, A=a\right\}\right] \\
&\quad + \frac{\mathbb{1}(A=1-a)}{\pi^{1-a}(1-\pi)^a}\left[\mathfrak{w}_{C,a,1-a}(\mathbf{Y}) - \mathbb{E}\left\{\mathfrak{w}_{C,a,1-a}(\mathbf{Y})|\mathbf{X}, \boldsymbol{C}, N, A=1-a\right\}\right], \\
\varphi^{\text{eff}}_{C,a,\mathbf{X}}(\mathbf{X}, N, \boldsymbol{C}) &= \mathbb{E}\left\{\mathfrak{w}_{C,a,a}(\mathbf{Y})|\mathbf{X}, \boldsymbol{C}, N, A=a\right\} + \mathbb{E}\left\{\mathfrak{w}_{C,a,1-a}(\mathbf{Y})|\mathbf{X}, \boldsymbol{C}, N, A=1-a\right\} \\
&\quad - \mathbb{E}\left\{\mathfrak{w}_{C,a,a}(\mathbf{Y})|\boldsymbol{C}, N, A=a\right\} - \mathbb{E}\left\{\mathfrak{w}_{C,a,1-a}(\mathbf{Y})|\boldsymbol{C}, N, A=1-a\right\}, \\
\varphi^{\text{eff}}_{C,a,\boldsymbol{C}}(\boldsymbol{C}, N) &= \mathbb{E}\left\{\mathfrak{w}_{C,a,a}(\mathbf{Y})|\boldsymbol{C}, N, A=a\right\} + \mathbb{E}\left\{\mathfrak{w}_{C,a,1-a}(\mathbf{Y})|\boldsymbol{C}, N, A=a\right\} \\
&\quad - \mathbb{E}\left\{\mathfrak{w}_{C,a,a}(\mathbf{Y})|\boldsymbol{C}, A=a\right\} - \mathbb{E}\left\{\mathfrak{w}_{C,a,1-a}(\mathbf{Y})|\boldsymbol{C}, A=a\right\}, \\
\varphi^{\text{eff}}_{C,a,N}(N) &= \mathbb{E}\left\{\mathfrak{w}_{C,a,a}(\mathbf{Y})|\boldsymbol{C}, A=a\right\} + \mathbb{E}\left\{\mathfrak{w}_{C,a,1-a}(\mathbf{Y})|\boldsymbol{C}, A=a\right\} - 2\lambda_{C,a}.
\end{aligned}$$

Some algebra gives us

$$\begin{aligned}
&\mathbb{E}\left\{\varphi^{\text{eff}}_{C,a,\mathbf{Y}}(\mathbf{Y}, \mathbf{X}, A, N, \boldsymbol{C})|\mathbf{X}, A, N, \boldsymbol{C}\right\} = \mathbb{E}\left\{\varphi^{\text{eff}}_{C,a,\mathbf{X}}(\mathbf{X}, A, N, \boldsymbol{C})|N, \boldsymbol{C}\right\} \\
&= \mathbb{E}\left\{\varphi^{\text{eff}}_{C,a,\boldsymbol{C}}(\boldsymbol{C}, N)|N\right\} = \mathbb{E}\left\{\varphi^{\text{eff}}_{C,a,N}(N)\right\} = 0,
\end{aligned}$$

which implies that $\varphi^{\text{eff}}_{C,a}(\mathcal{O}) \in \mathcal{T}$, completing the verification. The verification of $\varphi^{\text{eff}}_{I,a}(\mathcal{O}) \in \mathcal{T}$ follows the same process, and is thus omitted. □

# S4 The model-robust estimators

*Proof of Theorem 4.* By definition, $\widehat{\boldsymbol{\vartheta}} = (\widehat{\boldsymbol{\vartheta}}_1, \widehat{\boldsymbol{\vartheta}}_0)$ is obtained by solving estimating equations

$$\sum_{1\le i<k\le m} \boldsymbol{\psi}_{\boldsymbol{\vartheta}}(\mathcal{O}_i, \mathcal{O}_k; \boldsymbol{\vartheta}) = \sum_{1\le i<k\le m} \left\{ \begin{array}{c} \boldsymbol{\psi}_{\boldsymbol{\vartheta},1}(\mathcal{O}_i, \mathcal{O}_k; \boldsymbol{\vartheta}_1) \\ \boldsymbol{\psi}_{\boldsymbol{\vartheta},0}(\mathcal{O}_i, \mathcal{O}_k; \boldsymbol{\vartheta}_0) \end{array} \right\} = \mathbf{0}.$$

Therefore, the joint estimating equations for $(\widehat{\boldsymbol{\vartheta}}, \widehat{\boldsymbol{\lambda}}_C)$ are

$$\sum_{1\le i<k\le m} \boldsymbol{\psi}_C^{\text{eff}}(\mathcal{O}_i, \mathcal{O}_k; \boldsymbol{\vartheta}, \boldsymbol{\lambda}) = \sum_{1\le i<k\le m} \left\{ \begin{array}{l} \boldsymbol{\psi}_{\boldsymbol{\vartheta},1}(\mathcal{O}_i, \mathcal{O}_k; \boldsymbol{\vartheta}_1) \\ \boldsymbol{\psi}_{\boldsymbol{\vartheta},0}(\mathcal{O}_i, \mathcal{O}_k; \boldsymbol{\vartheta}_0) \\ \psi_{C,\boldsymbol{\lambda},1}^{\text{eff}}(\mathcal{O}_i, \mathcal{O}_k; \boldsymbol{\vartheta}, \lambda_1) \\ \psi_{C,\boldsymbol{\lambda},0}^{\text{eff}}(\mathcal{O}_i, \mathcal{O}_k; \boldsymbol{\vartheta}, \lambda_0) \end{array} \right\} = \mathbf{0},$$

where, for $a \in \{0,1\}$,

$$\begin{aligned} \psi_{C,\boldsymbol{\lambda},a}^{\text{eff}}(\mathcal{O}_i, \mathcal{O}_k; \boldsymbol{\vartheta}, \lambda_a) = 2^{-1} \Bigg[ & \frac{\mathbb{1}(A_i = a)\mathbb{1}(A_k = 1-a)}{\pi(1-\pi)} \{\overline{w}(\mathbf{Y}_i, \mathbf{Y}_k) - \zeta_{ik,a}(\boldsymbol{\vartheta}_a)\} \\ & + \frac{\mathbb{1}(A_k = a)\mathbb{1}(A_i = 1-a)}{\pi(1-\pi)} \{\overline{w}(\mathbf{Y}_k, \mathbf{Y}_i) - \zeta_{ki,a}(\boldsymbol{\vartheta}_a)\} + \zeta_{ik,a}(\boldsymbol{\vartheta}_a) + \zeta_{ki,a}(\boldsymbol{\vartheta}_a) - 2\lambda_a \Bigg]. \end{aligned}$$

Under the regularity conditions in Section S1, we have $(\widehat{\boldsymbol{\vartheta}}, \widehat{\boldsymbol{\lambda}}_C^{\text{mr}}) \xrightarrow{p} (\underline{\boldsymbol{\vartheta}}, \underline{\boldsymbol{\lambda}}_C^{\text{mr}})$ by Lemma S1, where $\underline{\boldsymbol{\lambda}}_C^{\text{mr}}$ satisfies

$$\mathbb{E}\left\{\boldsymbol{\psi}_C^{\text{eff}}(\mathcal{O}_i, \mathcal{O}_k; \underline{\boldsymbol{\vartheta}}, \underline{\boldsymbol{\lambda}}_C^{\text{mr}})\right\} = \mathbf{0}.$$

To see when $\underline{\lambda}_{C,a}^{\text{mr}} = \lambda_{C,a}$, we have,

$$\begin{aligned} & \mathbb{E}\left\{\psi_{C,a}^{\text{eff}}(\mathcal{O}_i, \mathcal{O}_k; \underline{\boldsymbol{\vartheta}}, \underline{\lambda}_{C,a}^{\text{mr}})\right\} \\ & = \mathbb{E}\left[2^{-1}\left\{\frac{\mathbb{1}(A_i = a)\mathbb{1}(A_k = 1-a)}{\pi(1-\pi)}\overline{w}(\mathbf{Y}_i, \mathbf{Y}_k) + \frac{\mathbb{1}(A_k = a)\mathbb{1}(A_i = 1-a)}{\pi(1-\pi)}\overline{w}(\mathbf{Y}_k, \mathbf{Y}_i)\right\}\right] \\ & \quad - \mathbb{E}\left[2^{-1}\left\{\frac{\mathbb{1}(A_i = a)\mathbb{1}(A_k = 1-a)}{\pi(1-\pi)}\zeta_{ik,a}(\underline{\boldsymbol{\vartheta}}_a) + \frac{\mathbb{1}(A_k = a)\mathbb{1}(A_i = 1-a)}{\pi(1-\pi)}\zeta_{ki,a}(\underline{\boldsymbol{\vartheta}}_a)\right\}\right] \\ & \quad + \mathbb{E}\left[2^{-1}\{\zeta_{ik,a}(\underline{\boldsymbol{\vartheta}}_a) + \zeta_{ki,a}(\underline{\boldsymbol{\vartheta}}_a)\}\right] - \underline{\lambda}_{C,a}^{\text{mr}} \\ & = \lambda_{C,a} - \underline{\lambda}_{C,a}^{\text{mr}}, \end{aligned}$$

implying that $\widehat{\lambda}_{C,a}^{\text{mr}}$ is consistent for $\lambda_{C,a}$ regardless whether $\zeta_a(\boldsymbol{\vartheta}_a)$ correctly specifies $\zeta_a^0$, because $\pi = \mathbb{P}(A_i = 1)$ is known in a CRE. We next prove the asymptotic normality. By the regularity conditions, Lemma S1 implies that

$$m^{1/2}(\widehat{\boldsymbol{\theta}}_C^{\text{mr}} - \underline{\boldsymbol{\theta}}_C^{\text{mr}}) = \frac{2}{\sqrt{m}} \sum_{i=1}^m \left(\underline{\boldsymbol{B}}_{C,\boldsymbol{\theta}}^{\text{mr}}\right)^{-1} \overline{\boldsymbol{\psi}}_C^{\text{eff}}(\mathcal{O}_i; \underline{\boldsymbol{\theta}}_C^{\text{mr}}) + \boldsymbol{o}_{\mathbb{P}}(1),$$

where $\widehat{\boldsymbol{\theta}}_C^{\text{mr}} = (\widehat{\boldsymbol{\vartheta}}^\top, \widehat{\boldsymbol{\lambda}}_C^{\text{mr}\prime})^\top$ and $\underline{\boldsymbol{B}}_{C,\boldsymbol{\theta}}^{\text{mr}} = \mathbb{E}\{\nabla_{\boldsymbol{\theta}} \boldsymbol{\psi}_C^{\text{eff}}(\mathcal{O}_i, \mathcal{O}_k; \underline{\boldsymbol{\theta}}_C^{\text{mr}})\}$. Thus, the asymptotic normality of $\widehat{\boldsymbol{\theta}}_C$ is obtained by the CLT. The asymptotic covariance matrix of $m^{1/2}\widehat{\boldsymbol{\theta}}_C^{\text{mr}}$ is $\underline{\boldsymbol{V}}_{C,\boldsymbol{\theta}}^{\text{mr}} = (\underline{\boldsymbol{B}}_{C,\boldsymbol{\theta}}^{\text{mr}})^{-1}\underline{\boldsymbol{\Sigma}}_{C,\boldsymbol{\theta}}^{\text{mr}}\{(\underline{\boldsymbol{B}}_{C,\boldsymbol{\theta}}^{\text{mr}})^{-1}\}^\top$, where $\underline{\boldsymbol{\Sigma}}_{C,\boldsymbol{\theta}}^{\text{mr}} = 4\mathbb{V}\text{ar}\{\overline{\boldsymbol{\psi}}_C^{\text{eff}}(\mathcal{O}_i; \underline{\boldsymbol{\theta}}_C^{\text{mr}})\}$ and $\overline{\boldsymbol{\psi}}_C^{\text{eff}}(\mathcal{O}_i; \underline{\boldsymbol{\theta}}_C^{\text{mr}}) = \mathbb{E}\{\boldsymbol{\psi}_C^{\text{eff}}(\mathcal{O}_i, \mathcal{O}_k; \underline{\boldsymbol{\theta}}_C^{\text{mr}})|\mathcal{O}_i\}$. We further investigate the influence function of $\widehat{\boldsymbol{\lambda}}_C^{\text{mr}}$ to obtain explicit expressions of the asymptotic covariance matrix and covariance estimator. Specifically, we have

$$\underline{\boldsymbol{B}}_{C,\boldsymbol{\theta}}^{\text{mr}} = \begin{pmatrix} \underline{\boldsymbol{B}}_{\boldsymbol{\vartheta}\boldsymbol{\vartheta}} & \underline{\boldsymbol{B}}_{\boldsymbol{\vartheta}\boldsymbol{\lambda}} \\ \underline{\boldsymbol{B}}_{C,\boldsymbol{\lambda}\boldsymbol{\vartheta}}^{\text{mr}} & \underline{\boldsymbol{B}}_{C,\boldsymbol{\lambda}\boldsymbol{\lambda}}^{\text{mr}} \end{pmatrix} = \begin{pmatrix} \underline{\boldsymbol{B}}_{\boldsymbol{\vartheta}\boldsymbol{\vartheta}} & \mathbf{0} \\ \underline{\boldsymbol{B}}_{C,\boldsymbol{\lambda}\boldsymbol{\vartheta}}^{\text{mr}} & \underline{\boldsymbol{B}}_{C,\boldsymbol{\lambda}\boldsymbol{\lambda}}^{\text{mr}} \end{pmatrix},$$

where $\underline{\boldsymbol{B}}_{\boldsymbol{\vartheta\vartheta}} = \mathbb{E}\{\nabla_{\boldsymbol{\vartheta}}\boldsymbol{\psi}_{\boldsymbol{\vartheta}}(\mathcal{O}_i,\mathcal{O}_k;\underline{\boldsymbol{\vartheta}})\}$, $\underline{\boldsymbol{B}}_{\boldsymbol{\vartheta\lambda}} = \mathbb{E}\{\nabla_{\boldsymbol{\lambda}}\boldsymbol{\psi}_{\boldsymbol{\vartheta}}(\mathcal{O}_i,\mathcal{O}_k;\underline{\boldsymbol{\vartheta}})\} = \mathbf{0}$, $\underline{\boldsymbol{B}}^{\mathrm{mr}}_{C,\boldsymbol{\lambda\vartheta}} = \mathbb{E}\{\nabla_{\boldsymbol{\vartheta}}\boldsymbol{\psi}^{\mathrm{eff}}_{C,\boldsymbol{\lambda}}(\mathcal{O}_i,\mathcal{O}_k;\underline{\boldsymbol{\vartheta}},\underline{\boldsymbol{\lambda}}^{\mathrm{mr}}_C)\}$, and $\underline{\boldsymbol{B}}^{\mathrm{mr}}_{C,\boldsymbol{\lambda\lambda}} = \mathbb{E}\{\nabla_{\boldsymbol{\lambda}}\boldsymbol{\psi}^{\mathrm{eff}}_{C,\boldsymbol{\lambda}}(\mathcal{O}_i,\mathcal{O}_k;\underline{\boldsymbol{\vartheta}},\underline{\boldsymbol{\lambda}}^{\mathrm{mr}}_C)\}$. Then, the inverse of the block lower-triangular matrix gives us

$$\left(\underline{\boldsymbol{B}}^{\mathrm{mr}}_{C,\boldsymbol{\theta}}\right)^{-1} = \begin{pmatrix} \underline{\boldsymbol{B}}^{-1}_{\boldsymbol{\vartheta\vartheta}} & \mathbf{0} \\ -\left(\underline{\boldsymbol{B}}^{\mathrm{mr}}_{C,\boldsymbol{\lambda\lambda}}\right)^{-1}\underline{\boldsymbol{B}}^{\mathrm{mr}}_{C,\boldsymbol{\lambda\vartheta}}\underline{\boldsymbol{B}}^{-1}_{\boldsymbol{\vartheta\vartheta}} & \left(\underline{\boldsymbol{B}}^{\mathrm{mr}}_{C,\boldsymbol{\lambda\lambda}}\right)^{-1} \end{pmatrix}.$$

Since,

$$\overline{\boldsymbol{\psi}}^{\mathrm{eff}}_C(\mathcal{O}_i;\boldsymbol{\theta}^{\mathrm{mr}}_C) = \begin{pmatrix} \overline{\boldsymbol{\psi}}_{\boldsymbol{\vartheta}}(\mathcal{O}_i;\boldsymbol{\vartheta}) \\ \overline{\boldsymbol{\psi}}^{\mathrm{eff}}_{C,\boldsymbol{\lambda}}(\mathcal{O}_i;\boldsymbol{\vartheta},\boldsymbol{\lambda}^{\mathrm{mr}}_C) \end{pmatrix},$$

by (S4), the influence function for $\widehat{\boldsymbol{\lambda}}^{\mathrm{mr}}_C$ is

$$\boldsymbol{\varphi}^{\mathrm{mr}}_C(\mathcal{O}_i;\boldsymbol{\vartheta},\boldsymbol{\lambda}^{\mathrm{mr}}_C) = -2\left(\boldsymbol{B}^{\mathrm{mr}}_{C,\boldsymbol{\lambda\lambda}}\right)^{-1}\left\{\overline{\boldsymbol{\psi}}^{\mathrm{eff}}_{C,\boldsymbol{\lambda}}(\mathcal{O}_i;\boldsymbol{\vartheta},\boldsymbol{\lambda}^{\mathrm{mr}}_C) - \boldsymbol{B}^{\mathrm{mr}}_{C,\boldsymbol{\lambda\vartheta}}\boldsymbol{B}^{-1}_{\boldsymbol{\vartheta\vartheta}}\overline{\boldsymbol{\psi}}_{\boldsymbol{\vartheta}}(\mathcal{O}_i;\boldsymbol{\vartheta})\right\}.$$

The asymptotic covariance matrix of $m^{1/2}\widehat{\boldsymbol{\lambda}}^{\mathrm{mr}}_C$ is $\underline{\boldsymbol{V}}^{\mathrm{mr}}_C = \mathbb{V}\mathrm{ar}\{\boldsymbol{\varphi}^{\mathrm{mr}}_C(\mathcal{O}_i;\underline{\boldsymbol{\vartheta}},\underline{\boldsymbol{\lambda}}^{\mathrm{mr}}_C)\}$. The covariance matrix estimator $\widehat{\boldsymbol{V}}^{\mathrm{mr}}_C = (m-1)^{-1}\sum_{i=1}^m \widehat{\boldsymbol{\varphi}}^{\mathrm{mr}}_C(\mathcal{O}_i;\widehat{\boldsymbol{\vartheta}},\widehat{\boldsymbol{\lambda}}^{\mathrm{mr}}_C)\widehat{\boldsymbol{\varphi}}^{\mathrm{mr}}_C(\mathcal{O}_i;\widehat{\boldsymbol{\vartheta}},\widehat{\boldsymbol{\lambda}}^{\mathrm{mr}}_C)^\top$, where

$$\widehat{\boldsymbol{\varphi}}^{\mathrm{mr}}_C(\mathcal{O}_i;\widehat{\boldsymbol{\vartheta}},\widehat{\boldsymbol{\lambda}}^{\mathrm{mr}}_C) = -2\left(\widehat{\boldsymbol{B}}^{\mathrm{mr}}_{C,\boldsymbol{\lambda\lambda}}\right)^{-1}\left\{\widehat{\boldsymbol{\psi}}^{\mathrm{eff}}_{C,\boldsymbol{\lambda}}(\mathcal{O}_i;\widehat{\boldsymbol{\vartheta}},\widehat{\boldsymbol{\lambda}}^{\mathrm{mr}}_C) - \widehat{\boldsymbol{B}}^{\mathrm{mr}}_{C,\boldsymbol{\lambda\vartheta}}\widehat{\boldsymbol{B}}^{-1}_{\boldsymbol{\vartheta\vartheta}}\widehat{\boldsymbol{\psi}}_{\boldsymbol{\vartheta}}(\mathcal{O}_i;\widehat{\boldsymbol{\vartheta}})\right\},$$

with

$$\widehat{\boldsymbol{B}}^{\mathrm{mr}}_{C,\boldsymbol{\lambda\lambda}} = \binom{m}{2}^{-1}\sum_{1\le i<k\le m}\nabla_{\boldsymbol{\lambda}}\boldsymbol{\psi}^{\mathrm{eff}}_{C,\boldsymbol{\lambda}}(\mathcal{O}_i,\mathcal{O}_k;\widehat{\boldsymbol{\vartheta}},\widehat{\boldsymbol{\lambda}}^{\mathrm{mr}}_C), \quad \widehat{\boldsymbol{B}}^{\mathrm{mr}}_{C,\boldsymbol{\lambda\vartheta}} = \binom{m}{2}^{-1}\sum_{1\le i<k\le m}\nabla_{\boldsymbol{\vartheta}}\boldsymbol{\psi}^{\mathrm{eff}}_{C,\boldsymbol{\lambda}}(\mathcal{O}_i,\mathcal{O}_k;\widehat{\boldsymbol{\vartheta}},\widehat{\boldsymbol{\lambda}}^{\mathrm{mr}}_C),$$
$$\widehat{\boldsymbol{B}}_{\boldsymbol{\vartheta\vartheta}} = \binom{m}{2}^{-1}\sum_{1\le i<k\le m}\nabla_{\boldsymbol{\vartheta}}\boldsymbol{\psi}_{\boldsymbol{\vartheta}}(\mathcal{O}_i,\mathcal{O}_k;\widehat{\boldsymbol{\vartheta}}), \quad \widehat{\boldsymbol{\psi}}^{\mathrm{eff}}_{C,\boldsymbol{\lambda}}(\mathcal{O}_i;\widehat{\boldsymbol{\vartheta}},\widehat{\boldsymbol{\lambda}}^{\mathrm{mr}}_C) = \frac{1}{m-1}\sum_{k:k\neq i}\boldsymbol{\psi}^{\mathrm{eff}}_{C,\boldsymbol{\lambda}}(\mathcal{O}_i,\mathcal{O}_k;\widehat{\boldsymbol{\vartheta}},\widehat{\boldsymbol{\lambda}}^{\mathrm{mr}}_C),$$
$$\widehat{\boldsymbol{\psi}}_{\boldsymbol{\vartheta}}(\mathcal{O}_i;\widehat{\boldsymbol{\vartheta}}) = \frac{1}{m-1}\sum_{k:k\neq i}\boldsymbol{\psi}_{\boldsymbol{\vartheta}}(\mathcal{O}_i,\mathcal{O}_k;\widehat{\boldsymbol{\vartheta}}).$$

The consistency and asymptotic normality of $\widehat{\Lambda}^{\mathrm{mr}}_C$ are obtained via the continuous mapping theorem. The asymptotic variance estimators of $m^{1/2}\widehat{\Lambda}^{\mathrm{mr}}_C$, $\widehat{V}^{\mathrm{mr}}_C$, can be obtained by applying the Delta method to $\widehat{\boldsymbol{V}}^{\mathrm{mr}}_C$. Lemma S1 implies that $\widehat{V}^{\mathrm{mr}}_I \xrightarrow{p} \underline{V}^{\mathrm{mr}}_I$. Slutsky's theorem implies the result in the theorem statement.

For the semiparametric efficiency statement, note that

$$\begin{aligned}\underline{\boldsymbol{B}}^{\mathrm{mr}}_{C,\boldsymbol{\lambda\vartheta}} = \mathbb{E}\left\{\nabla_{\boldsymbol{\vartheta}}\boldsymbol{\psi}^{\mathrm{eff}}_{C,\boldsymbol{\lambda}}(\mathcal{O}_i,\mathcal{O}_k;\underline{\boldsymbol{\vartheta}},\underline{\boldsymbol{\lambda}}^{\mathrm{mr}}_C)\right\} &= \mathbb{E}\left[\nabla_{\boldsymbol{\vartheta}}\mathbb{E}\left\{\boldsymbol{\psi}^{\mathrm{eff}}_{C,\boldsymbol{\lambda}}(\mathcal{O}_i,\mathcal{O}_k;\underline{\boldsymbol{\vartheta}},\underline{\boldsymbol{\lambda}}^{\mathrm{mr}}_C)\middle|\mathcal{O}_i\right\}\right] \\ &= \mathbb{E}\left\{2^{-1}\nabla_{\boldsymbol{\vartheta}}\boldsymbol{\varphi}^{\mathrm{eff}}_C(\mathcal{O}_i;\underline{\boldsymbol{\vartheta}},\underline{\boldsymbol{\lambda}}^{\mathrm{mr}}_C)\right\},\end{aligned}$$

which is equal to zero if the parametric working model correctly specifies the nuisance function, i.e., $\zeta_a(\underline{\boldsymbol{\vartheta}}_a) = \zeta^0_a$, because of the Neyman orthogonality of the EIF. Therefore, if the parametric working model correctly specifies the nuisance functions, $\underline{\boldsymbol{\lambda}}^{\mathrm{mr}}_C = \boldsymbol{\lambda}^0_C$, and

$$\boldsymbol{\varphi}^{\mathrm{mr}}_C(\mathcal{O}_i;\underline{\boldsymbol{\vartheta}},\boldsymbol{\lambda}^0_C) = -2\left(\underline{\boldsymbol{B}}^{\mathrm{mr}}_{C,\boldsymbol{\lambda\lambda}}\right)^{-1}\mathbb{E}\left\{\boldsymbol{\psi}^{\mathrm{eff}}_{C,\boldsymbol{\lambda}}(\mathcal{O}_i,\mathcal{O}_k;\underline{\boldsymbol{\vartheta}},\boldsymbol{\lambda}^0_C)\middle|\mathcal{O}_i\right\} = \boldsymbol{\varphi}^{\mathrm{eff}}_C(\mathcal{O}_i;\underline{\boldsymbol{\vartheta}},\boldsymbol{\lambda}^0_C),$$

because $\underline{\boldsymbol{B}}_{C,\boldsymbol{\lambda\lambda}}^{\mathrm{mr}} = -\boldsymbol{I}_2$, which proves the semiparametric efficient lower bound. The algebra is omitted.

Results for $\widehat{\boldsymbol{\lambda}}_I^{\mathrm{mr}}$, $\widehat{\Lambda}_I^{\mathrm{mr}}$, and their variance estimators, $\widehat{\boldsymbol{V}}_I^{\mathrm{mr}}$ and $\widehat{V}_I^{\mathrm{mr}}$, can be obtained following the same procedure. Here, we check the semiparametric efficiency lower bound. When the parametric working model correctly specifies the nuisance functions, $\underline{\boldsymbol{B}}_{I,\boldsymbol{\lambda\vartheta}}^{\mathrm{mr}} = \mathbb{E}\{\nabla_{\boldsymbol{\vartheta}}\boldsymbol{\psi}_{I,\boldsymbol{\lambda}}^{\mathrm{eff}}(\mathcal{O}_i, \mathcal{O}_k; \underline{\boldsymbol{\vartheta}}, \boldsymbol{\lambda}_I^0)\} = \mathbb{E}[\nabla_{\boldsymbol{\vartheta}}\mathbb{E}\{\boldsymbol{\psi}_{I,\boldsymbol{\lambda}}^{\mathrm{eff}}(\mathcal{O}_i, \mathcal{O}_k; \underline{\boldsymbol{\vartheta}}, \boldsymbol{\lambda}_I^0)|\mathcal{O}_i\}] = \mathbb{E}\{2^{-1}\nabla_{\boldsymbol{\vartheta}}\boldsymbol{\varphi}_I^{\text{eff-num}}(\mathcal{O}_i; \underline{\boldsymbol{\vartheta}}, \boldsymbol{\lambda}_I^0)\} = \mathbf{0}$ because of the Neyman orthogonality of the EIF. Therefore,

$$\boldsymbol{\varphi}_I^{\mathrm{mr}}(\mathcal{O}_i; \underline{\boldsymbol{\vartheta}}, \boldsymbol{\lambda}_I^0) = -2\left(\underline{\boldsymbol{B}}_{I,\boldsymbol{\lambda\lambda}}^{\mathrm{mr}}\right)^{-1}\mathbb{E}\left\{\boldsymbol{\psi}_{I,\boldsymbol{\lambda}}^{\mathrm{eff}}(\mathcal{O}_i, \mathcal{O}_k; \underline{\boldsymbol{\vartheta}}, \boldsymbol{\lambda}_I^0)\Big|\mathcal{O}_i\right\} = \boldsymbol{\varphi}_I^{\mathrm{eff}}(\mathcal{O}_i; \underline{\boldsymbol{\vartheta}}, \boldsymbol{\lambda}_I^0),$$

since $\underline{\boldsymbol{B}}_{I,\boldsymbol{\lambda\lambda}}^{\mathrm{mr}} = \mathbb{E}\{\nabla_{\boldsymbol{\lambda}}\boldsymbol{\psi}_{I,\boldsymbol{\lambda}}^{\mathrm{eff}}(\mathcal{O}_i, \mathcal{O}_k; \underline{\boldsymbol{\vartheta}}, \boldsymbol{\lambda}_I^0)\} = -\mathbb{E}(N_iN_k) \times \boldsymbol{I}_2$. □

# S5 The Debiased machine learning estimators

We first recap the sample-splitting scheme. The sample (single) index set $\mathcal{M} = \{1, \ldots, m\}$ is first divided into $|\mathfrak{I}^{\mathrm{si}}|$ subsets of similar sizes, forming a partition $\mathfrak{I}^{\mathrm{si}} = \{\mathcal{I}_1^{\mathrm{si}}, \ldots, \mathcal{I}_{|\mathfrak{I}^{\mathrm{si}}|}^{\mathrm{si}}\}$. Then, upon $\mathfrak{I}^{\mathrm{si}}$, a second partition, $\mathfrak{I}^{\mathrm{pr}}$, can be formed for all pairs $(i, k)$ with $1 \le i < k \le m$, which has $|\mathfrak{I}^{\mathrm{pr}}| = |\mathfrak{I}^{\mathrm{si}}|(|\mathfrak{I}^{\mathrm{si}}| + 1)/2$ elements, i.e., $\mathfrak{I}^{\mathrm{pr}} = \{\mathcal{I}_1^{\mathrm{pr}}, \ldots, \mathcal{I}_{|\mathfrak{I}^{\mathrm{pr}}|}^{\mathrm{pr}}\}$. For $v = C, I$, the following estimating equations are for $\widehat{\boldsymbol{\lambda}}_v^{\mathrm{dml}}$:

$$\sum_{p=1}^{|\mathfrak{I}^{\mathrm{pr}}|}\sum_{(i,k)\in\mathcal{I}_p^{\mathrm{pr}}}\boldsymbol{\psi}_v^{\mathrm{eff}}(\mathcal{O}_i, \mathcal{O}_k; \widehat{\zeta}_p, \boldsymbol{\lambda}) = \sum_{p=1}^{|\mathfrak{I}^{\mathrm{pr}}|}\sum_{(i,k)\in\mathcal{I}_p^{\mathrm{pr}}}\left\{\begin{array}{c}\psi_{v,1}^{\mathrm{eff}}(\mathcal{O}_i, \mathcal{O}_k; \widehat{\zeta}_p, \lambda_1)\\ \psi_{v,0}^{\mathrm{eff}}(\mathcal{O}_i, \mathcal{O}_k; \widehat{\zeta}_p, \lambda_0)\end{array}\right\} = \mathbf{0}$$

For a given partition $\mathfrak{I}^{\mathrm{pr}}$, we form intermediate estimating equations using observations in each $\mathcal{I}_p^{\mathrm{pr}}$ with $\widehat{\zeta}_p$ estimated using observations in $(\mathcal{I}_p^{\mathrm{pr}})^c$, which excludes pairs involving clusters in $\mathcal{I}_p^{\mathrm{pr}}$.

We state the following regularity conditions required to establish the consistency.

(C1) $\boldsymbol{\lambda} \in \boldsymbol{\Theta}_{\boldsymbol{\lambda}}$, a compact subset of the Euclidean space.

(C2) There exists a unique solution, $\boldsymbol{\lambda}_v^0$, in the interior of $\boldsymbol{\Theta}_{\boldsymbol{\lambda}}$ to the equations $\mathbb{E}\{\boldsymbol{\psi}_v^{\mathrm{eff}}(\mathcal{O}_1, \mathcal{O}_2; \zeta^0, \boldsymbol{\lambda})\} = \mathbf{0}$.

(C3) $\|\widehat{\zeta}_p - \zeta^0\| = o_{\mathbb{P}}(1)$, for $p = 1, \ldots, |\mathfrak{I}^{\mathrm{pr}}|$.

(C4) There exists a square-integrable function $e(\mathcal{O}_i, \mathcal{O}_k)$ such that

$$\left\|\boldsymbol{\psi}_v^{\mathrm{eff}}(\mathcal{O}_i, \mathcal{O}_k; \zeta, \boldsymbol{\lambda}) - \boldsymbol{\psi}_v^{\mathrm{eff}}(\mathcal{O}_i, \mathcal{O}_k; \widetilde{\zeta}, \widetilde{\boldsymbol{\lambda}})\right\| \le e(\mathcal{O}_i, \mathcal{O}_k)\left(\left\|\zeta - \widetilde{\zeta}\right\| + \left\|\boldsymbol{\lambda} - \widetilde{\boldsymbol{\lambda}}\right\|\right).$$

(C5) For all $\boldsymbol{\lambda} \in \boldsymbol{\Theta}_{\boldsymbol{\lambda}}$ and $p = 1, \ldots, |\mathfrak{I}^{\mathrm{pr}}|$,

$$\binom{m}{2}^{-1}\sum_{p=1}^{|\mathfrak{I}^{\mathrm{pr}}|}\sum_{(i,k)\in\mathcal{I}_p^{\mathrm{pr}}}\boldsymbol{\psi}_v^{\mathrm{eff}}(\mathcal{O}_i, \mathcal{O}_k; \widehat{\zeta}_p, \boldsymbol{\lambda}) \xrightarrow{p} \mathbb{E}\left\{\boldsymbol{\psi}_v^{\mathrm{eff}}(\mathcal{O}_i, \mathcal{O}_k; \zeta^0, \boldsymbol{\lambda})\right\}.$$

The following additional regularity conditions are required to establish the asymptotic normality.

(A1) $\|\widehat{\zeta}_p - \zeta^0\| = o_{\mathbb{P}}(m^{-1/4})$, for $p = 1, \ldots, |\mathfrak{I}^{\mathrm{pr}}|$.

(A2) The function $\boldsymbol{\psi}_v^{\mathrm{eff}}(\mathcal{O}_i, \mathcal{O}_k; \zeta, \boldsymbol{\lambda})$ is twice continuously differentiable in $\boldsymbol{\lambda}$ in a neighborhood of $\boldsymbol{\lambda}_v^0$, and once continuously differentiable in $\zeta$, for all $\mathcal{O}_i$ and $\mathcal{O}_k$.

(A3) $\boldsymbol{B}_{v,\boldsymbol{\lambda}}^{\text{eff},0} = \mathbb{E}\{\nabla_{\boldsymbol{\lambda}} \boldsymbol{\psi}_v^{\text{eff}}(\mathcal{O}_i, \mathcal{O}_k; \zeta^0, \boldsymbol{\lambda}_v^0)\}$ exists and is non-singular.

(A4) $\mathbb{E}\{\|\boldsymbol{\psi}_v^{\text{eff}}(\mathcal{O}_i, \mathcal{O}_k; \zeta^0, \boldsymbol{\lambda}_v^0)\|^2\} < \infty$.

(A5) There exists a square-integrable function $\dot{e}(\mathcal{O}_i, \mathcal{O}_k)$ such that

$$\left\|\nabla_{\boldsymbol{\lambda}} \boldsymbol{\psi}_v^{\text{eff}}(\mathcal{O}_i, \mathcal{O}_k; \zeta, \boldsymbol{\lambda}) - \nabla_{\boldsymbol{\lambda}} \boldsymbol{\psi}_v^{\text{eff}}(\mathcal{O}_i, \mathcal{O}_k; \widetilde{\zeta}, \widetilde{\boldsymbol{\lambda}})\right\| \le \dot{e}(\mathcal{O}_i, \mathcal{O}_k) \left(\left\|\zeta - \widetilde{\zeta}\right\| + \left\|\boldsymbol{\lambda} - \widetilde{\boldsymbol{\lambda}}\right\|\right).$$

The following additional regularity condition is required for the consistency of the variance estimator.

(V1) $\mathbb{E}\{\|\boldsymbol{\psi}_v^{\text{eff}}(\mathcal{O}_i, \mathcal{O}_k; \zeta^0, \boldsymbol{\lambda}_v^0)\|^4\} < \infty$.

*Proof of Theorem 4.* We first prove the consistency, which starts with proving

$$\sup_{\boldsymbol{\lambda} \in \boldsymbol{\Theta}_{\boldsymbol{\lambda}}} \left\| \binom{m}{2}^{-1} \sum_{p=1}^{|\mathfrak{I}^{\text{pr}}|} \sum_{(i,k) \in \mathcal{I}_p^{\text{pr}}} \boldsymbol{\psi}_v^{\text{eff}}(\mathcal{O}_i, \mathcal{O}_k; \widehat{\zeta}_p, \boldsymbol{\lambda}) - \mathbb{E}\left\{\boldsymbol{\psi}_v^{\text{eff}}(\mathcal{O}_i, \mathcal{O}_k; \zeta^0, \boldsymbol{\lambda})\right\} \right\| = o_{\mathbb{P}}(1) \tag{S9}$$

We decompose the difference on the left-hand side of (S9) as

$$\begin{aligned}
&\left\| \binom{m}{2}^{-1} \sum_{p=1}^{|\mathfrak{I}^{\text{pr}}|} \sum_{(i,k) \in \mathcal{I}_p^{\text{pr}}} \boldsymbol{\psi}_v^{\text{eff}}(\mathcal{O}_i, \mathcal{O}_k; \widehat{\zeta}_p, \boldsymbol{\lambda}) - \mathbb{E}\left\{\boldsymbol{\psi}_v^{\text{eff}}(\mathcal{O}_i, \mathcal{O}_k; \zeta^0, \boldsymbol{\lambda})\right\} \right\| \\
\le &\left\| \binom{m}{2}^{-1} \sum_{p=1}^{|\mathfrak{I}^{\text{pr}}|} \sum_{(i,k) \in \mathcal{I}_p^{\text{pr}}} \boldsymbol{\psi}_v^{\text{eff}}(\mathcal{O}_i, \mathcal{O}_k; \widehat{\zeta}_p, \boldsymbol{\lambda}) - \binom{m}{2}^{-1} \sum_{1 \le i < k \le m} \boldsymbol{\psi}_v^{\text{eff}}(\mathcal{O}_i, \mathcal{O}_k; \zeta^0, \boldsymbol{\lambda}) \right\| &\text{(S10)} \\
&+ \left\| \binom{m}{2}^{-1} \sum_{1 \le i < k \le m} \boldsymbol{\psi}_v^{\text{eff}}(\mathcal{O}_i, \mathcal{O}_k; \zeta^0, \boldsymbol{\lambda}) - \mathbb{E}\left\{\boldsymbol{\psi}_v^{\text{eff}}(\mathcal{O}_i, \mathcal{O}_k; \zeta^0, \boldsymbol{\lambda})\right\} \right\|, &\text{(S11)}
\end{aligned}$$

where (S10) is

$$\begin{aligned}
&\left\| \binom{m}{2}^{-1} \sum_{p=1}^{|\mathfrak{I}^{\text{pr}}|} \sum_{(i,k) \in \mathcal{I}_p^{\text{pr}}} \boldsymbol{\psi}_v^{\text{eff}}(\mathcal{O}_i, \mathcal{O}_k; \widehat{\zeta}_p, \boldsymbol{\lambda}) - \binom{m}{2}^{-1} \sum_{p=1}^{|\mathfrak{I}^{\text{pr}}|} \sum_{(i,k) \in \mathcal{I}_p^{\text{pr}}} \boldsymbol{\psi}_v^{\text{eff}}(\mathcal{O}_i, \mathcal{O}_k; \zeta^0, \boldsymbol{\lambda}) \right\| \\
\le &\binom{m}{2}^{-1} \sum_{p=1}^{|\mathfrak{I}^{\text{pr}}|} \sum_{(i,k) \in \mathcal{I}_p^{\text{pr}}} e(\mathcal{O}_i, \mathcal{O}_k) \left\| \widehat{\zeta}_p - \zeta^0 \right\|,
\end{aligned}$$

by the regularity condition (C4). By regularity condition (C3) and the law of large numbers for U-statistics:

$$\binom{m}{2}^{-1} \sum_{p=1}^{|\mathfrak{I}^{\text{pr}}|} \sum_{(i,k) \in \mathcal{I}_p^{\text{pr}}} e(\mathcal{O}_i, \mathcal{O}_k) = O_{\mathbb{P}}(1).$$

Thus,

$$\sup_{\boldsymbol{\lambda} \in \boldsymbol{\Theta}_{\boldsymbol{\lambda}}} \left\| \binom{m}{2}^{-1} \sum_{p=1}^{|\mathfrak{I}^{\text{pr}}|} \sum_{(i,k) \in \mathcal{I}_p^{\text{pr}}} \boldsymbol{\psi}_v^{\text{eff}}(\mathcal{O}_i, \mathcal{O}_k; \widehat{\zeta}_p, \boldsymbol{\lambda}) - \binom{m}{2}^{-1} \sum_{1 \le i < k \le m} \boldsymbol{\psi}_v^{\text{eff}}(\mathcal{O}_i, \mathcal{O}_k; \zeta^0, \boldsymbol{\lambda}) \right\| = o_{\mathbb{P}}(1).$$

For (S11), by regularity condition (C1), for any $\delta > 0$, there exists a finite cover $\{\boldsymbol{\lambda}^1, \ldots, \boldsymbol{\lambda}^{N_\delta}\}$ such that for any $\boldsymbol{\lambda}$, there exists $\jmath = 1, \ldots, N_\delta$ with $\|\boldsymbol{\lambda} - \boldsymbol{\lambda}^\jmath\| < \delta$. Then,

$$\begin{aligned}
&\sup_{\boldsymbol{\lambda}\in\boldsymbol{\Theta}_{\boldsymbol{\lambda}}} \left\| \binom{m}{2}^{-1} \sum_{1\le i<k\le m} \boldsymbol{\psi}_v^{\text{eff}}(\mathcal{O}_i, \mathcal{O}_k; \zeta^0, \boldsymbol{\lambda}) - \mathbb{E}\left\{\boldsymbol{\psi}_v^{\text{eff}}(\mathcal{O}_i, \mathcal{O}_k; \zeta^0, \boldsymbol{\lambda})\right\} \right\| \\
&\le \max_{1\le\jmath\le N_\delta} \left\| \binom{m}{2}^{-1} \sum_{1\le i<k\le m} \boldsymbol{\psi}_v^{\text{eff}}(\mathcal{O}_i, \mathcal{O}_k; \zeta^0, \boldsymbol{\lambda}^\jmath) - \mathbb{E}\left\{\boldsymbol{\psi}_v^{\text{eff}}(\mathcal{O}_i, \mathcal{O}_k; \zeta^0, \boldsymbol{\lambda}^\jmath)\right\} \right\| + \mathcal{R}_{v,m},
\end{aligned}$$

where, by regularity condition (C4),

$$\mathcal{R}_{v,m} \le \delta \binom{m}{2}^{-1} \sum_{1\le i<k\le m} e(\mathcal{O}_i, \mathcal{O}_k).$$

By regularity condition (C5),

$$\max_{1\le\jmath\le N_\delta} \left\| \binom{m}{2}^{-1} \sum_{1\le i<k\le m} \boldsymbol{\psi}_v^{\text{eff}}(\mathcal{O}_i, \mathcal{O}_k; \zeta^0, \boldsymbol{\lambda}^\jmath) - \mathbb{E}\left\{\boldsymbol{\psi}_v^{\text{eff}}(\mathcal{O}_i, \mathcal{O}_k; \zeta^0, \boldsymbol{\lambda}^\jmath)\right\} \right\| = o_{\mathbb{P}}(1),$$

and by choosing a small $\delta$, $\mathcal{R}_m$ can be made arbitrarily small. Thus,

$$\sup_{\boldsymbol{\lambda}\in\boldsymbol{\Theta}_{\boldsymbol{\lambda}}} \left\| \binom{m}{2}^{-1} \sum_{1\le i<k\le m} \boldsymbol{\psi}_v^{\text{eff}}(\mathcal{O}_i, \mathcal{O}_k; \zeta^0, \boldsymbol{\lambda}) - \mathbb{E}\left\{\boldsymbol{\psi}_v^{\text{eff}}(\mathcal{O}_i, \mathcal{O}_k; \zeta^0, \boldsymbol{\lambda})\right\} \right\| = o_{\mathbb{P}}(1).$$

Therefore, (S9) is proved. By definition,

$$\binom{m}{2}^{-1} \sum_{p=1}^{|\mathfrak{I}^{\text{pr}}|} \sum_{(i,k)\in\mathcal{I}_p^{\text{pr}}} \boldsymbol{\psi}_v^{\text{eff}}(\mathcal{O}_i, \mathcal{O}_k; \widehat{\zeta}_p, \widehat{\boldsymbol{\lambda}}_v^{\text{dml}}) = \mathbf{0}.$$

From (S9), we have

$$\begin{aligned}
&\left\| \mathbb{E}\left\{\boldsymbol{\psi}_v^{\text{eff}}(\mathcal{O}_i, \mathcal{O}_k; \zeta^0, \widehat{\boldsymbol{\lambda}}_v^{\text{dml}})\right\} \right\| \\
&= \left\| \mathbb{E}\left\{\boldsymbol{\psi}_v^{\text{eff}}(\mathcal{O}_i, \mathcal{O}_k; \zeta^0, \widehat{\boldsymbol{\lambda}}_v^{\text{dml}})\right\} - \binom{m}{2}^{-1} \sum_{p=1}^{|\mathfrak{I}^{\text{pr}}|} \sum_{(i,k)\in\mathcal{I}_p^{\text{pr}}} \boldsymbol{\psi}_v^{\text{eff}}(\mathcal{O}_i, \mathcal{O}_k; \widehat{\zeta}_p, \widehat{\boldsymbol{\lambda}}_v^{\text{dml}}) \right\| \\
&\le \sup_{\boldsymbol{\lambda}\in\boldsymbol{\Theta}_{\boldsymbol{\lambda}}} \left\| \binom{m}{2}^{-1} \sum_{p=1}^{|\mathfrak{I}^{\text{pr}}|} \sum_{(i,k)\in\mathcal{I}_p^{\text{pr}}} \boldsymbol{\psi}_v^{\text{eff}}(\mathcal{O}_i, \mathcal{O}_k; \widehat{\zeta}_p, \boldsymbol{\lambda}) - \mathbb{E}\left\{\boldsymbol{\psi}_v^{\text{eff}}(\mathcal{O}_i, \mathcal{O}_k; \zeta^0, \boldsymbol{\lambda})\right\} \right\| \\
&= o_{\mathbb{P}}(1).
\end{aligned}$$

Suppose $\widehat{\boldsymbol{\lambda}}_v^{\text{dml}}$ is not consistent. Then, there exists $\epsilon > 0$ such that $\limsup_{m\to\infty} \mathbb{P}(\|\widehat{\boldsymbol{\lambda}}_v^{\text{dml}} - \boldsymbol{\lambda}_v^0\| \ge \epsilon) > 0$. Define the set $\mathfrak{B}_\epsilon = \{\boldsymbol{\lambda} \in \boldsymbol{\Theta}_{\boldsymbol{\lambda}} : \|\boldsymbol{\lambda} - \boldsymbol{\lambda}_v^0\| \ge \epsilon\}$. By regularity condition (C1), $\mathfrak{B}_\epsilon$ is compact. By regularity condition (C2), we have

$c_\epsilon = \inf_{\boldsymbol{\lambda} \in \mathfrak{B}_\epsilon} \|\mathbb{E}\{\boldsymbol{\psi}_v^{\mathrm{eff}}(\mathcal{O}_i, \mathcal{O}_k; \zeta^0, \boldsymbol{\lambda})\}\| > 0$. However, then,

$$\mathbb{P}\left(\left\|\mathbb{E}\left\{\boldsymbol{\psi}_v^{\mathrm{eff}}(\mathcal{O}_i, \mathcal{O}_k; \zeta^0, \widehat{\boldsymbol{\lambda}}_v^{\mathrm{dml}})\right\}\right\| \geq c_\epsilon\right) \geq \mathbb{P}\left(\left\|\widehat{\boldsymbol{\lambda}}_v^{\mathrm{dml}} - \boldsymbol{\lambda}_v^0\right\| \geq \epsilon\right) > 0,$$

for infinitely many $m$, which contradicts $\|\mathbb{E}\{\boldsymbol{\psi}_v^{\mathrm{eff}}(\mathcal{O}_i, \mathcal{O}_k; \zeta^0, \widehat{\boldsymbol{\lambda}}_v^{\mathrm{dml}})\}\| = o_{\mathbb{P}}(1)$. Therefore, $\widehat{\boldsymbol{\lambda}}_v^{\mathrm{dml}} \xrightarrow{p} \boldsymbol{\lambda}_v^0$.

We then prove the asymptotic normality. By the mean value theorem,

$$\begin{aligned}
\mathbf{0} &= m^{1/2}\binom{m}{2}^{-1}\sum_{p=1}^{|\mathfrak{I}^{\mathrm{pr}}|}\sum_{(i,k)\in\mathcal{I}_p^{\mathrm{pr}}} \boldsymbol{\psi}_v^{\mathrm{eff}}(\mathcal{O}_i, \mathcal{O}_k; \widehat{\zeta}_p, \widehat{\boldsymbol{\lambda}}_v^{\mathrm{dml}}) \\
&= m^{1/2}\binom{m}{2}^{-1}\sum_{p=1}^{|\mathfrak{I}^{\mathrm{pr}}|}\sum_{(i,k)\in\mathcal{I}_p^{\mathrm{pr}}} \boldsymbol{\psi}_v^{\mathrm{eff}}(\mathcal{O}_i, \mathcal{O}_k; \widehat{\zeta}_p, \boldsymbol{\lambda}_v^0) \\
&\quad + \binom{m}{2}^{-1}\sum_{p=1}^{|\mathfrak{I}^{\mathrm{pr}}|}\sum_{(i,k)\in\mathcal{I}_p^{\mathrm{pr}}} \nabla_{\boldsymbol{\lambda}}\boldsymbol{\psi}_v^{\mathrm{eff}}(\mathcal{O}_i, \mathcal{O}_k; \widehat{\zeta}_p, \widetilde{\boldsymbol{\lambda}}_v) m^{1/2}(\widehat{\boldsymbol{\lambda}}_v^{\mathrm{dml}} - \boldsymbol{\lambda}_v^0),
\end{aligned}$$

where $\widetilde{\boldsymbol{\lambda}}_v$ lies on the segment between $\widehat{\boldsymbol{\lambda}}_v^{\mathrm{dml}}$ and $\boldsymbol{\lambda}_v^0$. By rearranging, we have

$$\begin{aligned}
m^{1/2}(\widehat{\boldsymbol{\lambda}}_v^{\mathrm{dml}} - \boldsymbol{\lambda}_v^0) &= -\left\{\binom{m}{2}^{-1}\sum_{p=1}^{|\mathfrak{I}^{\mathrm{pr}}|}\sum_{(i,k)\in\mathcal{I}_p^{\mathrm{pr}}} \nabla_{\boldsymbol{\lambda}}\boldsymbol{\psi}_v^{\mathrm{eff}}(\mathcal{O}_i, \mathcal{O}_k; \widehat{\zeta}_p, \widetilde{\boldsymbol{\lambda}}_v)\right\}^{-1} \\
&\qquad \times m^{1/2}\binom{m}{2}^{-1}\sum_{p=1}^{|\mathfrak{I}^{\mathrm{pr}}|}\sum_{(i,k)\in\mathcal{I}_p^{\mathrm{pr}}} \boldsymbol{\psi}_v^{\mathrm{eff}}(\mathcal{O}_i, \mathcal{O}_k; \widehat{\zeta}_p, \boldsymbol{\lambda}_v^0).
\end{aligned}$$

We then show that

$$\binom{m}{2}^{-1}\sum_{p=1}^{|\mathfrak{I}^{\mathrm{pr}}|}\sum_{(i,k)\in\mathcal{I}_p^{\mathrm{pr}}} \nabla_{\boldsymbol{\lambda}}\boldsymbol{\psi}_v^{\mathrm{eff}}(\mathcal{O}_i, \mathcal{O}_k; \widehat{\zeta}_p, \widetilde{\boldsymbol{\lambda}}_v) \xrightarrow{p} \boldsymbol{B}_{v,\boldsymbol{\lambda}}^{\mathrm{eff},0}. \tag{S12}$$

Specifically,

$$\begin{aligned}
&\left\|\binom{m}{2}^{-1}\sum_{p=1}^{|\mathfrak{I}^{\mathrm{pr}}|}\sum_{(i,k)\in\mathcal{I}_p^{\mathrm{pr}}} \nabla_{\boldsymbol{\lambda}}\boldsymbol{\psi}_v^{\mathrm{eff}}(\mathcal{O}_i, \mathcal{O}_k; \widehat{\zeta}_p, \widetilde{\boldsymbol{\lambda}}_v) - \boldsymbol{B}_{v,\boldsymbol{\lambda}}^{\mathrm{eff},0}\right\| \\
\leq &\left\|\binom{m}{2}^{-1}\sum_{p=1}^{|\mathfrak{I}^{\mathrm{pr}}|}\sum_{(i,k)\in\mathcal{I}_p^{\mathrm{pr}}} \nabla_{\boldsymbol{\lambda}}\boldsymbol{\psi}_v^{\mathrm{eff}}(\mathcal{O}_i, \mathcal{O}_k; \widehat{\zeta}_p, \widetilde{\boldsymbol{\lambda}}_v) - \binom{m}{2}^{-1}\sum_{1\leq i<k\leq m} \nabla_{\boldsymbol{\lambda}}\boldsymbol{\psi}_v^{\mathrm{eff}}(\mathcal{O}_i, \mathcal{O}_k; \zeta^0, \boldsymbol{\lambda}_v^0)\right\| \\
&\quad + \left\|\binom{m}{2}^{-1}\sum_{1\leq i<k\leq m} \nabla_{\boldsymbol{\lambda}}\boldsymbol{\psi}_v^{\mathrm{eff}}(\mathcal{O}_i, \mathcal{O}_k; \zeta^0, \boldsymbol{\lambda}_v^0) - \boldsymbol{B}_{v,\boldsymbol{\lambda}}^{\mathrm{eff},0}\right\|.
\end{aligned}$$

By the law of large numbers for U-statistics and regularity condition (A3),

$$\binom{m}{2}^{-1}\sum_{1\leq i<k\leq m} \nabla_{\boldsymbol{\lambda}}\boldsymbol{\psi}_v^{\mathrm{eff}}(\mathcal{O}_i, \mathcal{O}_k; \zeta^0, \boldsymbol{\lambda}_v^0) \xrightarrow{p} \boldsymbol{B}_{v,\lambda}^{\mathrm{eff},0}.$$

By regularity condition (A5) and the consistency ($\widetilde{\boldsymbol{\lambda}}_v \xrightarrow{p} \boldsymbol{\lambda}_v^0$ and $\widehat{\zeta}_p \xrightarrow{p} \zeta^0$),

$$\left\| \binom{m}{2}^{-1} \sum_{p=1}^{|\mathfrak{I}^{\mathrm{pr}}|} \sum_{(i,k)\in\mathcal{I}_p^{\mathrm{pr}}} \nabla_{\boldsymbol{\lambda}} \boldsymbol{\psi}_v^{\mathrm{eff}}(\mathcal{O}_i, \mathcal{O}_k; \widehat{\zeta}_p, \widetilde{\boldsymbol{\lambda}}_v) - \binom{m}{2}^{-1} \sum_{1\le i<k\le m} \nabla_{\boldsymbol{\lambda}} \boldsymbol{\psi}_v^{\mathrm{eff}}(\mathcal{O}_i, \mathcal{O}_k; \zeta^0, \boldsymbol{\lambda}_v^0) \right\|$$
$$\le \binom{m}{2}^{-1} \sum_{p=1}^{|\mathfrak{I}^{\mathrm{pr}}|} \sum_{(i,k)\in\mathcal{I}_p^{\mathrm{pr}}} \dot{e}(\mathcal{O}_i, \mathcal{O}_k) \left( \left\| \widetilde{\boldsymbol{\lambda}}_v - \boldsymbol{\lambda}_v^0 \right\| + \left\| \widehat{\zeta}_p - \zeta^0 \right\| \right) = o_{\mathbb{P}}(1).$$

Thus, (S12) is proved by Slutsky's theorem. Then,

$$m^{1/2} \binom{m}{2}^{-1} \sum_{p=1}^{|\mathfrak{I}^{\mathrm{pr}}|} \sum_{(i,k)\in\mathcal{I}_p^{\mathrm{pr}}} \boldsymbol{\psi}_v^{\mathrm{eff}}(\mathcal{O}_i, \mathcal{O}_k; \widehat{\zeta}_p, \boldsymbol{\lambda}_v^0)$$
$$= m^{1/2} \binom{m}{2}^{-1} \sum_{1\le i<k\le m} \boldsymbol{\psi}_v^{\mathrm{eff}}(\mathcal{O}_i, \mathcal{O}_k; \zeta^0, \boldsymbol{\lambda}_v^0)$$
$$+ m^{1/2} \left\{ \binom{m}{2}^{-1} \sum_{p=1}^{|\mathfrak{I}^{\mathrm{pr}}|} \sum_{(i,k)\in\mathcal{I}_p^{\mathrm{pr}}} \boldsymbol{\psi}_v^{\mathrm{eff}}(\mathcal{O}_i, \mathcal{O}_k; \widehat{\zeta}_p, \boldsymbol{\lambda}_v^0) - \binom{m}{2}^{-1} \sum_{1\le i<k\le m} \boldsymbol{\psi}_v^{\mathrm{eff}}(\mathcal{O}_i, \mathcal{O}_k; \zeta^0, \boldsymbol{\lambda}_v^0) \right\},$$

For the first term, by the central limit theorem for U-statistics (van der Vaart, 1998, Theorem 12.3), we have

$$m^{1/2} \binom{m}{2}^{-1} \sum_{1\le i<k\le m} \boldsymbol{\psi}_v^{\mathrm{eff}}(\mathcal{O}_i, \mathcal{O}_k; \zeta^0, \boldsymbol{\lambda}_v^0) \xrightarrow{d} \mathcal{N}(0, \boldsymbol{\Sigma}_v^{\mathrm{eff},0}),$$

where $\boldsymbol{\Sigma}_v^{\mathrm{eff},0} = 4\mathbb{V}\mathrm{ar}\{\overline{\boldsymbol{\psi}}_v^{\mathrm{eff}}(\mathcal{O}_i; \zeta^0, \boldsymbol{\lambda}_v^0)\}$. For the second term, a Taylor expansion in $\zeta$ around $\zeta^0$ gives us

$$m^{1/2} \left\{ \binom{m}{2}^{-1} \sum_{p=1}^{|\mathfrak{I}^{\mathrm{pr}}|} \sum_{(i,k)\in\mathcal{I}_p^{\mathrm{pr}}} \boldsymbol{\psi}_v^{\mathrm{eff}}(\mathcal{O}_i, \mathcal{O}_k; \widehat{\zeta}_p, \boldsymbol{\lambda}_v^0) - \binom{m}{2}^{-1} \sum_{1\le i<k\le m} \boldsymbol{\psi}_v^{\mathrm{eff}}(\mathcal{O}_i, \mathcal{O}_k; \zeta^0, \boldsymbol{\lambda}_v^0) \right\}$$
$$= \binom{m}{2}^{-1} \sum_{p=1}^{|\mathfrak{I}^{\mathrm{pr}}|} \sum_{(i,k)\in\mathcal{I}_p^{\mathrm{pr}}} \nabla_{\zeta} \boldsymbol{\psi}_v^{\mathrm{eff}}(\mathcal{O}_i, \mathcal{O}_k; \widetilde{\zeta}_p, \boldsymbol{\lambda}_v^0) m^{1/2}(\widehat{\zeta}_p - \zeta^0) + \text{remainder}.$$

Some algebra can verify that $\mathbb{E}\{\nabla_{\zeta} \boldsymbol{\psi}_v^{\mathrm{eff}}(\mathcal{O}_i, \mathcal{O}_k; \zeta^0, \boldsymbol{\lambda}^0)\} = \mathbf{0}$. Thus, by the law of large numbers,

$$\binom{m}{2}^{-1} \sum_{p=1}^{|\mathfrak{I}^{\mathrm{pr}}|} \sum_{(i,k)\in\mathcal{I}_p^{\mathrm{pr}}} \nabla_{\zeta} \boldsymbol{\psi}_v^{\mathrm{eff}}(\mathcal{O}_i, \mathcal{O}_k; \widetilde{\zeta}_p, \boldsymbol{\lambda}_v^0) = \boldsymbol{o}_{\mathbb{P}}(1).$$

The remainder term is $m^{1/2}\boldsymbol{O}_{\mathbb{P}}(\|\widehat{\zeta}_p - \zeta^0\|^2)$. Therefore, the second term is

$$m^{1/2}\boldsymbol{O}_{\mathbb{P}}(\|\widehat{\zeta}_p - \zeta^0\|^2) = m^{1/2}\boldsymbol{o}_{\mathbb{P}}(m^{-1/2}) = \boldsymbol{o}_{\mathbb{P}}(1)$$

by regularity condition (A1). Putting everything together, we have

$$m^{1/2}(\widehat{\boldsymbol{\lambda}}_v^{\mathrm{dml}} - \boldsymbol{\lambda}_v^0) = -\left(\boldsymbol{B}_{v,\boldsymbol{\lambda}}^{\mathrm{eff},0}\right)^{-1} m^{1/2}\binom{m}{2}^{-1} \sum_{1\le i<k\le m} \nabla_{\boldsymbol{\lambda}}\boldsymbol{\psi}_v^{\mathrm{eff}}(\mathcal{O}_i,\mathcal{O}_k;\zeta^0,\boldsymbol{\lambda}_v^0) + \boldsymbol{o}_{\mathbb{P}}(1).$$

Therefore,

$$m^{1/2}(\widehat{\boldsymbol{\lambda}}_v^{\mathrm{dml}} - \boldsymbol{\lambda}_v^0) \xrightarrow{d} \mathcal{N}(\mathbf{0}, \boldsymbol{V}_v^{\mathrm{eff},0}),$$

where $\boldsymbol{V}_v^{\mathrm{eff},0} = (\boldsymbol{B}_{v,\boldsymbol{\lambda}}^{\mathrm{eff},0})^{-1}\boldsymbol{\Sigma}_v^{\mathrm{eff},0}\{(\boldsymbol{B}_{v,\boldsymbol{\lambda}}^{\mathrm{eff},0})^{-1}\}^\top$. The asymptotic normality has been proved. The influence function of $\widehat{\boldsymbol{\lambda}}_v^{\mathrm{dml}}$ is

$$\boldsymbol{\varphi}_v^{\mathrm{dml}}(\mathcal{O}_i;\zeta,\boldsymbol{\lambda}) = -2\left(\boldsymbol{B}_{v,\boldsymbol{\lambda}}^{\mathrm{eff}}\right)^{-1}\mathbb{E}\left\{\boldsymbol{\psi}_v^{\mathrm{eff}}(\mathcal{O}_i,\mathcal{O}_k;\zeta,\boldsymbol{\lambda})\middle|\mathcal{O}_i\right\} = \boldsymbol{\varphi}_v^{\mathrm{eff}}(\mathcal{O}_i;\zeta,\boldsymbol{\lambda}),$$

which is the EIF for $\boldsymbol{\lambda}_v$ as we showed in the previous sections. Therefore, $\widehat{\boldsymbol{\lambda}}_v^{\mathrm{dml}}$ attains the semiparametric efficiency lower bound under the regularity conditions.

Lastly, we prove the consistency of the variance estimator $\widehat{\boldsymbol{V}}_v^{\mathrm{dml}}$ for $\boldsymbol{V}_v^{\mathrm{eff},0}$, where $\widehat{\boldsymbol{V}}_v^{\mathrm{dml}} = (\widehat{\boldsymbol{B}}_v^{\mathrm{dml}})^{-1}\widehat{\boldsymbol{\Sigma}}_v^{\mathrm{dml}}\{(\widehat{\boldsymbol{B}}_v^{\mathrm{dml}})^{-1}\}^\top$, with

$$\widehat{\boldsymbol{B}}_v^{\mathrm{dml}} = \binom{m}{2}^{-1}\sum_{p=1}^{|\mathfrak{I}^{\mathrm{pr}}|}\sum_{(i,k)\in\mathcal{I}_p^{\mathrm{pr}}} \nabla_{\boldsymbol{\lambda}}\boldsymbol{\psi}_v^{\mathrm{eff}}(\mathcal{O}_i,\mathcal{O}_k;\widehat{\zeta}_p,\widehat{\boldsymbol{\lambda}}_v^{\mathrm{dml}}),$$
$$\widehat{\boldsymbol{\Sigma}}_v^{\mathrm{dml}} = \frac{4}{m-1}\sum_{i=1}^{m}\widehat{\boldsymbol{\psi}}_v^{\mathrm{dml}}(\mathcal{O}_i;\widehat{\zeta},\widehat{\boldsymbol{\lambda}}_v^{\mathrm{dml}})\widehat{\boldsymbol{\psi}}_v^{\mathrm{dml}}(\mathcal{O}_i;\widehat{\zeta},\widehat{\boldsymbol{\lambda}}_v^{\mathrm{dml}})^\top,$$

and

$$\widehat{\boldsymbol{\psi}}_v^{\mathrm{dml}}(\mathcal{O}_i;\widehat{\zeta},\widehat{\boldsymbol{\lambda}}_v^{\mathrm{dml}}) = \frac{1}{m-1}\sum_{k:k\neq i}\sum_{p=1}^{|\mathfrak{I}^{\mathrm{pr}}|}\mathbb{1}\{(i,k)\in\mathcal{I}_p^{\mathrm{pr}}\}\boldsymbol{\psi}_v^{\mathrm{eff}}(\mathcal{O}_i,\mathcal{O}_k;\widehat{\zeta}_p,\widehat{\boldsymbol{\lambda}}_v^{\mathrm{dml}}).$$

We first show $\widehat{\boldsymbol{B}}_v^{\mathrm{dml}} \xrightarrow{p} \boldsymbol{B}_{v,\boldsymbol{\lambda}}^{\mathrm{eff},0}$. Specifically,

$$\left\|\widehat{\boldsymbol{B}}_v^{\mathrm{dml}} - \boldsymbol{B}_{v,\boldsymbol{\lambda}}^{\mathrm{eff},0}\right\| \le \left\|\widehat{\boldsymbol{B}}_v^{\mathrm{dml}} - \boldsymbol{B}_{v,\boldsymbol{\lambda}}^{\mathrm{eff}}(\widehat{\zeta},\widehat{\boldsymbol{\lambda}}_v^{\mathrm{dml}})\right\| + \left\|\boldsymbol{B}_{v,\boldsymbol{\lambda}}^{\mathrm{eff}}(\widehat{\zeta},\widehat{\boldsymbol{\lambda}}_v^{\mathrm{dml}}) - \boldsymbol{B}_{v,\boldsymbol{\lambda}}^{\mathrm{eff},0}\right\|,$$

where

$$\boldsymbol{B}_{v,\boldsymbol{\lambda}}^{\mathrm{eff}}(\widehat{\zeta},\widehat{\boldsymbol{\lambda}}_v^{\mathrm{dml}}) = \mathbb{E}\left\{\binom{m}{2}^{-1}\sum_{p=1}^{|\mathfrak{I}^{\mathrm{pr}}|}\sum_{(i,k)\in\mathcal{I}_p^{\mathrm{pr}}}\nabla_{\boldsymbol{\lambda}}\boldsymbol{\psi}_v^{\mathrm{eff}}(\mathcal{O}_i,\mathcal{O}_k;\widehat{\zeta}_p,\widehat{\boldsymbol{\lambda}}_v^{\mathrm{dml}})\middle|\widehat{\zeta},\widehat{\boldsymbol{\lambda}}_v^{\mathrm{dml}}\right\}.$$

The second term is the approximation error. By regularity condition (A5),

$$\left\|\boldsymbol{B}_{v,\boldsymbol{\lambda}}^{\mathrm{eff}}(\widehat{\zeta},\widehat{\boldsymbol{\lambda}}_v^{\mathrm{dml}}) - \boldsymbol{B}_{v,\boldsymbol{\lambda}}^{\mathrm{eff},0}\right\| \le \mathbb{E}\{\dot{e}(\mathcal{O}_i,\mathcal{O}_k)\}\left(\left\|\widehat{\zeta}-\zeta^0\right\| + \left\|\widehat{\boldsymbol{\lambda}}_v^{\mathrm{dml}} - \boldsymbol{\lambda}_v^0\right\|\right) = o_{\mathbb{P}}(1).$$

The first term is the statistical error. By the Hoeffding decomposition, for fixed $(\widehat{\zeta}, \widehat{\boldsymbol{\lambda}}_v^{\text{dml}})$,

$$\widehat{\boldsymbol{B}}_v^{\text{dml}} - \boldsymbol{B}_{v,\boldsymbol{\lambda}}^{\text{eff}}(\widehat{\zeta}, \widehat{\boldsymbol{\lambda}}_v^{\text{dml}}) = \frac{2}{m}\sum_{i=1}^{m} \boldsymbol{b}_{v,1}(\mathcal{O}_i; \widehat{\zeta}, \widehat{\boldsymbol{\lambda}}_v^{\text{dml}}) + \boldsymbol{r}_{v,m}(\widehat{\zeta}, \widehat{\boldsymbol{\lambda}}_v^{\text{dml}}),$$

where

$$\boldsymbol{b}_{v,1}(\mathcal{O}_i; \widehat{\zeta}, \widehat{\boldsymbol{\lambda}}_v^{\text{dml}}) = \mathbb{E}\left\{\nabla_{\boldsymbol{\lambda}} \boldsymbol{\psi}_v^{\text{eff}}(\mathcal{O}_i, \mathcal{O}_k; \widehat{\zeta}, \widehat{\boldsymbol{\lambda}}_v^{\text{dml}}) \Big| \mathcal{O}_i\right\} - \mathbb{E}\left\{\nabla_{\boldsymbol{\lambda}} \boldsymbol{\psi}_v^{\text{eff}}(\mathcal{O}_i, \mathcal{O}_k; \widehat{\zeta}, \widehat{\boldsymbol{\lambda}}_v^{\text{dml}})\right\},$$
$$\mathbb{E}\left\{\boldsymbol{b}_{v,1}(\mathcal{O}_i; \widehat{\zeta}, \widehat{\boldsymbol{\lambda}}_v^{\text{dml}})\right\} = \boldsymbol{0}, \quad \mathbb{E}\left\{\left\|\boldsymbol{r}_{v,m}(\widehat{\zeta}, \widehat{\boldsymbol{\lambda}}_v^{\text{dml}})\right\|^2\right\} = O(m^{-1}).$$

By the sample-splitting scheme, for each fold $p$, $\widehat{\zeta}_p$ is independent of $\mathcal{O}_i$ for $i$ involved in the index pairs in $\mathcal{I}_p^{\text{pr}}$. We denote this by $i \in \mathcal{I}_p^{\text{pr}}$ with a slight abuse of notation. Thus, conditional on $(\mathcal{I}_p^{\text{pr}})^c$, the terms $\{\boldsymbol{b}_{v,1}(\mathcal{O}_i; \widehat{\zeta}, \widehat{\boldsymbol{\lambda}}_v^{\text{dml}}), i \in \mathcal{I}_p^{\text{pr}}\}$ are independent with mean zero.

We next apply the weak law of large numbers for triangular arrays (Durrett and Durrett, 2019, Theorem 2.2.6). The Lindeberg condition, i.e., for any $\epsilon > 0$,

$$m^{-1}\sum_{i=1}^{m} \mathbb{E}\left[\left\|\boldsymbol{b}_{v,1}(\mathcal{O}_i; \widehat{\zeta}, \widehat{\boldsymbol{\lambda}}_v^{\text{dml}})\right\|^2 \mathbb{1}\left\{\left\|\boldsymbol{b}_{v,1}(\mathcal{O}_i; \widehat{\zeta}, \widehat{\boldsymbol{\lambda}}_v^{\text{dml}})\right\| > \epsilon m^{1/2}\right\}\right] \to 0,$$

holds by the uniform integrability from regularity conditions (A4) and (V1), and the consistency of $(\widehat{\zeta}, \widehat{\boldsymbol{\lambda}}_v^{\text{dml}})$. The degenerate term $\boldsymbol{r}_{v,m}(\widehat{\zeta}, \widehat{\boldsymbol{\lambda}}_v^{\text{dml}})$ satisfies $\mathbb{E}(\|\boldsymbol{r}_{v,m}(\widehat{\zeta}, \widehat{\boldsymbol{\lambda}}_v^{\text{dml}})\|) \leq [\mathbb{E}\{\|\boldsymbol{r}_{v,m}(\widehat{\zeta}, \widehat{\boldsymbol{\lambda}}_v^{\text{dml}})\|^2\}]^{1/2} = O(m^{-1/2}) = o(1)$. Thus, $\|\widehat{\boldsymbol{B}}_v^{\text{dml}} - \boldsymbol{B}_{v,\boldsymbol{\lambda}}^{\text{eff},0}\| = o_{\mathbb{P}}(1)$.

We then show $\widehat{\boldsymbol{\Sigma}}_v^{\text{dml}} \xrightarrow{p} \boldsymbol{\Sigma}_v^{\text{eff},0}$. Let $\overline{\boldsymbol{\psi}}_v^{\text{eff}}(\mathcal{O}_i; \zeta, \boldsymbol{\lambda}) = \mathbb{E}\{\boldsymbol{\psi}_v^{\text{eff}}(\mathcal{O}_i, \mathcal{O}_k; \zeta, \boldsymbol{\lambda})|\mathcal{O}_i\}$. The intermediate result is to show the Hájek projection consistency, i.e.,

$$m^{-1}\sum_{i=1}^{m} \left\|\widehat{\boldsymbol{\psi}}_v^{\text{eff}}(\mathcal{O}_i; \widehat{\zeta}, \widehat{\boldsymbol{\lambda}}_v^{\text{dml}}) - \overline{\boldsymbol{\psi}}_v^{\text{eff}}(\mathcal{O}_i; \zeta^0, \boldsymbol{\lambda}_v^0)\right\|^2 = o_{\mathbb{P}}(1).$$

We have the following decomposition,

$$\begin{aligned} &\left\|\widehat{\boldsymbol{\psi}}_v^{\text{eff}}(\mathcal{O}_i; \widehat{\zeta}, \widehat{\boldsymbol{\lambda}}_v^{\text{dml}}) - \overline{\boldsymbol{\psi}}_v^{\text{eff}}(\mathcal{O}_i; \zeta^0, \boldsymbol{\lambda}_v^0)\right\| \\ \leq &\left\|\widehat{\boldsymbol{\psi}}_v^{\text{eff}}(\mathcal{O}_i; \widehat{\zeta}, \widehat{\boldsymbol{\lambda}}_v^{\text{dml}}) - \overline{\boldsymbol{\psi}}_v^{\text{eff}}(\mathcal{O}_i; \widehat{\zeta}, \widehat{\boldsymbol{\lambda}}_v^{\text{dml}})\right\| + \left\|\overline{\boldsymbol{\psi}}_v^{\text{eff}}(\mathcal{O}_i; \widehat{\zeta}, \widehat{\boldsymbol{\lambda}}_v^{\text{dml}}) - \overline{\boldsymbol{\psi}}_v^{\text{eff}}(\mathcal{O}_i; \zeta^0, \boldsymbol{\lambda}_v^0)\right\|, \end{aligned} \tag{S13}$$

where $\overline{\boldsymbol{\psi}}_v^{\text{eff}}(\mathcal{O}_i; \widehat{\zeta}, \widehat{\boldsymbol{\lambda}}_v^{\text{dml}}) = \mathbb{E}\{\boldsymbol{\psi}_v^{\text{eff}}(\mathcal{O}_i, \mathcal{O}_k; \widehat{\zeta}, \widehat{\boldsymbol{\lambda}}_v^{\text{dml}})|\mathcal{O}_i\}$. For the second term on the right-hand side of (S13), regularity condition (C4) and Jensen's inequality imply that there exists a square-integrable function $\overline{e}(\mathcal{O}_i)$ such that

$$\left\|\overline{\boldsymbol{\psi}}_v^{\text{eff}}(\mathcal{O}_i; \zeta, \boldsymbol{\lambda}) - \overline{\boldsymbol{\psi}}_v^{\text{eff}}(\mathcal{O}_i; \widetilde{\zeta}, \widetilde{\boldsymbol{\lambda}})\right\| \leq \overline{e}(\mathcal{O}_i)\left(\left\|\zeta - \widetilde{\zeta}\right\| + \left\|\boldsymbol{\lambda} - \widetilde{\boldsymbol{\lambda}}\right\|\right).$$

Therefore,

$$\left\|\overline{\boldsymbol{\psi}}_v^{\text{eff}}(\mathcal{O}_i; \widehat{\zeta}, \widehat{\boldsymbol{\lambda}}_v^{\text{dml}}) - \overline{\boldsymbol{\psi}}_v^{\text{eff}}(\mathcal{O}_i; \zeta^0, \boldsymbol{\lambda}_v^0)\right\| \leq \mathbb{E}\{\overline{e}(\mathcal{O}_i)\}\left(\left\|\widehat{\zeta} - \zeta^0\right\| + \left\|\widehat{\boldsymbol{\lambda}}_v^{\text{dml}} - \boldsymbol{\lambda}_v^0\right\|\right),$$

which leads to

$$
\begin{aligned}
& m^{-1}\sum_{i=1}^{m}\left\|\overline{\boldsymbol{\psi}}_v^{\text{eff}}(\mathcal{O}_i;\widehat{\zeta},\widehat{\boldsymbol{\lambda}}_v^{\text{dml}})-\overline{\boldsymbol{\psi}}_v^{\text{eff}}(\mathcal{O}_i;\zeta^0,\boldsymbol{\lambda}_v^0)\right\|^2 \\
&\leq \left[m^{-1}\sum_{i=1}^{m}\mathbb{E}\{\overline{e}(\mathcal{O}_i)\}^2\right]\left(\left\|\widehat{\zeta}-\zeta^0\right\|+\left\|\widehat{\boldsymbol{\lambda}}_v^{\text{dml}}-\boldsymbol{\lambda}_v^0\right\|\right)^2=o_{\mathbb{P}}(1).
\end{aligned}
$$

For the first term on the right-hand side of (S13), by the Marcinkiewicz-Zygmund inequality (Chow and Teicher, 1997, pp. 386),

$$
\begin{aligned}
& \mathbb{E}\left\{\left\|\widehat{\boldsymbol{\psi}}_v^{\text{eff}}(\mathcal{O}_i;\widehat{\zeta},\widehat{\boldsymbol{\lambda}}_v^{\text{dml}})-\overline{\boldsymbol{\psi}}_v^{\text{eff}}(\mathcal{O}_i;\widehat{\zeta},\widehat{\boldsymbol{\lambda}}_v^{\text{dml}})\right\|^4\middle|\mathcal{O}_i\right\} \\
&=\mathbb{E}\left\{\left\|\frac{1}{m-1}\sum_{k:k\neq i}\left\{\boldsymbol{\psi}_v^{\text{eff}}(\mathcal{O}_i,\mathcal{O}_k;\widehat{\zeta},\widehat{\boldsymbol{\lambda}}_v^{\text{dml}})-\overline{\boldsymbol{\psi}}_v^{\text{eff}}(\mathcal{O}_i;\widehat{\zeta},\widehat{\boldsymbol{\lambda}}_v^{\text{dml}})\right\}\right\|^4\middle|\mathcal{O}_i\right\} \\
&\leq \frac{K}{(m-1)^2}\mathbb{E}\left\{\left\|\boldsymbol{\psi}_v^{\text{eff}}(\mathcal{O}_i,\mathcal{O}_k;\widehat{\zeta},\widehat{\boldsymbol{\lambda}}_v^{\text{dml}})-\overline{\boldsymbol{\psi}}_v^{\text{eff}}(\mathcal{O}_i;\widehat{\zeta},\widehat{\boldsymbol{\lambda}}_v^{\text{dml}})\right\|^4\middle|\mathcal{O}_i\right\},
\end{aligned}
$$

for some constant $K>0$. By the $c_r$-inequality (Loève, 1977, pp. 157),

$$
\begin{aligned}
& \mathbb{E}\left\{\left\|\boldsymbol{\psi}_v^{\text{eff}}(\mathcal{O}_i,\mathcal{O}_k;\widehat{\zeta},\widehat{\boldsymbol{\lambda}}_v^{\text{dml}})-\overline{\boldsymbol{\psi}}_v^{\text{eff}}(\mathcal{O}_i;\widehat{\zeta},\widehat{\boldsymbol{\lambda}}_v^{\text{dml}})\right\|^4\middle|\mathcal{O}_i\right\} \\
&\leq 8\left[\mathbb{E}\left\{\left\|\boldsymbol{\psi}_v^{\text{eff}}(\mathcal{O}_i,\mathcal{O}_k;\widehat{\zeta},\widehat{\boldsymbol{\lambda}}_v^{\text{dml}})\right\|^4\middle|\mathcal{O}_i\right\}+\left\|\overline{\boldsymbol{\psi}}_v^{\text{eff}}(\mathcal{O}_i;\widehat{\zeta},\widehat{\boldsymbol{\lambda}}_v^{\text{dml}})\right\|^4\right],
\end{aligned}
$$

and by Jensen's inequality

$$
\left\|\overline{\boldsymbol{\psi}}_v^{\text{eff}}(\mathcal{O}_i;\widehat{\zeta},\widehat{\boldsymbol{\lambda}}_v^{\text{dml}})\right\|^4\leq\mathbb{E}\left\{\left\|\boldsymbol{\psi}_v^{\text{eff}}(\mathcal{O}_i,\mathcal{O}_k;\widehat{\zeta},\widehat{\boldsymbol{\lambda}}_v^{\text{dml}})\right\|^4\middle|\mathcal{O}_i\right\}.
$$

Therefore,

$$
\mathbb{E}\left\{\left\|\boldsymbol{\psi}_v^{\text{eff}}(\mathcal{O}_i,\mathcal{O}_k;\widehat{\zeta},\widehat{\boldsymbol{\lambda}}_v^{\text{dml}})-\overline{\boldsymbol{\psi}}_v^{\text{eff}}(\mathcal{O}_i;\widehat{\zeta},\widehat{\boldsymbol{\lambda}}_v^{\text{dml}})\right\|^4\middle|\mathcal{O}_i\right\}\leq 16\mathbb{E}\left\{\left\|\boldsymbol{\psi}_v^{\text{eff}}(\mathcal{O}_i,\mathcal{O}_k;\widehat{\zeta},\widehat{\boldsymbol{\lambda}}_v^{\text{dml}})\right\|^4\middle|\mathcal{O}_i\right\}
$$

By regularity condition (V1) and taking the expectation w.r.t $\mathcal{O}_i$, we have

$$
\begin{aligned}
& \mathbb{E}\left\{\left\|\widehat{\boldsymbol{\psi}}_v^{\text{eff}}(\mathcal{O}_i;\widehat{\zeta},\widehat{\boldsymbol{\lambda}}_v^{\text{dml}})-\overline{\boldsymbol{\psi}}_v^{\text{eff}}(\mathcal{O}_i;\widehat{\zeta},\widehat{\boldsymbol{\lambda}}_v^{\text{dml}})\right\|^4\right\} \\
&\leq \frac{16K}{(m-1)^2}\mathbb{E}\left\{\left\|\boldsymbol{\psi}_v^{\text{eff}}(\mathcal{O}_i,\mathcal{O}_k;\widehat{\zeta},\widehat{\boldsymbol{\lambda}}_v^{\text{dml}})\right\|^4\right\}\{1+o(1)\}=O(m^{-2}).
\end{aligned}
$$

By Lyapunov's inequality (Loève, 1977, pp. 158),

$$
\begin{aligned}
& \mathbb{E}\left\{\left\|\widehat{\boldsymbol{\psi}}_v^{\text{eff}}(\mathcal{O}_i;\widehat{\zeta},\widehat{\boldsymbol{\lambda}}_v^{\text{dml}})-\overline{\boldsymbol{\psi}}_v^{\text{eff}}(\mathcal{O}_i;\widehat{\zeta},\widehat{\boldsymbol{\lambda}}_v^{\text{dml}})\right\|^2\right\} \\
&\leq \left[\mathbb{E}\left\{\left\|\widehat{\boldsymbol{\psi}}_v^{\text{eff}}(\mathcal{O}_i;\widehat{\zeta},\widehat{\boldsymbol{\lambda}}_v^{\text{dml}})-\overline{\boldsymbol{\psi}}_v^{\text{eff}}(\mathcal{O}_i;\widehat{\zeta},\widehat{\boldsymbol{\lambda}}_v^{\text{dml}})\right\|^4\right\}\right]^{1/2}=O(m^{-1}).
\end{aligned}
$$

Thus,

$$\mathbb{E}\left\{m^{-1}\sum_{i=1}^{m}\left\|\widehat{\boldsymbol{\psi}}_v^{\rm eff}(\mathcal{O}_i;\widehat{\zeta},\widehat{\boldsymbol{\lambda}}_v^{\rm dml})-\overline{\boldsymbol{\psi}}_v^{\rm eff}(\mathcal{O}_i;\widehat{\zeta},\widehat{\boldsymbol{\lambda}}_v^{\rm dml})\right\|^2\right\}=O(m^{-1})=o(1),$$

and by Markov's inequality,

$$m^{-1}\sum_{i=1}^{m}\left\|\widehat{\boldsymbol{\psi}}_v^{\rm eff}(\mathcal{O}_i;\widehat{\zeta},\widehat{\boldsymbol{\lambda}}_v^{\rm dml})-\overline{\boldsymbol{\psi}}_v^{\rm eff}(\mathcal{O}_i;\widehat{\zeta},\widehat{\boldsymbol{\lambda}}_v^{\rm dml})\right\|^2=o_{\mathbb{P}}(1).$$

Let $\widehat{\boldsymbol{\psi}}_{v,i}^{\rm dml}=\widehat{\boldsymbol{\psi}}_v^{\rm eff}(\mathcal{O}_i;\widehat{\zeta},\widehat{\boldsymbol{\lambda}}_v^{\rm dml})$ and $\widehat{\boldsymbol{\psi}}_v^{\rm dml}=m^{-1}\sum_{i=1}^{m}\widehat{\boldsymbol{\psi}}_{v,i}^{\rm dml}=\mathbf{0}$. Then,

$$\widehat{\boldsymbol{\Sigma}}_v^{\rm dml}=\frac{4}{m-1}\sum_{i=1}^{m}\widehat{\boldsymbol{\psi}}_{v,i}^{\rm dml}(\widehat{\boldsymbol{\psi}}_{v,i}^{\rm dml})^\top.$$

By the intermediate result that $\widehat{\boldsymbol{\psi}}_{v,i}^{\rm dml}\xrightarrow{p}\overline{\boldsymbol{\psi}}_v^{\rm eff}(\mathcal{O}_i;\zeta^0,\boldsymbol{\lambda}_v^0)$ and the continuous mapping theorem,

$$\frac{1}{m-1}\sum_{i=1}^{m}\widehat{\boldsymbol{\psi}}_{v,i}^{\rm dml}(\widehat{\boldsymbol{\psi}}_{v,i}^{\rm dml})^\top=\frac{1}{m-1}\sum_{i=1}^{m}\overline{\boldsymbol{\psi}}_v^{\rm eff}(\mathcal{O}_i;\zeta^0,\boldsymbol{\lambda}_v^0)\overline{\boldsymbol{\psi}}_v^{\rm eff}(\mathcal{O}_i;\zeta^0,\boldsymbol{\lambda}_v^0)^\top+\boldsymbol{o}_{\mathbb{P}}(1).$$

The law of large numbers gives us

$$\frac{1}{m-1}\sum_{i=1}^{m}\overline{\boldsymbol{\psi}}_v^{\rm eff}(\mathcal{O}_i;\zeta^0,\boldsymbol{\lambda}_v^0)\overline{\boldsymbol{\psi}}_v^{\rm eff}(\mathcal{O}_i;\zeta^0,\boldsymbol{\lambda}_v^0)^\top\xrightarrow{p}\mathbb{E}\left\{\overline{\boldsymbol{\psi}}_v^{\rm eff}(\mathcal{O}_i;\zeta^0,\boldsymbol{\lambda}_v^0)\overline{\boldsymbol{\psi}}_v^{\rm eff}(\mathcal{O}_i;\zeta^0,\boldsymbol{\lambda}_v^0)^\top\right\}.$$

By the Neyman orthogonality of the EIF and the Delta method,

$$\mathbb{E}\left(\widehat{\boldsymbol{\psi}}_{v,i}^{\rm dml}\right)=\mathbb{E}\left\{\overline{\boldsymbol{\psi}}_v^{\rm eff}(\mathcal{O}_i;\widehat{\zeta},\widehat{\boldsymbol{\lambda}}_v^{\rm dml})\right\}=\boldsymbol{O}\left(\left\|\widehat{\zeta}-\zeta^0\right\|^2+\left\|\widehat{\boldsymbol{\lambda}}_v^{\rm dml}-\boldsymbol{\lambda}_v^0\right\|^2\right)=\boldsymbol{o}_{\mathbb{P}}(1),$$

by regularity condition (A1). The variance of $\widehat{\boldsymbol{\psi}}_{v,i}^{\rm dml}$ is $\boldsymbol{O}(m^{-1})$ as shown previously. Therefore, by Markov's inequality, $\widehat{\boldsymbol{\psi}}_{v,i}^{\rm dml}=\boldsymbol{o}_{\mathbb{P}}(1)$. Since $\mathbb{E}\{\overline{\boldsymbol{\psi}}_v^{\rm eff}(\mathcal{O}_i;\zeta^0,\boldsymbol{\lambda}_v^0)\}=\mathbf{0}$, we have $\boldsymbol{\Sigma}_v^{\rm eff,0}=4\mathbb{E}\{\overline{\boldsymbol{\psi}}_v^{\rm eff}(\mathcal{O}_i;\zeta^0,\boldsymbol{\lambda}_v^0)\overline{\boldsymbol{\psi}}_v^{\rm eff}(\mathcal{O}_i;\zeta^0,\boldsymbol{\lambda}_v^0)^\top\}$. Thus, $\widehat{\boldsymbol{\Sigma}}_v^{\rm dml}\xrightarrow{p}\boldsymbol{\Sigma}_v^{\rm eff,0}$. By the continuous mapping theorem, $\widehat{\boldsymbol{V}}_v^{\rm dml}\xrightarrow{p}\boldsymbol{V}_v^{\rm eff,0}$.

The consistency and asymptotic normality of $\widehat{\Lambda}_v^{\rm dml}$ are obtained via the continuous mapping theorem. The asymptotic variance estimators of $m^{1/2}\widehat{\Lambda}_v^{\rm dml}$, $\widehat{V}_v^{\rm dml}$, can be obtained by applying the Delta method to $\widehat{\boldsymbol{V}}_v^{\rm dml}$, with $\widehat{V}_v^{\rm dml}\xrightarrow{p}V_v^{\rm eff,0}$. Slutsky's theorem implies the result in the theorem statement.

□

# S6 The subsample-based estimators

*Proof of Theorem 5.* We focus the arguments on $\widehat{\boldsymbol{\lambda}}_v^{\rm est,*}$ and $\widehat{\boldsymbol{V}}_v^{\rm est,*}$ for conciseness. Let $\mathcal{M}_r$ denote the indices of the subsample $r$, where $|\mathcal{M}_r|=m_r$ with $m_r=O(m)$, for $r=1,\ldots,R$. The consistency and asymptotic normality of $\widehat{\boldsymbol{\lambda}}_v^{{\rm est},(r)}$ are inherited from those of $\widehat{\boldsymbol{\lambda}}_v^{\rm est}$ for $r=1,\ldots,R$, est $=$ np, mr, dml, and $v=C,I$. Similarly, $\widehat{\boldsymbol{V}}_v^{{\rm est},(r)}$ is consistent for $\boldsymbol{V}_v^{\rm est}$. Let $\boldsymbol{\varphi}_v^{\rm est}(\mathcal{O}_i;\boldsymbol{\theta}_v^{\rm est})$ denote the influence function for $\widehat{\boldsymbol{\lambda}}_v^{\rm est}$, where $\boldsymbol{\theta}_v^{\rm np}=\boldsymbol{\lambda}_v$, $\boldsymbol{\theta}_v^{\rm mr}=(\boldsymbol{\vartheta},\boldsymbol{\lambda}_v)$, and

$\boldsymbol{\theta}_v^{\mathrm{dml}} = (\zeta, \boldsymbol{\lambda}_v)$. Then, we have

$$m_r^{1/2}(\widehat{\boldsymbol{\lambda}}_v^{\mathrm{est},(r)} - \boldsymbol{\lambda}_v^0) = \frac{2}{\sqrt{m_r}} \sum_{i \in \mathcal{M}_r} \boldsymbol{\varphi}_v^{\mathrm{est}}(\mathcal{O}_i; \boldsymbol{\theta}_v^{\mathrm{est}}) + \boldsymbol{o}_{\mathbb{P}}(1).$$

Since the $R$ subsamples are independent,

$$R^{-1} \sum_{r=1}^{R} m_r^{1/2}(\widehat{\boldsymbol{\lambda}}_v^{\mathrm{est},(r)} - \boldsymbol{\lambda}_v^0) = m^{1/2} \left( R^{-1} \sum_{r=1}^{R} \widehat{\boldsymbol{\lambda}}_v^{\mathrm{est},(r)} - \boldsymbol{\lambda}_v^0 \right) + \boldsymbol{o}_{\mathbb{P}}(1)$$
$$\iff m^{1/2}(\widehat{\boldsymbol{\lambda}}_v^{\mathrm{est},*} - \boldsymbol{\lambda}_v^0) = \frac{2}{\sqrt{m}} \sum_{i=1}^{m} \boldsymbol{\varphi}_v^{\mathrm{est}}(\mathcal{O}_i; \boldsymbol{\theta}_v^{\mathrm{est}}) + \boldsymbol{o}_{\mathbb{P}}(1).$$

Thus, $\widehat{\boldsymbol{\lambda}}_v^{\mathrm{est},*}$ has the same influence function as $\widehat{\boldsymbol{\lambda}}_v^{\mathrm{est}}$. The continuous mapping theorem and Slutsky's theorem imply the result in the theorem statement. □

## S6.1 Some discussions on the proposed approach

This proposed approach is a specific and highly structured type of the incomplete U-statistic (Blom, 1976). More specifically, in the context of modern statistical literature, particularly in the context of big data and parallel computing, we can refer to this specific construction as a *divide-and-conquer U-statistic* or a *block-diagonal design*.

An incomplete U-statistic is broadly defined as any U-statistic that sums over a subset of the possible kernel indices rather than all combinations. The classic incomplete U-statistics (Blom, 1976) use *random sampling*, e.g., selecting $M$ pairs at random from the pool of $\binom{m}{2}$. While efficient, random access to data can be computationally expensive in distributed systems. Our block-design divides the sample into $R$ disjoint groups and computes the U-statistic (U-estimating equation) for each, effectively selecting a *deterministic subset* of pairs. If we visualize the interaction matrix of all samples as an $m \times m$ grid), a complete U-statistic calculates the entire upper triangle. The subsample-based method calculates only the "blocks" along the diagonal.

The preservation of the asymptotic efficiency lies in the Hoeffding decomposition (van der Vaart, 1998, \$11.4). The variance of an order-two U-statistic is composed of terms of decreasing order:

$$\mathbb{V}\mathrm{ar}(U_n) = \frac{4\eta_1}{m} + O(m^{-2}).$$

The linear term $\eta_1$ represents the "main effect" of each individual data point. It captures how much the function changes when one observation varies. Because the subsample-based method uses every data point (just not every pair), this leading-order term is preserved perfectly. The quadratic term $O(m^{-2})$ captures the "interaction" between specific pairs. By ignoring the cross-group pairs (pairs where one point is in Group A and the other in Group B), the subsample-based method does not capture this interaction information. We lose information only in the $O(m^{-2})$ term. As $m \to \infty$, the linear term dominates, meaning the ratio of the variances approaches one. Therefore, we retain 100% of the first-order information while calculating only $R^{-1}$ of the second-order interactions.

## S7 Additional simulation results

We conducted simulation study III to demonstrate the finite-sample performance of the estimators based on subsamples. Specifically, we continue with the same settings as in simulation studies I and II, with the total number of clusters $m = 60$. We set $R = 2$, and thus for each dataset with $m = 60$ clusters, we obtain estimates $\widehat{\boldsymbol{\lambda}}_v^{\text{est},(r)}$ and $\widehat{\boldsymbol{V}}_v^{\text{est},(r)}$ for $r = 1, 2$ and $\text{est} = \text{np}, \text{mr}, \text{dml}$. The final estimate for $\boldsymbol{\lambda}_v$ is $\widehat{\boldsymbol{\lambda}}_v^{\text{est},*} = R^{-1}\sum_{r=1}^{R}\widehat{\boldsymbol{\lambda}}_v^{\text{est},(r)}$ and that for $\boldsymbol{V}_v^{\text{est}}$ is $\widehat{\boldsymbol{V}}_v^{\text{est},*} = R^{-1}\sum_{r=1}^{R}\widehat{\boldsymbol{V}}_v^{\text{est},(r)}$. For each setting, we simulate 500 replicates. The results using the full sample of $m = 60$ are also provided for comparison.

Web Table S1: Results from simulation study III, comparing with subsample-based estimators. NP: nonparametric; MB: model-robust; DML: debiased machine learning; SJZ: Smith et al. (2025). ESE: empirical standard error; ASE: average standard error; ECP: empirical coverage percentage of the 95% confidence interval. $m = 60$: estimation using the full sample of size $m = 60$; $m = 2 \times 30$: estimation using two subsamples of size $m = 30$.

| | | Simulation study I | | | | | | | |
|---|---|---|---|---|---|---|---|---|---|
| | | $\lambda_{C,1} = .588$ | | | | $\lambda_{I,1} = .603$ | | | |
| $m$ | Method | Bias | ESE | ASE | ECP | Bias | ESE | ASE | ECP |
| 60 | NP | −.001 | .029 | .027 | .926 | −.001 | .028 | .027 | .930 |
| | MR | −.001 | .024 | .024 | .948 | −.001 | .023 | .023 | .942 |
| | DML | −.001 | .023 | .023 | .934 | −.001 | .023 | .023 | .940 |
| | SJZ | .001 | .028 | .027 | .898 | −.001 | .028 | .027 | .934 |
| 2×30 | NP | −.002 | .029 | .027 | .926 | −.002 | .029 | .026 | .932 |
| | MB | −.003 | .027 | .025 | .928 | −.003 | .027 | .025 | .922 |
| | DML | −.002 | .026 | .026 | .924 | −.002 | .027 | .026 | .936 |
| | SJZ | .007 | .028 | .027 | .920 | −.008 | .028 | .027 | .928 |
| | | Simulation study II | | | | | | | |
| | | $\lambda_{C,1} = .621$ | | | | $\lambda_{I,1} = .649$ | | | |
| $m$ | Method | Bias | ESE | ASE | ECP | Bias | ESE | ASE | ECP |
| 60 | NP | .002 | .050 | .050 | .944 | .004 | .049 | .049 | .922 |
| | MR | .002 | .040 | .041 | .944 | .004 | .041 | .040 | .948 |
| | DML | .003 | .038 | .040 | .938 | .004 | .038 | .039 | .934 |
| | SJZ | .021 | .049 | .052 | .934 | −.006 | .049 | .052 | .940 |
| 2×30 | NP | .001 | .055 | .050 | .908 | .001 | .054 | .049 | .914 |
| | MB | .002 | .050 | .044 | .910 | .001 | .048 | .043 | .924 |
| | DML | .002 | .047 | .042 | .914 | .003 | .046 | .041 | .916 |
| | SJZ | .020 | .054 | .053 | .912 | −.007 | .054 | .053 | .924 |

Results from simulation study III are summarized in Web Table S1, with violin plots of the estimators given in Web Figure S1. It can be observed that the subsample-based estimators, i.e., NP, MR, and DML, are consistent. However, compared to estimators using the full sample, the subsample-based estimators exhibit a slight finite-sample efficiency loss, as their ESEs are slightly larger than those of the corresponding full-sample estimator. The variance estimators are consistent, which is more apparent under the setting of simulation study I. Since these estimators use smaller subsamples, small-sample variance-bias correction approaches are needed to ensure that the 95% confidence intervals achieve the

nominal level.

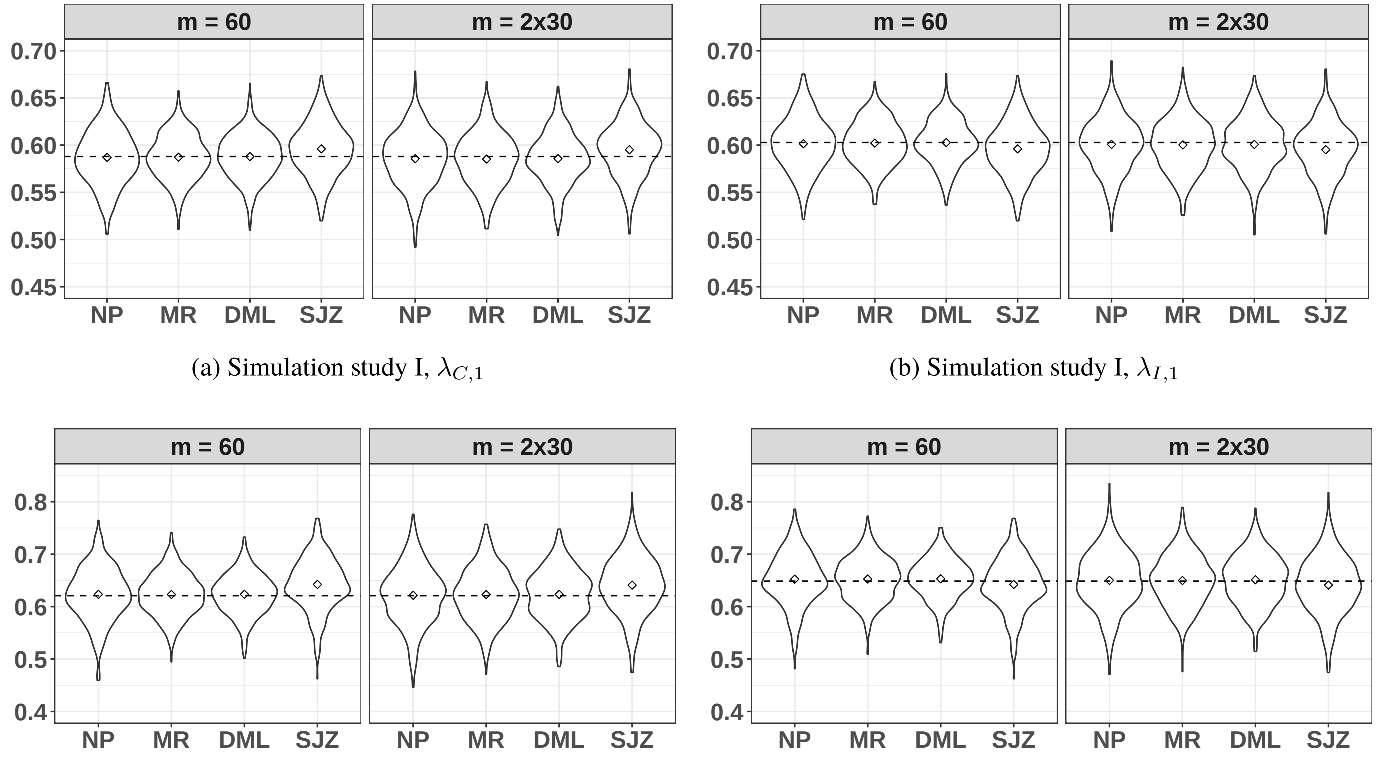


(a) Simulation study I, $\lambda_{C,1}$

(b) Simulation study I, $\lambda_{I,1}$

(c) Simulation study II, $\lambda_{C,1}$

(d) Simulation study II, $\lambda_{I,1}$

Web Figure S1: Violin plots of estimators from simulation studies I and II. NP: nonparametric; MR: model-robust; DML: debiased machine learning; SJZ: Smith et al. (2025). $m = 60$: estimation using the full sample of size $m = 60$; $m = 2 \times 30$: estimation using two subsamples of size $m = 30$.

For small-sample variance-bias correction, we adopted the convenient-to-implement DF-correction approach (MacKinnon and White, 1985; Li and Redden, 2015) introduced in the main article, where the final variance estimator $\widehat{\boldsymbol{V}}_v^{\text{est},*,\dagger} = (m/R)/\{(m/R) - p\} \cdot \widehat{\boldsymbol{V}}_v^{\text{est},*}$ and the standard normal quantiles are replaced by the $t_{m-p}$ quantiles. Here, similar to the main article, we set $p = 4$ for the degree-of-freedom loss. The results are summarized in Web Table S2. Across settings in simulation studies I and II, with the DF-correction, the ASEs of the NP, MR, and DML estimators are close to their corresponding ESEs, and the ECPs of the 95% confidence intervals are at their nominal level.

# S8 Theoretical results under the treatment-arm-specific within-cluster subsampling

## S8.1 Setting and assumptions

For the generality of our results, in this setting, we consider the possible treatment-arm-specific within-cluster subsampling. Specifically, let $M_i = \sum_{j=1}^{J} S_{ij} \leq N_i$ be the observed cluster size (number of units sampled into the study), where $S_{ij} \in \{0, 1\}$ is the sampling indicator. We thereby label $N_i$ as the original cluster size of cluster $i$. Under Assumption 1 in the main article, we have $M_i = A_i M_i(1) + (1 - A_i) M_i(0)$ and $S_{ij} = A_i S_{ij}(1) + (1 - A_i) S_{ij}(0)$. For cluster $i$, define $\boldsymbol{S}_i(a) = \{S_{ij}(a), j = 1, \ldots N_i\}$. Then, the full data for cluster $i$ in this setting is $\mathcal{D}_i = \{\mathbf{Y}_i(1), \mathbf{Y}_i(0), \boldsymbol{S}_i(1), \boldsymbol{S}_i(0), N_i, \boldsymbol{C}_i, \mathbf{X}_i\}$, and the observed data is $\mathcal{O}_i = \{\mathbf{Y}_i^o, A_i, N_i, M_i, \boldsymbol{C}_i, \mathbf{X}_i^o\}$, where $\mathbf{Y}_i^o = \{\boldsymbol{Y}_{ij} : S_{ij} = 1, j = 1, \ldots, N_i\}$ and $\mathbf{X}_i^o = \{\boldsymbol{X}_{ij} :$

Web Table S2: Results for the subsample-based estimators with finite-sample adjustments to the variance estimators under settings in simulation studies I and II, where $m = 2\times30$. NP: nonparametric; MR: model-robust; DML: debiased machine learning. ESE: empirical standard error; ASE: average standard error; ECP: empirical coverage percentage of the 95% confidence interval. ESE: empirical standard error; ASE$^\dagger$: average standard error after the DF-correction; ECP$^\dagger$: empirical coverage percentage of the 95% confidence interval after the DF-correction.

| Simulation study I | | | | | | | | | | |
|---|---|---|---|---|---|---|---|---|---|---|
| | $\lambda_{C,1} = .588$ | | | | | $\lambda_{I,1} = .603$ | | | | |
| Method | ESE | ASE | ECP | ASE$^\dagger$ | ECP$^\dagger$ | ESE | ASE | ECP | ASE$^\dagger$ | ECP$^\dagger$ |
| NP | .029 | .027 | .926 | .029 | .952 | .029 | .026 | .932 | .028 | .952 |
| MR | .027 | .025 | .928 | .027 | .952 | .027 | .025 | .922 | .026 | .952 |
| DML | .026 | .026 | .924 | .028 | .952 | .027 | .026 | .936 | .028 | .956 |
| Simulation study II | | | | | | | | | | |
| | $\lambda_{C,1} = .621$ | | | | | $\lambda_{I,1} = .649$ | | | | |
| Method | ESE | ASE | ECP | ASE$^\dagger$ | ECP$^\dagger$ | ESE | ASE | ECP | ASE$^\dagger$ | ECP$^\dagger$ |
| NP | .055 | .050 | .908 | .054 | .934 | .054 | .049 | .914 | .052 | .946 |
| MR | .050 | .044 | .910 | .047 | .932 | .048 | .043 | .924 | .047 | .950 |
| DML | .047 | .042 | .914 | .045 | .938 | .046 | .041 | .916 | .044 | .942 |

$S_{ij} = 1, j = 1, \dots, N_i\}$. In addition to Assumptions 1-3 in the main article, we make the following assumption regarding within-cluster subsampling.

**Assumption S1** (Cluster-dependent subsampling)**.** *For $a = 0, 1$, the potential observed cluster size $M(a) = h_a(N, \boldsymbol{C}, \epsilon_a)$ for some unknown function $h_a$ and exogenous random noise $\epsilon_a$ that is independent of $\{N, \boldsymbol{C}, \mathbf{X}, \mathbf{Y}(a)\}$. Furthermore, for each possible $N$-dimensional binary vector $\boldsymbol{s}$ with $M(a)$ ones,*

$$\mathbb{P}\{\boldsymbol{S}(a) = \boldsymbol{s} | \mathbf{Y}(a), M(a), \mathbf{X}, N, \boldsymbol{C}\} = \binom{N}{M(a)}^{-1}.$$

Assumption S1 implies that the number of observed individuals can depend on the assignment $A$ and cluster characteristics (cluster size $N$ and cluster-level covariates $\boldsymbol{C}$), but this subsampling process is completely random given the number of observed individuals and the cluster size. This assumption was adopted in Wang et al. (2024), which relaxes the setting of Bugni et al. (2025) to allow for treatment-arm-specific subsampling. Important special cases of Assumption S1 include full enrollment where $M(a) = N$; random subsampling with a treatment-arm-specific subsample size where $M(a) = m_a$ for some integer $m_a \leq N$; and independent cluster-specific subsampling such that each $S_{ij}(a)$ is independently determined by flipping a cluster-specific coin. Assumption S1 can be violated when the subsampling additionally depends on individual-level covariates, which are generally unobserved for nonparticipants.

## S8.2 Estimation

Similar to the main article, we propose estimators by solving various U-estimating equations. Section S8.2.1 presents the nonparametric estimators. Section S8.2.2 derives the EIF for the cp- and ip-GCE under within-cluster subsampling. Section S8.2.3 proposes the triply robust estimators motivated by the EIFs. Section S8.2.4 proposes the DML estimator using cross-fitting. The asymptotic properties of the estimators are also discussed under the regime of the number of

clusters $m \to \infty$.

### S8.2.1 The nonparametric estimators

Under within-cluster subsampling, the moment condition-motivated U-estimating equations are

$$\sum_{1\le i<k\le m} \boldsymbol{\psi}_v^{\mathrm{np}}(\mathcal{O}_i,\mathcal{O}_k;\boldsymbol{\lambda}) = \sum_{1\le i<k\le m} \left\{ \begin{array}{c} \psi_{v,1}^{\mathrm{np}}(\mathcal{O}_i,\mathcal{O}_k;\lambda_1) \\ \psi_{v,0}^{\mathrm{np}}(\mathcal{O}_i,\mathcal{O}_k;\lambda_0) \end{array} \right\} = \mathbf{0}, \tag{S14}$$

where $v = C, I$. For $a = 0, 1$,

$$\psi_{C,a}^{\mathrm{np}}(\mathcal{O}_i,\mathcal{O}_k;\lambda_a) = 2^{-1}\Bigg[\frac{\mathbb{1}(A_i=a)\mathbb{1}(A_k=1-a)}{M_iM_k}\sum_{j:S_{ij}=1}\sum_{l:S_{kl}=1}\{w(\boldsymbol{Y}_{ij},\boldsymbol{Y}_{kl})-\lambda_a\}$$
$$+\frac{\mathbb{1}(A_k=a)\mathbb{1}(A_i=1-a)}{M_iM_k}\sum_{j:S_{ij}=1}\sum_{l:S_{kl}=1}\{w(\boldsymbol{Y}_{kl},\boldsymbol{Y}_{ij})-\lambda_a\}\Bigg]$$

and $\boldsymbol{\psi}_I^{\mathrm{np}}(\mathcal{O}_i,\mathcal{O}_k;\boldsymbol{\lambda}) = N_iN_k\boldsymbol{\psi}_C^{\mathrm{np}}(\mathcal{O}_i,\mathcal{O}_k;\boldsymbol{\lambda})$. Solving (S14) leads to the nonparametric estimator $\widehat{\lambda}_{v,a}^{\mathrm{np}}$, and the nonparametric estimator for $\Lambda_v$ is $\widehat{\Lambda}_v^{\mathrm{np}} = f(\widehat{\lambda}_{v,1}^{\mathrm{np}},\widehat{\lambda}_{v,0}^{\mathrm{np}})$. Let $V_v^{\mathrm{np}}$ denote the asymptotic variance of $m^{1/2}\widehat{\Lambda}_v^{\mathrm{np}}$, with $\widehat{V}_v^{\mathrm{np}}$ denoting its estimator. We have the following theorem, which summarizes the properties of the nonparametric estimators.

**Theorem S1.** *Under Assumptions 1-3 in the main article and Assumption S1, for $v = C, I$, if regularity conditions (P1)-(P4) listed in Section S1 hold, then $\widehat{\boldsymbol{\lambda}}_v^{\mathrm{np}} \xrightarrow{p} \boldsymbol{\lambda}_v$; furthermore, if regularity conditions (P5)-(P7) also hold, then $m^{1/2}(\widehat{\boldsymbol{\lambda}}_v^{\mathrm{np}} - \boldsymbol{\lambda}_v) \xrightarrow{d} \mathcal{N}(\mathbf{0},\boldsymbol{V}_v^{\mathrm{np}})$ and $\widehat{\boldsymbol{V}}_v^{\mathrm{np}} \xrightarrow{p} \boldsymbol{V}_v^{\mathrm{np}}$.*

Define the Jacobian $\boldsymbol{B}_v^{\mathrm{np}} = \mathbb{E}\{\nabla_{\boldsymbol{\lambda}}\boldsymbol{\psi}_v^{\mathrm{np}}(\mathcal{O}_i,\mathcal{O}_k;\boldsymbol{\lambda}_v)\}$, where $\nabla_{\boldsymbol{\lambda}}\boldsymbol{\psi}_v^{\mathrm{np}}(\mathcal{O}_i,\mathcal{O}_k;\boldsymbol{\lambda}_v)$ is the first-order derivative of $\boldsymbol{\psi}_v^{\mathrm{np}}(\mathcal{O}_i,\mathcal{O}_k;\boldsymbol{\lambda})$ evaluated at $\boldsymbol{\lambda}_v = (\lambda_{v,1},\lambda_{v,0})^\top$, and the Hájek projection of the estimating function $\overline{\boldsymbol{\psi}}_v^{\mathrm{np}}(\mathcal{O}_i;\boldsymbol{\lambda}) = \mathbb{E}\{\boldsymbol{\psi}_v^{\mathrm{np}}(\mathcal{O}_i,\mathcal{O}_k;\boldsymbol{\lambda})|\mathcal{O}_i\}$. The asymptotic covariance matrix of $m^{1/2}\widehat{\boldsymbol{\lambda}}_v^{\mathrm{np}} = m^{1/2}(\widehat{\boldsymbol{\lambda}}_{v,1}^{\mathrm{np}},\widehat{\boldsymbol{\lambda}}_{v,0}^{\mathrm{np}})^\top$ is

$$\boldsymbol{V}_v^{\mathrm{np}} = (\boldsymbol{B}_v^{\mathrm{np}})^{-1}\boldsymbol{\Sigma}_v^{\mathrm{np}}\{(\boldsymbol{B}_v^{\mathrm{np}})^{-1}\}^\top,$$

where $\boldsymbol{\Sigma}_v^{\mathrm{np}} = 4\mathbb{V}\mathrm{ar}\{\overline{\boldsymbol{\psi}}_v^{\mathrm{np}}(\mathcal{O}_i;\boldsymbol{\lambda}_v)\}$, and the $V_v^{\mathrm{np}} = \{\nabla_{\boldsymbol{\lambda}}f(\boldsymbol{\lambda}_v)\}^\top\boldsymbol{V}_v^{\mathrm{np}}\nabla_{\boldsymbol{\lambda}}f(\boldsymbol{\lambda}_v)$ by the Delta method. The covariance matrix $\boldsymbol{V}_v^{\mathrm{np}}$ is estimated by the sandwich variance estimator, $\widehat{\boldsymbol{V}}_v^{\mathrm{np}} = (\widehat{\boldsymbol{B}}_v^{\mathrm{np}})^{-1}\widehat{\boldsymbol{\Sigma}}_v^{\mathrm{np}}\{(\widehat{\boldsymbol{B}}_v^{\mathrm{np}})^{-1}\}^\top$, where

$$\widehat{\boldsymbol{B}}_v^{\mathrm{np}} = \binom{m}{2}^{-1}\sum_{1\le i<k\le m}\nabla_{\boldsymbol{\lambda}}\psi_v^{\mathrm{np}}(\mathcal{O}_i,\mathcal{O}_k;\widehat{\boldsymbol{\lambda}}_v^{\mathrm{np}}),\quad \widehat{\boldsymbol{\Sigma}}_v^{\mathrm{np}} = \frac{4}{m-1}\sum_{i=1}^m\widehat{\boldsymbol{\psi}}_v^{\mathrm{np}}(\mathcal{O}_i;\widehat{\boldsymbol{\lambda}}_v^{\mathrm{np}})\widehat{\boldsymbol{\psi}}_v^{\mathrm{np}}(\mathcal{O}_i;\widehat{\boldsymbol{\lambda}}_v^{\mathrm{np}})^\top,$$

with $\widehat{\boldsymbol{\psi}}_v^{\mathrm{np}}(\mathcal{O}_i;\widehat{\boldsymbol{\lambda}}_v^{\mathrm{np}}) = (m-1)^{-1}\sum_{k:k\neq i}\boldsymbol{\psi}_v^{\mathrm{np}}(\mathcal{O}_i,\mathcal{O}_k;\widehat{\boldsymbol{\lambda}}_v^{\mathrm{np}})$. By Delta method, $\widehat{V}_v^{\mathrm{np}} = \{\nabla_{\boldsymbol{\lambda}}f(\widehat{\boldsymbol{\lambda}}_v^{\mathrm{np}})\}^\top\widehat{\boldsymbol{V}}_v^{\mathrm{np}}\nabla_{\boldsymbol{\lambda}}f(\widehat{\boldsymbol{\lambda}}_v^{\mathrm{np}})$. For $\widehat{\Lambda}_v^{\mathrm{np}}$, Theorem S1 implies that $(\widehat{V}_v^{\mathrm{np}})^{-1/2}(\widehat{\Lambda}_v^{\mathrm{np}} - \Lambda_v) \xrightarrow{d} \mathcal{N}(0,1)$ for $v = C, I$.

### S8.2.2 The efficient influence functions

We derive the EIFs for $\lambda_{C,a}$ and $\lambda_{I,a}$ under within-cluster subsampling. Define

$$\overline{w}(\mathbf{Y}_i^o, \mathbf{Y}_k^o) = \frac{1}{M_i M_k} \sum_{j:S_{ij}=1} \sum_{l:S_{kl}=1} w(\boldsymbol{Y}_{ij}, \boldsymbol{Y}_{kl})$$

as the observed average contrasts between two clusters regardless of treatments. The EIFs for $\lambda_{C,a}$ and $\lambda_{I,a}$ are given in Theorem S2.

**Theorem S2.** *(i) The EIF for $\lambda_{C,a}$ is*

$$\begin{aligned}
\varphi_{C,a}(\mathcal{O}) = &\frac{\mathbb{1}(A=a)}{\pi^a(1-\pi)^{1-a}}\left[\mathfrak{w}_{C,a,a}(\mathbf{Y}^o) - \mathbb{E}\left\{\mathfrak{w}_{C,a,a}(\mathbf{Y}^o)|\mathbf{X}^o, M, \boldsymbol{C}, N, A=a\right\}\right] \\
&+ \frac{\mathbb{1}(A=1-a)}{\pi^{1-a}(1-\pi)^{a}}\left[\mathfrak{w}_{C,a,1-a}(\mathbf{Y}^o) - \mathbb{E}\left\{\mathfrak{w}_{C,a,1-a}(\mathbf{Y}^o)|\mathbf{X}^o, M, \boldsymbol{C}, N, A=1-a\right\}\right] \\
&+ \frac{\mathbb{P}(A=a|M,\boldsymbol{C},N)}{\pi^a(1-\pi)^{1-a}}\left[\mathbb{E}\left\{\mathfrak{w}_{C,a,a}(\mathbf{Y}^o)|\mathbf{X}^o, M, \boldsymbol{C}, N, A=a\right\} - \mathbb{E}\left\{\mathfrak{w}_{C,a,a}(\mathbf{Y}^o)|\boldsymbol{C}, N, A=a\right\}\right] \\
&+ \frac{\mathbb{P}(A=1-a|M,\boldsymbol{C},N)}{\pi^{1-a}(1-\pi)^{a}}\left[\mathbb{E}\left\{\mathfrak{w}_{C,a,1-a}(\mathbf{Y}^o)|\mathbf{X}^o, M, \boldsymbol{C}, N, A=1-a\right\}\right. \\
&\qquad\qquad\left. - \mathbb{E}\left\{\mathfrak{w}_{C,a,1-a}(\mathbf{Y}^o)|\boldsymbol{C}, N, A=1-a\right\}\right] \\
&+ \mathbb{E}\left\{\mathfrak{w}_{C,a,a}(\mathbf{Y}^o)|\boldsymbol{C}, N, A=a\right\} + \mathbb{E}\left\{\mathfrak{w}_{C,a,1-a}(\mathbf{Y}^o)|\boldsymbol{C}, N, A=1-a\right\} - 2\lambda_{C,a},
\end{aligned}$$

*where* $\mathfrak{w}_{C,a,a}(\mathbf{y}) = \mathbb{E}\{\overline{w}(\mathbf{y}, \mathbf{Y}_k^o)|A_k = 1-a\}$ *and* $\mathfrak{w}_{C,a,1-a}(\mathbf{y}) = \mathbb{E}\{\overline{w}(\mathbf{Y}_k^o, \mathbf{y})|A_k = a\}$.

*(ii) The EIF for $\lambda_{I,a}$ is*

$$\begin{aligned}
\varphi_{I,a}(\mathcal{O}) = &\frac{\mathbb{1}(A=a)N}{\pi^a(1-\pi)^{1-a}\{\mathbb{E}(N)\}^2}\left[\mathfrak{w}_{I,a,a}(\mathbf{Y}^o) - \mathbb{E}\left\{\mathfrak{w}_{I,a,a}(\mathbf{Y}^o)|\mathbf{X}^o, M, \boldsymbol{C}, N, A=a\right\}\right] \\
&+ \frac{\mathbb{1}(A=1-a)N}{\pi^{1-a}(1-\pi)^{a}\{\mathbb{E}(N)\}^2}\left[\mathfrak{w}_{I,a,1-a}(\mathbf{Y}^o) - \mathbb{E}\left\{\mathfrak{w}_{I,a,1-a}(\mathbf{Y}^o)|\mathbf{X}^o, M, \boldsymbol{C}, N, A=1-a\right\}\right] \\
&+ \frac{\mathbb{P}(A=a|M,\boldsymbol{C},N)N}{\pi^a(1-\pi)^{1-a}\{\mathbb{E}(N)\}^2}\left[\mathbb{E}\left\{\mathfrak{w}_{I,a,a}(\mathbf{Y}^o)|\mathbf{X}^o, M, \boldsymbol{C}, N, A=a\right\} - \mathbb{E}\left\{\mathfrak{w}_{I,a,a}(\mathbf{Y}^o)|\boldsymbol{C}, N, A=a\right\}\right] \\
&+ \frac{\mathbb{P}(A=1-a|M,\boldsymbol{C},N)N}{\pi^{1-a}(1-\pi)^{a}\{\mathbb{E}(N)\}^2}\left[\mathbb{E}\left\{\mathfrak{w}_{I,a,1-a}(\mathbf{Y}^o)|\mathbf{X}^o, M, \boldsymbol{C}, N, A=1-a\right\}\right. \\
&\qquad\qquad\left. - \mathbb{E}\left\{\mathfrak{w}_{I,a,1-a}(\mathbf{Y}^o)|\boldsymbol{C}, N, A=1-a\right\}\right] \\
&+ \frac{N}{\{\mathbb{E}(N)\}^2}\mathbb{E}\left\{\mathfrak{w}_{I,a,a}(\mathbf{Y}^o)|\boldsymbol{C}, N, A=a\right\} + \frac{N}{\{\mathbb{E}(N)\}^2}\mathbb{E}\left\{\mathfrak{w}_{I,a,1-a}(\mathbf{Y}^o)|\boldsymbol{C}, N, A=1-a\right\} \\
&- \frac{2N\lambda_{I,a}}{\mathbb{E}(N)},
\end{aligned}$$

*where* $\mathfrak{w}_{I,a,a}(\mathbf{y}) = \mathbb{E}\{N_k\overline{w}(\mathbf{y}, \mathbf{Y}_k^o)|A_k = 1-a\}$ *and* $\mathfrak{w}_{I,a,1-a}(\mathbf{y}) = \mathbb{E}\{N_k\overline{w}(\mathbf{Y}_k^o, \mathbf{y})|A_k = a\}$.

With full enrollment, i.e., $M(a) = M(1-a) = N$, Theorem S2 includes the EIF in Theorem 2 in the main article as a special case.

### S8.2.3 The triply robust estimators

Estimators with improved efficiency and satisfactory robustness can be motivated by the EIFs. To begin, we define the following nuisance functions

$$
\begin{aligned}
\zeta_{ik,a}^{\mathrm{m1}} &= \zeta_a^{\mathrm{m1}}(\mathbf{X}_i^o, \mathbf{X}_k^o, M_i, M_k, \boldsymbol{C}_i, \boldsymbol{C}_k, N_i, N_k) \\
&= \mathbb{E}\left\{\overline{w}(\mathbf{Y}_i^o, \mathbf{Y}_k^o) | \mathbf{X}_i^o, \mathbf{X}_k^o, M_i, M_k, \boldsymbol{C}_i, \boldsymbol{C}_k, N_i, N_k, A_i = a, A_k = 1-a\right\}, \\
\zeta_{ik,a}^{\mathrm{m2}} &= \zeta_a^{\mathrm{m2}}(\boldsymbol{C}_i, \boldsymbol{C}_k, N_i, N_k) = \mathbb{E}\left\{\overline{w}(\mathbf{Y}_i^o, \mathbf{Y}_k^o) | \boldsymbol{C}_i, \boldsymbol{C}_k, N_i, N_k, A_i = a, A_k = 1-a\right\}, \\
\zeta_{i,a}^{\mathrm{p}} &= \zeta_a^{\mathrm{p}}(M_i, \boldsymbol{C}_i, N_i) = \mathbb{P}(A_i = a | M_i, \boldsymbol{C}_i, N_i),
\end{aligned}
$$

where $\zeta_{ik,a}^{\mathrm{m1}}$ is the (first-level) expected observed average contrast between clusters $i$ and $k$ with cluster $i$ under treatment $a$ and cluster $k$ under $1-a$, conditional on observed individual- and cluster-level covariates as well as observed and original cluster sizes; $\zeta_{ik,a}^{\mathrm{m2}}$ is the (second-level) expected observed average contrast conditional on cluster-level covariates and original cluster sizes; and $\zeta_{i,a}^{\mathrm{p}}$ is the propensity score (conditional probability) of cluster $i$ receiving treatment $a$ given the observed and original cluster sizes as well as the cluster-level covariates.

We can consider parametric working models for $\boldsymbol{\zeta}_a = (\zeta_a^{\mathrm{m1}}, \zeta_a^{\mathrm{m2}}, \zeta_a^{\mathrm{p}})$. That is, $\zeta_a^{\mathrm{m1}} = \zeta_a^{\mathrm{m1}}(\boldsymbol{\vartheta}_a^{\mathrm{m1}})$, $\zeta_a^{\mathrm{m2}} = \zeta_a^{\mathrm{m2}}(\boldsymbol{\vartheta}_a^{\mathrm{m2}})$, and $\zeta_a^{\mathrm{p}} = \zeta_a^{\mathrm{p}}(\boldsymbol{\vartheta}_a^{\mathrm{p}})$, where $\zeta_a^{\mathrm{m1}}$, $\zeta_a^{\mathrm{m2}}$, and $\zeta_a^{\mathrm{p}}$ are prespecified functions with corresponding finite-dimensional parameters $\boldsymbol{\vartheta}_a^{\mathrm{m1}}$, $\boldsymbol{\vartheta}_a^{\mathrm{m2}}$, and $\boldsymbol{\vartheta}_a^{\mathrm{p}}$. Define estimated nuisance functions $\widehat{\boldsymbol{\zeta}}_a = (\widehat{\zeta}_a^{\mathrm{m1}}, \widehat{\zeta}_a^{\mathrm{m2}}, \widehat{\zeta}_a^{\mathrm{p}})$ and true nuisance functions $\boldsymbol{\zeta}_a^0 = (\zeta_a^{\mathrm{m1},0}, \zeta_a^{\mathrm{m2},0}, \zeta_a^{\mathrm{p},0})$. In this case, $(\widehat{\zeta}_a^{\mathrm{m1}}, \widehat{\zeta}_a^{\mathrm{m2}}, \widehat{\zeta}_a^{\mathrm{p}}) = \{\zeta_a^{\mathrm{m1}}(\widehat{\boldsymbol{\vartheta}}_a^{\mathrm{m1}}), \zeta_a^{\mathrm{m2}}(\widehat{\boldsymbol{\vartheta}}_a^{\mathrm{m2}}), \zeta_a^{\mathrm{p}}(\widehat{\boldsymbol{\vartheta}}_a^{\mathrm{p}})\}$. The EIFs in Theorem S2 motivate the following U-estimating equations:

$$
\sum_{1 \le i < k \le m} \boldsymbol{\psi}_v^{\mathrm{eff}}(\mathcal{O}_i, \mathcal{O}_k; \widehat{\boldsymbol{\vartheta}}, \boldsymbol{\lambda}) = \sum_{1 \le i < k \le m} \left\{ \begin{array}{c} \psi_{v,1}^{\mathrm{eff}}(\mathcal{O}_i, \mathcal{O}_k; \widehat{\boldsymbol{\vartheta}}, \lambda_1) \\ \psi_{v,0}^{\mathrm{eff}}(\mathcal{O}_i, \mathcal{O}_k; \widehat{\boldsymbol{\vartheta}}, \lambda_0) \end{array} \right\} = \mathbf{0}, \tag{S15}
$$

where $v = C, I$. For $a = 0, 1$,

$$
\begin{aligned}
\psi_{C,a}^{\mathrm{eff}}(\mathcal{O}_i, \mathcal{O}_k; \widehat{\boldsymbol{\vartheta}}, \lambda_a) = 2^{-1} \Bigg[ & \frac{\mathbb{1}(A_i = a)\mathbb{1}(A_k = 1-a)}{\pi(1-\pi)} \left\{\overline{w}(\mathbf{Y}_i^o, \mathbf{Y}_k^o) - \zeta_{ik,a}^{\mathrm{m1}}(\widehat{\boldsymbol{\vartheta}}_a^{\mathrm{m1}})\right\} \\
&+ \frac{\mathbb{1}(A_k = a)\mathbb{1}(A_i = 1-a)}{\pi(1-\pi)} \left\{\overline{w}(\mathbf{Y}_k^o, \mathbf{Y}_i^o) - \zeta_{ki,a}^{\mathrm{m1}}(\widehat{\boldsymbol{\vartheta}}_a^{\mathrm{m1}})\right\} + \frac{\zeta_{i,a}^{\mathrm{p}}(\widehat{\boldsymbol{\vartheta}}_a^{\mathrm{p}})\zeta_{k,1-a}^{\mathrm{p}}(\widehat{\boldsymbol{\vartheta}}_{1-a}^{\mathrm{p}})}{\pi(1-\pi)} \left\{\zeta_{ik,a}^{\mathrm{m1}}(\widehat{\boldsymbol{\vartheta}}_a^{\mathrm{m1}}) - \zeta_{ik,a}^{\mathrm{m2}}(\widehat{\boldsymbol{\vartheta}}_a^{\mathrm{m2}})\right\} \\
&+ \frac{\zeta_{i,1-a}^{\mathrm{p}}(\widehat{\boldsymbol{\vartheta}}_{1-a}^{\mathrm{p}})\zeta_{k,a}^{\mathrm{p}}(\widehat{\boldsymbol{\vartheta}}_a^{\mathrm{p}})}{\pi(1-\pi)} \left\{\zeta_{ki,a}^{\mathrm{m1}}(\widehat{\boldsymbol{\vartheta}}_a^{\mathrm{m1}}) - \zeta_{ki,a}^{\mathrm{m2}}(\widehat{\boldsymbol{\vartheta}}_a^{\mathrm{m2}})\right\} + \zeta_{ik,a}^{\mathrm{m2}}(\widehat{\boldsymbol{\vartheta}}_a^{\mathrm{m2}}) + \zeta_{ki,a}^{\mathrm{m2}}(\widehat{\boldsymbol{\vartheta}}_a^{\mathrm{m2}}) - 2\lambda_a \Bigg]
\end{aligned}
$$

and $\boldsymbol{\psi}_I^{\mathrm{eff}}(\mathcal{O}_i, \mathcal{O}_k; \widehat{\boldsymbol{\vartheta}}, \boldsymbol{\lambda}) = N_i N_k \boldsymbol{\psi}_C^{\mathrm{eff}}(\mathcal{O}_i, \mathcal{O}_k; \widehat{\boldsymbol{\vartheta}}, \boldsymbol{\lambda})$. Solving (S15) leads to estimators $\widehat{\lambda}_{v,a}^{\mathrm{tr}}$ and $\widehat{\Lambda}_v^{\mathrm{tr}} = f(\widehat{\lambda}_{v,1}^{\mathrm{tr}}, \widehat{\lambda}_{v,0}^{\mathrm{tr}})$. Let $(\underline{\boldsymbol{\vartheta}}_a^{\mathrm{m1}}, \underline{\boldsymbol{\vartheta}}_a^{\mathrm{m2}}, \underline{\boldsymbol{\vartheta}}_a^{\mathrm{p}})$ denote the probability limit of $(\widehat{\boldsymbol{\vartheta}}_a^{\mathrm{m1}}, \widehat{\boldsymbol{\vartheta}}_a^{\mathrm{m2}}, \widehat{\boldsymbol{\vartheta}}_a^{\mathrm{p}})$, respectively. We have the following theorem, which summarizes the properties of these estimators.

**Theorem S3.** *Under Assumptions 1-3 in the main article and Assumption S1, for $v = C, I$, if (i) $\zeta_a^{\mathrm{p}}(\underline{\boldsymbol{\vartheta}}_a^{\mathrm{p}}) = \zeta_a^{\mathrm{p},0}$ or (ii) $\mathbb{E}\{\zeta_a^{\mathrm{m1}}(\underline{\boldsymbol{\vartheta}}_a^{\mathrm{m1}}) | M_i, M_k, N_i, N_k, \boldsymbol{C}_i, \boldsymbol{C}_k\} = \zeta_a^{\mathrm{m2}}(\underline{\boldsymbol{\vartheta}}_a^{\mathrm{m2}})$, and regularity conditions (P1)-(P4) listed in Section S1 hold, then $\widehat{\boldsymbol{\lambda}}_v^{\mathrm{tr}} \xrightarrow{p} \boldsymbol{\lambda}_v$; furthermore, if regularity conditions (P5)-(P7) also hold, then $m^{1/2}(\widehat{\boldsymbol{\lambda}}_v^{\mathrm{tr}} - \boldsymbol{\lambda}_v) \xrightarrow{d} \mathcal{N}(\mathbf{0}, \boldsymbol{V}_v^{\mathrm{tr}})$ and $\widehat{\boldsymbol{V}}_v^{\mathrm{tr}} \xrightarrow{p} \boldsymbol{V}_v^{\mathrm{tr}}$; moreover, if (i) and (ii) are both satisfied, then $\widehat{\boldsymbol{V}}_v^{\mathrm{tr}}$ converges in probability to the semiparametric efficiency lower bound of $\boldsymbol{\lambda}_v$.*

Theorem S3 states that $\widehat{\lambda}^{\mathrm{tr}}_{v,a}$ is triply robust in the sense that it is consistent and asymptotically normal if $\zeta^{\mathrm{p}}_a(\underline{\boldsymbol{\vartheta}}^{\mathrm{p}}_a)$ correctly specifies $\zeta^{\mathrm{p},0}_a$ or $\zeta^{\mathrm{m1}}_a(\underline{\boldsymbol{\vartheta}}^{\mathrm{m1}}_a)$ and $\zeta^{\mathrm{m2}}_a(\underline{\boldsymbol{\vartheta}}^{\mathrm{m2}}_a)$ are compatible conditional on $(M_i, M_k, N_i, N_k, \boldsymbol{C}_i, \boldsymbol{C}_k)$. Similar to the model-robust estimator in the main article, the estimating function $\psi^{\mathrm{eff}}_{v,a}(\mathcal{O}_i, \mathcal{O}_k; \widehat{\boldsymbol{\vartheta}}, \lambda_a)$ is the efficient score because $\boldsymbol{V}^{\mathrm{tr}}_v$, the asymptotic variance of $m^{1/2}\widehat{\boldsymbol{\lambda}}^{\mathrm{tr}}_v$, attains the semiparametric efficiency lower bound of $\boldsymbol{\lambda}_v$ if all parametric working models correctly specify their respective nuisance functions. For $\widehat{\Lambda}^{\mathrm{tr}}_v$, Theorem S3 implies that, for $v = C, I$, $(\widehat{V}^{\mathrm{tr}}_v)^{-1/2}(\widehat{\Lambda}^{\mathrm{tr}}_v - \Lambda_v) \xrightarrow{d} \mathcal{N}(0,1)$, and, if (i) and (ii) in Theorem S3 are both satisfied, then $\widehat{V}^{\mathrm{tr}}_v$ converges in probability to the semiparametric efficiency lower bound of $\Lambda_v$.

As we discussed in Section 3.3 of the main article, the triply robust estimator can also be viewed as a U-statistic analog to the augmented inverse probability-weighted (AIPW) estimator for the ATE. Because of the within-cluster subsampling, a total of eight conditional expectations need to be imputed, which are summarized in Web Table S3.

Web Table S3: The conditional expectations to be imputed when implementing the model-robust and triply robust estimators for the GCE estimand. Here, the combination of treatment $a$ and observation $i$ means that the observation $i$ is in the winning position and under treatment $a$.

| | | Within-cluster subsampling | |
|---|---|---|---|
| Treatment | Obs. | No | Yes |
| $a$ | $i$ | $\mathbb{E}\left\{\overline{w}(\mathbf{Y}_i,\mathbf{Y}_k) \mid \begin{array}{l} A_i=a,\mathbf{X}_i,\boldsymbol{C}_i,N_i \\ A_k=1-a,\mathbf{X}_k,\boldsymbol{C}_k,N_k \end{array}\right\}$ | $\mathbb{E}\left\{\overline{w}(\mathbf{Y}_i,\mathbf{Y}_k) \mid \begin{array}{l} A_i=a,\mathbf{X}_i,M_i,\boldsymbol{C}_i,N_i \\ A_k=1-a,\mathbf{X}_k,M_i,\boldsymbol{C}_k,N_k \end{array}\right\}$ |
| | | – | $\mathbb{E}\left\{\overline{w}(\mathbf{Y}_i,\mathbf{Y}_k) \mid \begin{array}{l} A_i=a,\boldsymbol{C}_i,N_i \\ A_k=1-a,\boldsymbol{C}_k,N_k \end{array}\right\}$ |
| | $k$ | $\mathbb{E}\left\{\overline{w}(\mathbf{Y}_k,\mathbf{Y}_i) \mid \begin{array}{l} A_k=a,\mathbf{X}_k,\boldsymbol{C}_k,N_k \\ A_i=1-a,\mathbf{X}_i,\boldsymbol{C}_i,N_i \end{array}\right\}$ | $\mathbb{E}\left\{\overline{w}(\mathbf{Y}_k,\mathbf{Y}_i) \mid \begin{array}{l} A_k=a,\mathbf{X}_k,M_k,\boldsymbol{C}_k,N_k \\ A_i=1-a,\mathbf{X}_i,M_i,\boldsymbol{C}_i,N_i \end{array}\right\}$ |
| | | – | $\mathbb{E}\left\{\overline{w}(\mathbf{Y}_k,\mathbf{Y}_i) \mid \begin{array}{l} A_k=a,\boldsymbol{C}_k,N_k \\ A_i=1-a,\boldsymbol{C}_i,N_i \end{array}\right\}$ |
| $1-a$ | $i$ | $\mathbb{E}\left\{\overline{w}(\mathbf{Y}_i,\mathbf{Y}_k) \mid \begin{array}{l} A_i=1-a,\mathbf{X}_i,\boldsymbol{C}_i,N_i \\ A_k=a,\mathbf{X}_k,\boldsymbol{C}_k,N_k \end{array}\right\}$ | $\mathbb{E}\left\{\overline{w}(\mathbf{Y}_i,\mathbf{Y}_k) \mid \begin{array}{l} A_i=1-a,\mathbf{X}_i,M_i,\boldsymbol{C}_i,N_i \\ A_k=a,\mathbf{X}_k,M_i,\boldsymbol{C}_k,N_k \end{array}\right\}$ |
| | | – | $\mathbb{E}\left\{\overline{w}(\mathbf{Y}_i,\mathbf{Y}_k) \mid \begin{array}{l} A_i=1-a,\boldsymbol{C}_i,N_i \\ A_k=a,\boldsymbol{C}_k,N_k \end{array}\right\}$ |
| | $k$ | $\mathbb{E}\left\{\overline{w}(\mathbf{Y}_k,\mathbf{Y}_i) \mid \begin{array}{l} A_k=1-a,\mathbf{X}_k,\boldsymbol{C}_k,N_k \\ A_i=a,\mathbf{X}_i,\boldsymbol{C}_i,N_i \end{array}\right\}$ | $\mathbb{E}\left\{\overline{w}(\mathbf{Y}_k,\mathbf{Y}_i) \mid \begin{array}{l} A_k=1-a,\mathbf{X}_k,M_k,\boldsymbol{C}_k,N_k \\ A_i=a,\mathbf{X}_i,M_i,\boldsymbol{C}_i,N_i \end{array}\right\}$ |
| | | – | $\mathbb{E}\left\{\overline{w}(\mathbf{Y}_k,\mathbf{Y}_i) \mid \begin{array}{l} A_k=1-a,\boldsymbol{C}_k,N_k \\ A_i=a,\boldsymbol{C}_i,N_i \end{array}\right\}$ |

### S8.2.4 Debiased machine learning estimators

We use the same sample-splitting scheme given in Section 3.4 of the main article. With the EIFs, we obtain the following estimating equations for the DML estimators:

$$\sum_{p=1}^{|\mathfrak{I}^{\mathrm{pr}}|} \sum_{(i,k)\in\mathcal{I}^{\mathrm{pr}}_p} \boldsymbol{\psi}^{\mathrm{eff}}_v(\mathcal{O}_i, \mathcal{O}_k; \widehat{\boldsymbol{\zeta}}_p, \boldsymbol{\lambda}) = \sum_{p=1}^{|\mathfrak{I}^{\mathrm{pr}}|} \sum_{(i,k)\in\mathcal{I}^{\mathrm{pr}}_p} \left\{ \begin{array}{c} \psi^{\mathrm{eff}}_{v,1}(\mathcal{O}_i, \mathcal{O}_k; \widehat{\boldsymbol{\zeta}}_p, \lambda_1) \\ \psi^{\mathrm{eff}}_{v,0}(\mathcal{O}_i, \mathcal{O}_k; \widehat{\boldsymbol{\zeta}}_p, \lambda_0) \end{array} \right\} = \mathbf{0}, \tag{S16}$$

for $v = C, I$. For $a = 0, 1$,

$$\psi^{\text{eff}}_{C,a}(\mathcal{O}_i, \mathcal{O}_k; \widehat{\boldsymbol{\zeta}}_p, \lambda_a) = 2^{-1}\Bigg[\frac{\mathbb{1}(A_i = a)\mathbb{1}(A_k = 1-a)}{\pi(1-\pi)}\left\{\overline{w}(\mathbf{Y}^o_i, \mathbf{Y}^o_k) - \widehat{\zeta}^{\text{m1}}_{ik,p,a}\right\}$$
$$+ \frac{\mathbb{1}(A_k = a)\mathbb{1}(A_i = 1-a)}{\pi(1-\pi)}\left\{\overline{w}(\mathbf{Y}^o_k, \mathbf{Y}^o_i) - \widehat{\zeta}^{\text{m1}}_{ki,p,a}\right\} + \frac{\widehat{\zeta}^{\text{p}}_{i,p,a}\widehat{\zeta}^{\text{p}}_{k,p,1-a}}{\pi(1-\pi)}\left(\widehat{\zeta}^{\text{m1}}_{ik,p,a} - \widehat{\zeta}^{\text{m2}}_{ik,p,a}\right)$$
$$+ \frac{\widehat{\zeta}^{\text{p}}_{i,p,1-a}\widehat{\zeta}^{\text{p}}_{k,p,a}}{\pi(1-\pi)}\left(\widehat{\zeta}^{\text{m1}}_{ki,p,a} - \widehat{\zeta}^{\text{m2}}_{ki,p,a}\right) + \widehat{\zeta}^{\text{m2}}_{ik,p,a} + \widehat{\zeta}^{\text{m2}}_{ki,p,a} - 2\lambda_a\Bigg]$$

and $\boldsymbol{\psi}^{\text{eff}}_I(\mathcal{O}_i, \mathcal{O}_k; \widehat{\boldsymbol{\zeta}}_p, \boldsymbol{\lambda}) = N_i N_k \boldsymbol{\psi}^{\text{eff}}_C(\mathcal{O}_i, \mathcal{O}_k; \widehat{\boldsymbol{\zeta}}_p, \boldsymbol{\lambda})$. For a given partition $\mathfrak{I}^{\text{pr}}$, we form intermediate estimating equations using observations in each $\mathcal{I}^{\text{pr}}_p$ with $\widehat{\boldsymbol{\zeta}}_{p,a}$ estimated using observations in $(\mathcal{I}^{\text{pr}}_p)^c$, comprised of clusters not in $\mathcal{I}^{\text{pr}}_p$. Solving (S16) leads to the DML estimators $\widehat{\lambda}^{\text{dml}}_{v,a}$ and $\widehat{\Lambda}^{\text{dml}}_v = f(\widehat{\lambda}^{\text{dml}}_{v,1}, \widehat{\lambda}^{\text{dml}}_{v,0})$. Let $\widehat{\boldsymbol{V}}^{\text{dml}}_v = (\widehat{\boldsymbol{B}}^{\text{dml}}_v)^{-1}\widehat{\boldsymbol{\Sigma}}^{\text{dml}}_v\{(\widehat{\boldsymbol{B}}^{\text{dml}}_v)^{-1}\}^\top$ and $\widehat{V}^{\text{dml}}_v = \{\nabla_{\boldsymbol{\lambda}} f(\widehat{\boldsymbol{\lambda}}^{\text{dml}}_v)\}^\top \widehat{\boldsymbol{V}}^{\text{dml}}_v \times \nabla_{\boldsymbol{\lambda}} f(\widehat{\boldsymbol{\lambda}}^{\text{dml}}_v)$, where

$$\widehat{\boldsymbol{B}}^{\text{dml}}_v = \binom{m}{2}^{-1}\sum_{p=1}^{|\mathfrak{I}^{\text{pr}}|}\sum_{(i,k)\in\mathcal{I}^{\text{pr}}_p}\nabla_\lambda \boldsymbol{\psi}^{\text{eff}}_v(\mathcal{O}_i, \mathcal{O}_k; \widehat{\boldsymbol{\zeta}}_p, \widehat{\boldsymbol{\lambda}}^{\text{dml}}_v),$$
$$\widehat{\boldsymbol{\Sigma}}^{\text{dml}}_v = \frac{4}{m-1}\sum_{i=1}^{m}\widehat{\boldsymbol{\psi}}^{\text{eff}}_v(\mathcal{O}_i; \widehat{\boldsymbol{\zeta}}, \widehat{\boldsymbol{\lambda}}^{\text{dml}}_v)\widehat{\boldsymbol{\psi}}^{\text{eff}}_v(\mathcal{O}_i; \widehat{\boldsymbol{\zeta}}, \widehat{\boldsymbol{\lambda}}^{\text{dml}}_v)^\top,$$

with

$$\widehat{\boldsymbol{\psi}}^{\text{eff}}_v(\mathcal{O}_i; \widehat{\boldsymbol{\zeta}}, \widehat{\boldsymbol{\lambda}}^{\text{dml}}_v) = \frac{1}{m-1}\sum_{k:k\neq i}\sum_{p=1}^{|\mathfrak{I}^{\text{pr}}|}\mathbb{1}\{(i,k)\in\mathcal{I}^{\text{pr}}_p\}\boldsymbol{\psi}^{\text{eff}}_v(\mathcal{O}_i, \mathcal{O}_k; \widehat{\boldsymbol{\zeta}}_p, \widehat{\boldsymbol{\lambda}}^{\text{dml}}_v).$$

Here, $\widehat{\boldsymbol{V}}^{\text{dml}}_v$ and $\widehat{V}^{\text{dml}}_v$ are analytical variance estimators under the same sample-splitting scheme used to estimate $\widehat{\boldsymbol{\lambda}}^{\text{dml}}_v$. The structure of the estimated Hájek projection function $\widehat{\boldsymbol{\psi}}^{\text{eff}}_v(\mathcal{O}_i; \widehat{\boldsymbol{\zeta}}, \widehat{\boldsymbol{\lambda}}^{\text{dml}})$ allows us to locate the partition membership $\mathcal{I}^{\text{pr}}_p$ for each $(i, k)$ and plug in the corresponding estimated nuisance function $\widehat{\boldsymbol{\zeta}}_p$. We have the following theorem, which summarizes the properties of the DML estimators.

**Theorem S4.** *Under Assumptions 1-3 in the main article and Assumption S1, for $v = C, I$, if regularity conditions (C1)-(C5) listed in Section S5 hold, then $\widehat{\boldsymbol{\lambda}}^{\text{dml}}_v \xrightarrow{p} \boldsymbol{\lambda}_v$; furthermore, if regularity conditions (A1)-(A5) also hold, then $m^{1/2}(\widehat{\boldsymbol{\lambda}}^{\text{dml}}_v - \boldsymbol{\lambda}_v) \xrightarrow{d} \mathcal{N}(\mathbf{0}, \boldsymbol{V}^{\text{dml}}_v)$; moreover, if (V1) also holds, then $\widehat{\boldsymbol{V}}^{\text{dml}}_v \xrightarrow{p} \boldsymbol{V}^{\text{dml}}_v$, where $\boldsymbol{V}^{\text{dml}}_v$ is the semiparametric efficiency lower bounds of $\boldsymbol{\lambda}_v$.*

For $\widehat{\Lambda}^{\text{dml}}_v$, Theorem S4 implies that, for $v = C, I$, $(\widehat{V}^{\text{dml}}_v)^{-1/2}(\widehat{\Lambda}^{\text{dml}}_v - \Lambda_v) \xrightarrow{d} \mathcal{N}(0, 1)$, and $\widehat{V}^{\text{dml}}_v$ converge in probability to the semiparametric efficiency lower bounds of $\Lambda_v$.

### S8.3 Proofs of theoretical results

We first prove Theorem S1, and then derive the EIFs in Theorem S2. Lastly, we prove Theorem S3. The proof of Theorem S4 closely follows that of Theorem 4 in the main article, and is thus omitted.

#### S8.3.1 Intermediary theoretical results

**Lemma S2.** *Under Assumptions 1-3 in the main article and Assumption S1, (i)* $\mathbf{X} \perp (A, M)|(N, \boldsymbol{C})$*, (ii)* $(A, \mathbf{X}, \mathbf{Y}, \boldsymbol{C}) \perp \boldsymbol{S}|(M, N)$*, and (iii)* $\mathbf{X} \perp \boldsymbol{S} \perp A|(M, N, \boldsymbol{C})$*.*

Lemma S2 is from Lemma 1 of Wang et al. (2024, Supplementary Material), and the proof is thus omitted.

**Lemma S3.** *Define the following notations,*

$$\overline{w}\{\mathbf{Y}_i(a), \mathbf{Y}_k(a')\} = \sum_{j=1}^{N_i}\sum_{l=1}^{N_k} \frac{w\{\mathbf{Y}_{ij}(a), \mathbf{Y}_{kl}(a')\}}{N_i N_k}, \quad \overline{w}(\mathbf{Y}_i, \mathbf{Y}_k) = \sum_{j=1}^{N_i}\sum_{l=1}^{N_k} \frac{w\{\mathbf{Y}_{ij}(A_i), \mathbf{Y}_{kl}(A_k)\}}{N_i N_k},$$

$$\overline{w}\{\mathbf{Y}_i^o(a), \mathbf{Y}_k^o(a')\} = \sum_{j=1}^{N_i}\sum_{l=1}^{N_k} \frac{S_{ij}(a)S_{kl}(a')w\{\mathbf{Y}_{ij}(a), \mathbf{Y}_{kl}(a')\}}{M_i(a)M_k(a')},$$

$$\overline{w}(\mathbf{Y}_i^o, \mathbf{Y}_k^o) = \sum_{j=1}^{N_i}\sum_{l=1}^{N_k} \frac{S_{ij}(A_i)S_{kl}(A_k)w\{\mathbf{Y}_{ij}(A_i), \mathbf{Y}_{kl}(A_k)\}}{M_i(A_i)M_k(A_k)}.$$

*Under Assumptions 1-3 in the main article and Assumption S1, we have the conditional expectations of the above quantities being equivalent given the treatment assignments, cluster sizes, and cluster-level covariates, i.e.,*

$$\begin{aligned}
&\mathbb{E}\left[\overline{w}\{\mathbf{Y}_i(a), \mathbf{Y}_k(a')\}\big|N_i, N_k, \boldsymbol{C}_i, \boldsymbol{C}_k\right] = \mathbb{E}\left[\overline{w}\{\mathbf{Y}_i^o(a), \mathbf{Y}_k^o(a')\}\big|N_i, N_k, \boldsymbol{C}_i, \boldsymbol{C}_k\right] \\
&= \mathbb{E}\left\{\overline{w}(\mathbf{Y}_i, \mathbf{Y}_k)\big|A_i = a, A_k = a', N_i, N_k, \boldsymbol{C}_i, \boldsymbol{C}_k\right\} = \mathbb{E}\left\{\overline{w}(\mathbf{Y}_i^o, \mathbf{Y}_k^o)\big|A_i = a, A_k = a', M_i, M_k, N_i, N_k, \boldsymbol{C}_i, \boldsymbol{C}_k\right\}.
\end{aligned}$$

*Proof of Lemma S3.* We first prove

$$\mathbb{E}\left[\overline{w}\{\mathbf{Y}_i(a), \mathbf{Y}_k(a')\}\big|N_i, N_k, \boldsymbol{C}_i, \boldsymbol{C}_k\right] = \mathbb{E}\left[\overline{w}\{\mathbf{Y}_i^o(a), \mathbf{Y}_k^o(a')\}\big|N_i, N_k, \boldsymbol{C}_i, \boldsymbol{C}_k\right].$$

Assumption S1 implies that for each $j = 1, \ldots, N_i$ and $l = 1, \ldots, N_k$,

$$\mathbb{P}\{S_{ij}(a) = 1|\mathbf{Y}_i(a), \mathbf{X}_i, M_i(a), N_i, \boldsymbol{C}_i\} = \frac{\binom{N_i - 1}{M_i(a) - 1}}{\binom{N_i}{M_i(a)}} = \frac{M_i(a)}{N_i},$$

$$\mathbb{P}\{S_{kl}(a) = 1|\mathbf{Y}_k(a), \mathbf{X}_k, M_k(a), N_k, \boldsymbol{C}_k\} = \frac{\binom{N_k - 1}{M_k(a) - 1}}{\binom{N_k}{M_k(a)}} = \frac{M_k(a)}{N_k}.$$

Therefore, for $a, a' \in \{0, 1\}$,

$$\begin{aligned}
&\mathbb{E}\left[\overline{w}\{\mathbf{Y}_i^o(a), \mathbf{Y}_k^o(a')\}|N_i, N_k, \boldsymbol{C}_i, \boldsymbol{C}_k\right] \\
&= \mathbb{E}\left(\mathbb{E}\left[\sum_{j=1}^{N_i}\sum_{l=1}^{N_k} \frac{S_{ij}(a)S_{kl}(a')w\{\mathbf{Y}_{ij}(a), \mathbf{Y}_{kl}(a')\}}{M_i(a)M_k(a')} \middle| \begin{array}{l} \mathbf{Y}_i(a), \mathbf{X}_i, M_i(a), N_i, \boldsymbol{C}_i, \\ \mathbf{Y}_k(a), \mathbf{X}_k, M_k(a), N_k, \boldsymbol{C}_k \end{array}\right] \middle| \begin{array}{l} N_i, \boldsymbol{C}_i, \\ N_k, \boldsymbol{C}_k \end{array}\right) \\
&= \mathbb{E}\left[\sum_{j=1}^{N_i}\sum_{l=1}^{N_k} \mathbb{E}\left\{S_{ij}(a)S_{kl}(a') \middle| \begin{array}{l} \mathbf{Y}_i(a), \mathbf{X}_i, M_i(a), N_i, \boldsymbol{C}_i, \\ \mathbf{Y}_k(a), \mathbf{X}_k, M_k(a), N_k, \boldsymbol{C}_k \end{array}\right\} \frac{w\{\mathbf{Y}_{ij}(a), \mathbf{Y}_{kl}(a')\}}{M_i(a)M_k(a')} \middle| \begin{array}{l} N_i, \boldsymbol{C}_i, \\ N_k, \boldsymbol{C}_k \end{array}\right]
\end{aligned}$$

$$
\begin{aligned}
&= \mathbb{E}\left[\sum_{j=1}^{N_i}\sum_{l=1}^{N_k}\frac{w\{\mathbf{Y}_{ij}(a),\mathbf{Y}_{kl}(a')\}}{N_iN_k}\middle| N_i, N_k, \boldsymbol{C}_i, \boldsymbol{C}_k\right] \\
&= \mathbb{E}\left[\overline{w}\{\mathbf{Y}_i(a),\mathbf{Y}_k(a')\}\middle| N_i, N_k, \boldsymbol{C}_i, \boldsymbol{C}_k\right].
\end{aligned}
$$

Next, since $A \perp \mathcal{D}$ and $\overline{w}\{\mathbf{Y}_i^o(a),\mathbf{Y}_k^o(a')\}$ is a function of $(\mathcal{D}_i,\mathcal{D}_k)$, then

$$
\begin{aligned}
&\mathbb{E}\left\{\overline{w}(\mathbf{Y}_i^o,\mathbf{Y}_k^o)\middle| A_i = a, A_k = a', N_i, N_k, \boldsymbol{C}_i, \boldsymbol{C}_k\right\} \\
&= \mathbb{E}\left[aa'\overline{w}\{\mathbf{Y}_i^o(1),\mathbf{Y}_k^o(1)\}\middle| A_i = a, A_k = a', N_i, N_k, \boldsymbol{C}_i, \boldsymbol{C}_k\right] \\
&\quad + \mathbb{E}\left[a(1-a')\overline{w}\{\mathbf{Y}_i^o(1),\mathbf{Y}_k^o(0)\}\middle| A_i = a, A_k = a', N_i, N_k, \boldsymbol{C}_i, \boldsymbol{C}_k\right] \\
&\quad + \mathbb{E}\left[(1-a)a'\overline{w}\{\mathbf{Y}_i^o(0),\mathbf{Y}_k^o(1)\}\middle| A_i = a, A_k = a', N_i, N_k, \boldsymbol{C}_i, \boldsymbol{C}_k\right] \\
&\quad + \mathbb{E}\left[(1-a)(1-a')\overline{w}\{\mathbf{Y}_i^o(0),\mathbf{Y}_k^o(0)\}\middle| A_i = a, A_k = a', N_i, N_k, \boldsymbol{C}_i, \boldsymbol{C}_k\right] \\
&= \mathbb{E}\left[\overline{w}\{\mathbf{Y}_i^o(a),\mathbf{Y}_k^o(a')\}\middle| A_i = a, A_k = a', N_i, N_k, \boldsymbol{C}_i, \boldsymbol{C}_k\right],
\end{aligned}
$$

as desired. Finally, we prove

$$
\mathbb{E}\left[\overline{w}\{\mathbf{Y}_i(a),\mathbf{Y}_k(a')\}\middle| N_i, N_k, \boldsymbol{C}_i, \boldsymbol{C}_k\right] = \mathbb{E}\left\{\overline{w}(\mathbf{Y}_i^o,\mathbf{Y}_k^o)\middle| A_i = a, A_k = a', M_i, M_k, N_i, N_k, \boldsymbol{C}_i, \boldsymbol{C}_k\right\}.
$$

Assumption S1 implies that

$$
\mathbb{E}\left[\overline{w}\{\mathbf{Y}_i(a),\mathbf{Y}_k(a')\}\middle| N_i, N_k, \boldsymbol{C}_i, \boldsymbol{C}_k\right] = \mathbb{E}\left[\overline{w}\{\mathbf{Y}_i(a),\mathbf{Y}_k(a')\}\middle| M_i(a), M_k(a'), N_i, N_k, \boldsymbol{C}_i, \boldsymbol{C}_k\right].
$$

Again, using the conditional distribution of $(S_i(a), S_k(a'))$, we have

$$
\mathbb{E}\left[\overline{w}\{\mathbf{Y}_i(a),\mathbf{Y}_k(a')\}\middle| M_i(a), M_k(a'), N_i, N_k, \boldsymbol{C}_i, \boldsymbol{C}_k\right] = \mathbb{E}\left[\overline{w}\{\mathbf{Y}_i^o(a),\mathbf{Y}_k^o(a')\}\middle| M_i(a), M_k(a'), N_i, N_k, \boldsymbol{C}_i, \boldsymbol{C}_k\right].
$$

Since $A \perp \mathcal{D}$, we obtain

$$
\mathbb{E}\left[\overline{w}\{\mathbf{Y}_i^o(a),\mathbf{Y}_k^o(a')\}\middle| M_i(a), M_k(a'), N_i, N_k, \boldsymbol{C}_i, \boldsymbol{C}_k\right] = \mathbb{E}\left\{\overline{w}(\mathbf{Y}_i^o,\mathbf{Y}_k^o)\middle| A_i = a, A_k = a', M_i, M_k, N_i, N_k, \boldsymbol{C}_i, \boldsymbol{C}_k\right\},
$$

which completes the proof. □

### S8.3.2 The nonparametric estimators

*Proof of Theorem S1.* For the condition

$$
\mathbb{E}\left\{\sum_{1\le i<k\le m}\psi_{C,a}^{\mathrm{np}}(\mathcal{O}_i,\mathcal{O}_k;\lambda_a)\right\} = 0,
$$

we can write it as

$$
\mathbb{E}\left(\sum_{1\le i<k\le m} 2^{-1}\left[\frac{\mathbb{1}(A_i = a)\mathbb{1}(A_k = 1-a)}{M_iM_k}\sum_{j=1}^{N_i}\sum_{l=1}^{N_k} S_{ij}S_{kl}\left\{w(\boldsymbol{Y}_{ij},\boldsymbol{Y}_{kl}) - \lambda_a\right\}\right.\right.
$$

$$+\frac{\mathbb{1}(A_k=a)\mathbb{1}(A_i=1-a)}{M_iM_k}\sum_{j=1}^{N_i}\sum_{l=1}^{N_k}S_{ij}S_{kl}\left\{w(\mathbf{Y}_{kl},\mathbf{Y}_{ij})-\lambda_a\right\}\Bigg]\Bigg)=0,$$

which is rearranged into

$$\mathbb{E}\left\{\sum_{1\le i\ne k\le m}\frac{\mathbb{1}(A_i=a)\mathbb{1}(A_k=1-a)}{M_iM_k}\sum_{j=1}^{N_i}\sum_{l=1}^{N_k}S_{ij}S_{kl}w(\mathbf{Y}_{ij},\mathbf{Y}_{kl})\right\}=\lambda_a\mathbb{E}\left\{\sum_{1\le i\ne k\le m}\mathbb{1}(A_i=a)\mathbb{1}(A_k=1-a)\right\}.$$

Multiplied by $\{m(m-1)\}^{-1}$ on both sides and by Lemma S2, the left-hand side of the above equality is

$$\begin{aligned}
&\frac{1}{m(m-1)}\sum_{1\le i\ne k\le m}\mathbb{E}\left\{\mathbb{1}(A_i=a)\mathbb{1}(A_k=1-a)\sum_{j=1}^{N_i}\sum_{l=1}^{N_k}\frac{S_{ij}S_{kl}w(\mathbf{Y}_{ij},\mathbf{Y}_{kl})}{M_iM_k}\right\}\\
&=\frac{1}{m(m-1)}\sum_{1\le i\ne k\le m}\pi(1-\pi)\mathbb{E}\left[\sum_{j=1}^{N_i}\sum_{l=1}^{N_k}\frac{S_{ij}(a)S_{kl}(1-a)w\{\mathbf{Y}_{ij}(a),\mathbf{Y}_{kl}(1-a)\}}{M_i(a)M_k(1-a)}\right]\\
&=\pi(1-\pi)\mathbb{E}\left[\sum_{j=1}^{N_i}\sum_{l=1}^{N_k}\frac{S_{ij}(a)S_{kl}(1-a)w\{\mathbf{Y}_{ij}(a),\mathbf{Y}_{kl}(1-a)\}}{M_i(a)M_k(1-a)}\right]\\
&=\pi(1-\pi)\mathbb{E}\left(\mathbb{E}\left[\sum_{j=1}^{N_i}\sum_{l=1}^{N_k}\frac{S_{ij}(a)S_{kl}(1-a)w\{\mathbf{Y}_{ij}(a),\mathbf{Y}_{kl}(1-a)\}}{M_i(a)M_k(1-a)}\,\middle|\,\begin{array}{l}N_i,N_k,M_i(a),M_k(1-a),\\ \boldsymbol{C}_i,\boldsymbol{C}_k,\mathbf{Y}_i(a),\mathbf{Y}_k(1-a)\end{array}\right]\right)\\
&=\pi(1-\pi)\mathbb{E}\left[\sum_{j=1}^{N_i}\sum_{l=1}^{N_k}\frac{w\{\mathbf{Y}_{ij}(a),\mathbf{Y}_{kl}(1-a)\}}{M_i(a)M_k(1-a)}\mathbb{E}\{S_{ij}(a)|N_i,M_i(a),\boldsymbol{C}_i\}\mathbb{E}\{S_{kl}(1-a)|N_k,M_k(1-a),\boldsymbol{C}_k\}\right]\\
&=\pi(1-\pi)\mathbb{E}\left[\sum_{j=1}^{N_i}\sum_{l=1}^{N_k}\frac{w\{\mathbf{Y}_{ij}(a),\mathbf{Y}_{kl}(1-a)\}}{M_i(a)M_k(1-a)}\frac{M_i(a)}{N_i}\frac{M_k(1-a)}{N_k}\right]\\
&=\pi(1-\pi)\mathbb{E}\left[\sum_{j=1}^{N_i}\sum_{l=1}^{N_k}\frac{w\{\mathbf{Y}_{ij}(a),\mathbf{Y}_{kl}(1-a)\}}{N_iN_k}\right],
\end{aligned}$$

and the right-hand side is

$$\frac{1}{m(m-1)}\sum_{1\le i\ne k\le m}\mathbb{E}\{\mathbb{1}(A_i=a)\mathbb{1}(A_k=1-a)\}=\frac{1}{m(m-1)}\sum_{1\le i\ne k\le m}\pi(1-\pi)=\pi(1-\pi).$$

Thus, this gives us

$$\lambda_a=\lambda_{C,a}=\mathbb{E}\left[\sum_{j=1}^{N_i}\sum_{l=1}^{N_k}\frac{w\{\mathbf{Y}_{ij}(a),\mathbf{Y}_{kl}(1-a)\}}{N_iN_k}\right].$$

The asymptotic normality follows the same arguments in Section S2. For $\widehat{\boldsymbol{\lambda}}_I^{\text{np}}$ and $\widehat{\boldsymbol{V}}_I^{\text{np}}$, it suffices to investigate the condition

$$\mathbb{E}\left\{\sum_{1\le i<k\le m}\psi_{I,a}^{\text{np}}(\mathcal{O}_i,\mathcal{O}_k;\lambda_a)\right\}=0,$$

which can be written as

$$\mathbb{E}\left(\sum_{1\le i<k\le m}2^{-1}\left[\frac{\mathbb{1}(A_i=a)\mathbb{1}(A_k=1-a)N_iN_k}{M_iM_k}\sum_{j=1}^{N_i}\sum_{l=1}^{N_k}S_{ij}S_{kl}\left\{w(\mathbf{Y}_{ij},\mathbf{Y}_{kl})-\lambda_a\right\}\right.\right.$$
$$\left.\left.+\frac{\mathbb{1}(A_k=a)\mathbb{1}(A_i=1-a)N_iN_k}{M_iM_k}\sum_{j=1}^{N_i}\sum_{l=1}^{N_k}S_{ij}S_{kl}\left\{w(\mathbf{Y}_{kl},\mathbf{Y}_{ij})-\lambda_a\right\}\right]\right)=0,$$

and rearranged into

$$\begin{aligned}&\mathbb{E}\left\{\sum_{1\le i\neq k\le m}\frac{\mathbb{1}(A_i=a)\mathbb{1}(A_k=1-a)N_iN_k}{M_iM_k}\sum_{j=1}^{N_i}\sum_{l=1}^{N_k}S_{ij}S_{kl}w(\mathbf{Y}_{ij},\mathbf{Y}_{kl})\right\}\\&=\lambda_a\mathbb{E}\left\{\sum_{1\le i\neq k\le m}\mathbb{1}(A_i=a)\mathbb{1}(A_k=1-a)N_iN_k\right\}.\end{aligned}$$

Similar to the previous derivations for the cp-GCE, the left-hand side of the above equality can be shown to be

$$\pi(1-\pi)\mathbb{E}\left[\sum_{j=1}^{N_i}\sum_{l=1}^{N_k}w\{\mathbf{Y}_{ij}(a),\mathbf{Y}_{kl}(1-a)\}\right],$$

and the right-hand side is $\pi(1-\pi)\mathbb{E}(N_iN_k)$, which gives us

$$\lambda_a=\lambda_{I,a}=\frac{\mathbb{E}\left[\sum_{j=1}^{N_i}\sum_{l=1}^{N_k}w\{\mathbf{Y}_{ij}(a),\mathbf{Y}_{kl}(1-a)\}\right]}{\mathbb{E}(N_iN_k)}.$$

The proof is complete. □

#### S8.3.3 The efficient influence functions

*Proof of Theorem S2.* We derive efficient influence functions (EIFs) for the cp- and ip-GCE. We first derive the EIF for $\lambda_{C,a}=\mathbb{E}\left[\overline{w}\{\mathbf{Y}_i(a),\mathbf{Y}_k(1-a)\}\right]$. By Lemma S3 and the iterative conditional expectation,

$$\begin{aligned}\lambda_{C,a}&=\mathbb{E}\left[\overline{w}\{\mathbf{Y}_i(a),\mathbf{Y}_k(1-a)\}\right]\\&=\mathbb{E}\left(\mathbb{E}\left[\overline{w}\{\mathbf{Y}_i(a),\mathbf{Y}_k(1-a)\}|N_i,N_k\right]\right)\\&=\mathbb{E}\left(\mathbb{E}\left[\mathbb{E}\left\{\overline{w}(\mathbf{Y}_i,\mathbf{Y}_k)|A_i=a,A_k=1-a,N_i,N_k,\boldsymbol{C}_i,\boldsymbol{C}_k\right\}|N_i,N_k\right]\right)\\&=\mathbb{E}\left\{\mathbb{E}\left(\mathbb{E}\left[\mathbb{E}\left\{\overline{w}(\mathbf{Y}_i,\mathbf{Y}_k)\middle|\begin{matrix}A_i,M_i,N_i,\boldsymbol{C}_i,\\A_k,M_k,N_k,\boldsymbol{C}_k\end{matrix}\right\}\middle|\begin{matrix}A_i,N_i,\boldsymbol{C}_i,\\A_k,N_k,\boldsymbol{C}_k\end{matrix}\right]\middle|N_i,N_k\right)\right\}\end{aligned}$$

$$= \mathbb{E}\left[\mathbb{E}\left\{\mathbb{E}\left(\mathbb{E}\left[\mathbb{E}\left\{\overline{w}(\mathbf{Y}_i,\mathbf{Y}_k)\middle| \begin{array}{l} A_i,\mathbf{X}_i,M_i,N_i,\boldsymbol{C}_i, \\ A_k,\mathbf{X}_k,M_k,N_k,\boldsymbol{C}_k \end{array}\right\}\middle| \begin{array}{l} A_i,M_i,N_i,\boldsymbol{C}_i, \\ A_k,M_k,N_k,\boldsymbol{C}_k \end{array}\right]\middle| \begin{array}{l} A_i,N_i,\boldsymbol{C}_i, \\ A_k,N_k,\boldsymbol{C}_k \end{array}\right)\middle| N_i,N_k\right\}\right]$$

$$= \mathbb{E}\left[\mathbb{E}\left\{\mathbb{E}\left(\mathbb{E}\left[\mathbb{E}\left\{\overline{w}(\mathbf{Y}_i^o,\mathbf{Y}_k^o)\middle| \begin{array}{l} A_i,\mathbf{X}_i^o,M_i,N_i,\boldsymbol{C}_i, \\ A_k,\mathbf{X}_k^o,M_k,N_k,\boldsymbol{C}_k \end{array}\right\}\middle| \begin{array}{l} A_i,M_i,N_i,\boldsymbol{C}_i, \\ A_k,M_k,N_k,\boldsymbol{C}_k \end{array}\right]\middle| \begin{array}{l} A_i,N_i,\boldsymbol{C}_i, \\ A_k,N_k,\boldsymbol{C}_k \end{array}\right)\middle| N_i,N_k\right\}\right]$$

$$= \mathbb{E}\left[\mathbb{E}\left\{\mathbb{E}\left(\mathbb{E}\left[\mathbb{E}\left\{\overline{w}(\mathbf{Y}_i^o,\mathbf{Y}_k^o)\middle| \begin{array}{l} A_i,\mathbf{X}_i^o,M_i,N_i,\boldsymbol{C}_i, \\ A_k,\mathbf{X}_k^o,M_k,N_k,\boldsymbol{C}_k \end{array}\right\}\middle| \begin{array}{l} M_i,N_i,\boldsymbol{C}_i, \\ M_k,N_k,\boldsymbol{C}_k \end{array}\right]\middle| \begin{array}{l} A_i,N_i,\boldsymbol{C}_i, \\ A_k,N_k,\boldsymbol{C}_k \end{array}\right)\middle| N_i,N_k\right\}\right].$$

We use the point contamination approach (Hines et al., 2022) to derive the EIFs, where for $\mathcal{O}$ and its density function $f(o)$, the point contaminated density $f_t(o) = t\mathbb{1}_{\tilde{\mathcal{O}}}(o) + (1-t)f(o)$. The observed data for cluster $i$ is $\mathcal{O}_i = (\mathbf{Y}_i^o, \mathbf{X}_i^o, M_i, A_i, N_i, \boldsymbol{C}_i)$, the distribution of which is

$$\mathcal{P}(\mathcal{O}) = \mathcal{P}(\mathbf{Y}^o|\mathbf{X}^o, M, A, N, \boldsymbol{C})\mathcal{P}(\mathbf{X}^o|M, N, \boldsymbol{C})\mathcal{P}(M|A, N, \boldsymbol{C})\mathcal{P}(\boldsymbol{C}|N)\mathcal{P}(N)\mathcal{P}(A).$$

Define

$$\begin{aligned}&\Psi_{C,a,a}(\mathcal{P})\\ &= \int_n\int_{\boldsymbol{c}}\int_m\int_{\mathbf{x}^o}\int_{\mathbf{y}^o} \overline{w}(\mathbf{y}_i^o,\mathbf{y}_k^o) f(\mathbf{y}_i^o|\mathbf{x}_i^o, m_i, \boldsymbol{c}_i, n_i, a) f(\mathbf{y}_k^o|\mathbf{x}_k^o, m_k, \boldsymbol{c}_k, n_k, 1-a) f(\mathbf{x}_i^o|m_i,\boldsymbol{c}_i,n_i) f(\mathbf{x}_k^o|m_k,\boldsymbol{c}_k,n_k)\\ &\qquad \times f(m_i|\boldsymbol{c}_i,n_i,a) f(m_k|\boldsymbol{c}_k,n_k,1-a) f(\boldsymbol{c}_i|n_i) f(\boldsymbol{c}_k|n_k) f(n_i) f(n_k) \mathrm{d}\mathbf{y}^o \mathrm{d}\mathbf{x}^o \mathrm{d}m \mathrm{d}\boldsymbol{c} \mathrm{d}n,\end{aligned}$$

and

$$\begin{aligned}&\Psi_{C,a,1-a}(\mathcal{P})\\ &= \int_n\int_{\boldsymbol{c}}\int_m\int_{\mathbf{x}^o}\int_{\mathbf{y}^o} \overline{w}(\mathbf{y}_k^o,\mathbf{y}_i^o) f(\mathbf{y}_i^o|\mathbf{x}_i^o, m_i, \boldsymbol{c}_i, n_i, 1-a) f(\mathbf{y}_k^o|\mathbf{x}_k^o, m_k, \boldsymbol{c}_k, n_k, a) f(\mathbf{x}_i^o|m_i,\boldsymbol{c}_i,n_i) f(\mathbf{x}_k^o|m_k,\boldsymbol{c}_k,n_k)\\ &\qquad \times f(m_i|\boldsymbol{c}_i,n_i,1-a) f(m_k|\boldsymbol{c}_k,n_k,a) f(\boldsymbol{c}_i|n_i) f(\boldsymbol{c}_k|n_k) f(n_i) f(n_k) \mathrm{d}\mathbf{y}^o \mathrm{d}\mathbf{x}^o \mathrm{d}m \mathrm{d}\boldsymbol{c} \mathrm{d}n,\end{aligned}$$

with

$$\begin{aligned}&\Psi_{C,a,a}(\mathcal{P}_t)\\ &= \int_n\int_{\boldsymbol{c}}\int_m\int_{\mathbf{x}^o}\int_{\mathbf{y}^o} \overline{w}(\mathbf{y}_i^o,\mathbf{y}_k^o) f_t(\mathbf{y}_i^o|\mathbf{x}_i^o, m_i, \boldsymbol{c}_i, n_i, a) f(\mathbf{y}_k^o|\mathbf{x}_k^o, m_k, \boldsymbol{c}_k, n_k, 1-a) f_t(\mathbf{x}_i^o|m_i,\boldsymbol{c}_i,n_i) f(\mathbf{x}_k^o|m_k,\boldsymbol{c}_k,n_k)\\ &\qquad \times f_t(m_i|\boldsymbol{c}_i,n_i,a) f(m_k|\boldsymbol{c}_k,n_k,1-a) f_t(\boldsymbol{c}_i|n_i) f(\boldsymbol{c}_k|n_k) f_t(n_i) f(n_k) \mathrm{d}\mathbf{y}^o \mathrm{d}\mathbf{x}^o \mathrm{d}m \mathrm{d}\boldsymbol{c} \mathrm{d}n,\end{aligned}$$

and

$$\begin{aligned}&\Psi_{C,a,1-a}(\mathcal{P}_t)\\ &= \int_n\int_{\boldsymbol{c}}\int_m\int_{\mathbf{x}^o}\int_{\mathbf{y}^o} \overline{w}(\mathbf{y}_k^o,\mathbf{y}_i^o) f_t(\mathbf{y}_i^o|\mathbf{x}_i^o, m_i, \boldsymbol{c}_i, n_i, 1-a) f(\mathbf{y}_k^o|\mathbf{x}_k^o, m_k, \boldsymbol{c}_k, n_k, a) f_t(\mathbf{x}_i^o|m_i,\boldsymbol{c}_i,n_i) f(\mathbf{x}_k^o|m_k,\boldsymbol{c}_k,n_k)\\ &\qquad \times f_t(m_i|\boldsymbol{c}_i,n_i,1-a) f(m_k|\boldsymbol{c}_k,n_k,a) f_t(\boldsymbol{c}_i|n_i) f(\boldsymbol{c}_k|n_k) f_t(n_i) f(n_k) \mathrm{d}\mathbf{y}^o \mathrm{d}\mathbf{x}^o \mathrm{d}m \mathrm{d}\boldsymbol{c} \mathrm{d}n.\end{aligned}$$

The EIF, defined as the Gâteaux derivative (Hines et al., 2022), is

$$\varphi_{C,a}^{\text{eff}}(\mathcal{O}) = \frac{\mathrm{d}}{\mathrm{d}t}\Psi_{C,a,a}(\mathcal{P}_t)\bigg|_{t=0} + \frac{\mathrm{d}}{\mathrm{d}t}\Psi_{C,a,1-a}(\mathcal{P}_t)\bigg|_{t=0}.$$

Then, by the chain rule, we have

$$\begin{aligned}
&\frac{\mathrm{d}}{\mathrm{d}t}\Psi_{C,a,a}(\mathcal{P}_t)\bigg|_{t=0}\\
&= \int_n\int_{\boldsymbol{c}}\int_m\int_{\mathbf{x}^o}\int_{\mathbf{y}^o} \overline{w}(\mathbf{y}_i^o,\mathbf{y}_k^o)\left\{\frac{\mathrm{d}}{\mathrm{d}t}f_t(\mathbf{y}_i^o|\mathbf{x}_i^o,m_i,\boldsymbol{c}_i,n_i,a)\bigg|_{t=0}\right\} f(\mathbf{y}_k^o|\mathbf{x}_k^o,m_k,\boldsymbol{c}_k,n_k,1-a)f(\mathbf{x}_i^o|m_i,\boldsymbol{c}_i,n_i)\\
&\qquad\times f(\mathbf{x}_k^o|m_k,\boldsymbol{c}_k,n_k)f(m_i|\boldsymbol{c}_i,n_i,a)f(m_k|\boldsymbol{c}_k,n_k,1-a)f(\boldsymbol{c}_i|n_i)f(\boldsymbol{c}_k|n_k)f(n_i)f(n_k)\mathrm{d}\mathbf{y}^o\mathrm{d}\mathbf{x}^o\mathrm{d}m\mathrm{d}\boldsymbol{c}\mathrm{d}n\\
&\quad+\int_n\int_{\boldsymbol{c}}\int_m\int_{\mathbf{x}^o}\int_{\mathbf{y}^o} \overline{w}(\mathbf{y}_i^o,\mathbf{y}_k^o)f(\mathbf{y}_i^o|\mathbf{x}_i^o,m_i,\boldsymbol{c}_i,n_i,a)f(\mathbf{y}_k^o|\mathbf{x}_k^o,m_k,\boldsymbol{c}_k,n_k,1-a)\left\{\frac{\mathrm{d}}{\mathrm{d}t}f_t(\mathbf{x}_i^o|m_i,\boldsymbol{c}_i,n_i)\bigg|_{t=0}\right\}\\
&\qquad\times f(\mathbf{x}_k^o|m_k,\boldsymbol{c}_k,n_k)f(m_i|\boldsymbol{c}_i,n_i,a)f(m_k|\boldsymbol{c}_k,n_k,1-a)f(\boldsymbol{c}_i|n_i)f(\boldsymbol{c}_k|n_k)f(n_i)f(n_k)\mathrm{d}\mathbf{y}^o\mathrm{d}\mathbf{x}^o\mathrm{d}m\mathrm{d}\boldsymbol{c}\mathrm{d}n\\
&\quad+\int_n\int_{\boldsymbol{c}}\int_m\int_{\mathbf{x}^o}\int_{\mathbf{y}^o} \overline{w}(\mathbf{y}_i^o,\mathbf{y}_k^o)f(\mathbf{y}_i^o|\mathbf{x}_i^o,m_i,\boldsymbol{c}_i,n_i,a)f(\mathbf{y}_k^o|\mathbf{x}_k^o,m_k,\boldsymbol{c}_k,n_k,1-a)f(\mathbf{x}_i^o|m_i,\boldsymbol{c}_i,n_i)f(\mathbf{x}_k^o|m_k,\boldsymbol{c}_k,n_k)\\
&\qquad\times\left\{\frac{\mathrm{d}}{\mathrm{d}t}f_t(m_i|\boldsymbol{c}_i,n_i,a)\bigg|_{t=0}\right\}f(m_k|\boldsymbol{c}_k,n_k,1-a)f(\boldsymbol{c}_i|n_i)f(\boldsymbol{c}_k|n_k)f(n_i)f(n_k)\mathrm{d}\mathbf{y}^o\mathrm{d}\mathbf{x}^o\mathrm{d}m\mathrm{d}\boldsymbol{c}\mathrm{d}n\\
&\quad+\int_n\int_{\boldsymbol{c}}\int_m\int_{\mathbf{x}^o}\int_{\mathbf{y}^o} \overline{w}(\mathbf{y}_i^o,\mathbf{y}_k^o)f(\mathbf{y}_i^o|\mathbf{x}_i^o,m_i,\boldsymbol{c}_i,n_i,a)f(\mathbf{y}_k^o|\mathbf{x}_k^o,m_k,\boldsymbol{c}_k,n_k,1-a)f(\mathbf{x}_i^o|m_i,\boldsymbol{c}_i,n_i)f(\mathbf{x}_k^o|m_k,\boldsymbol{c}_k,n_k)\\
&\qquad\times f(m_i|\boldsymbol{c}_i,n_i,a)f(m_k|\boldsymbol{c}_k,n_k,1-a)\left\{\frac{\mathrm{d}}{\mathrm{d}t}f_t(\boldsymbol{c}_i|n_i)\bigg|_{t=0}\right\}f(\boldsymbol{c}_k|n_k)f(n_i)f(n_k)\mathrm{d}\mathbf{y}^o\mathrm{d}\mathbf{x}^o\mathrm{d}m\mathrm{d}\boldsymbol{c}\mathrm{d}n\\
&\quad+\int_n\int_{\boldsymbol{c}}\int_m\int_{\mathbf{x}^o}\int_{\mathbf{y}^o} \overline{w}(\mathbf{y}_i^o,\mathbf{y}_k^o)f(\mathbf{y}_i^o|\mathbf{x}_i^o,m_i,\boldsymbol{c}_i,n_i,a)f(\mathbf{y}_k^o|\mathbf{x}_k^o,m_k,\boldsymbol{c}_k,n_k,1-a)f(\mathbf{x}_i^o|m_i,\boldsymbol{c}_i,n_i)f(\mathbf{x}_k^o|m_k,\boldsymbol{c}_k,n_k)\\
&\qquad\times f(m_i|\boldsymbol{c}_i,n_i,a)f(m_k|\boldsymbol{c}_k,n_k,1-a)\frac{\mathrm{d}}{\mathrm{d}t}f(\boldsymbol{c}_i|n_i)f(\boldsymbol{c}_k|n_k)\left\{f_t(n_i)\bigg|_{t=0}\right\}f(n_k)\mathrm{d}\mathbf{y}^o\mathrm{d}\mathbf{x}^o\mathrm{d}m\mathrm{d}\boldsymbol{c}\mathrm{d}n.
\end{aligned}$$

The first term,

$$\begin{aligned}
&\frac{\mathrm{d}}{\mathrm{d}t}f_t(\mathbf{y}_i^o|\mathbf{x}_i^o,m_i,\boldsymbol{c}_i,n_i,a)\bigg|_{t=0} = \frac{\mathrm{d}}{\mathrm{d}t}\frac{f_t(\mathbf{y}_i^o,\mathbf{x}_i^o,m_i,\boldsymbol{c}_i,n_i,a)}{f_t(\mathbf{x}_i^o,m_i,\boldsymbol{c}_i,n_i,a)}\bigg|_{t=0}\\
&= \frac{f(\mathbf{y}_i^o,\mathbf{x}_i^o,m_i,\boldsymbol{c}_i,n_i,a)}{f(\mathbf{x}_i^o,m_i,\boldsymbol{c}_i,n_i,a)}\left\{\frac{\mathbb{1}_{\tilde{\mathbf{Y}}_i^o}(\mathbf{y}_i^o)\mathbb{1}_{\tilde{\mathbf{X}}_i^o}(\mathbf{x}_i^o)\mathbb{1}_{\tilde{M}_i}(m_i)\mathbb{1}_{\tilde{\boldsymbol{C}}_i}(\boldsymbol{c}_i)\mathbb{1}_{\tilde{N}_i}(n_i)\mathbb{1}_{\tilde{A}_i}(a)}{f(\mathbf{y}_i^o,\mathbf{x}_i^o,m_i,\boldsymbol{c}_i,n_i,a)}\right.\\
&\qquad\left.-\frac{\mathbb{1}_{\tilde{\mathbf{X}}_i^o}(\mathbf{x}_i^o)\mathbb{1}_{\tilde{M}_i}(m_i)\mathbb{1}_{\tilde{\boldsymbol{C}}_i}(\boldsymbol{c}_i)\mathbb{1}_{\tilde{N}_i}(n_i)\mathbb{1}_{\tilde{A}_i}(a)}{f(\mathbf{x}_i^o,m_i,\boldsymbol{c}_i,n_i,a)}\right\}.
\end{aligned}$$

The second term,

$$\begin{aligned}
&\frac{\mathrm{d}}{\mathrm{d}t}f_t(\mathbf{x}_i^o|m_i,\boldsymbol{c}_i,n_i)\bigg|_{t=0} = \frac{\mathrm{d}}{\mathrm{d}t}\frac{f_t(\mathbf{x}_i^o,m_i,\boldsymbol{c}_i,n_i)}{f_t(m_i,\boldsymbol{c}_i,n_i)}\bigg|_{t=0}\\
&= \frac{f(\mathbf{x}_i^o,m_i,\boldsymbol{c}_i,n_i)}{f(m_i,\boldsymbol{c}_i,n_i)}\left\{\frac{\mathbb{1}_{\tilde{\mathbf{X}}_i^o}(\mathbf{x}_i^o)\mathbb{1}_{\tilde{M}_i}(m_i)\mathbb{1}_{\tilde{\boldsymbol{C}}_i}(\boldsymbol{c}_i)\mathbb{1}_{\tilde{N}_i}(n_i)}{f(\mathbf{x}_i^o,m_i,\boldsymbol{c}_i,n_i)} - \frac{\mathbb{1}_{\tilde{M}_i}(m_i)\mathbb{1}_{\tilde{\boldsymbol{C}}_i}(\boldsymbol{c}_i)\mathbb{1}_{\tilde{N}_i}(n_i)}{f(m_i,\boldsymbol{c}_i,n_i)}\right\}.
\end{aligned}$$

The third term,

$$\left.\frac{\mathrm{d}}{\mathrm{d}t}f_t(m_i|\boldsymbol{c}_i,n_i,a)\right|_{t=0} = \left.\frac{\mathrm{d}}{\mathrm{d}t}\frac{f_t(m_i,\boldsymbol{c}_i,n_i,a)}{f_t(\boldsymbol{c}_i,n_i,a)}\right|_{t=0}$$
$$= \frac{f(m_i,\boldsymbol{c}_i,n_i,a)}{f(\boldsymbol{c}_i,n_i,a)}\left\{\frac{\mathbb{1}_{\tilde{M}_i}(m_i)\mathbb{1}_{\tilde{\boldsymbol{C}}_i}(\boldsymbol{c}_i)\mathbb{1}_{\tilde{N}_i}(n_i)\mathbb{1}_{\tilde{A}_i}(a)}{f(m_i,\boldsymbol{c}_i,n_i,a)} - \frac{\mathbb{1}_{\tilde{\boldsymbol{C}}_i}(\boldsymbol{c}_i)\mathbb{1}_{\tilde{N}_i}(n_i)\mathbb{1}_{\tilde{A}_i}(a)}{f(\boldsymbol{c}_i,n_i,a)}\right\}.$$

The fourth term,

$$\left.\frac{\mathrm{d}}{\mathrm{d}t}f_t(\boldsymbol{c}_i|n_i)\right|_{t=0} = \left.\frac{\mathrm{d}}{\mathrm{d}t}\frac{f_t(\boldsymbol{c}_i,n_i)}{f_t(n_i)}\right|_{t=0} = \frac{f(\boldsymbol{c}_i,n_i)}{f(n_i)}\left\{\frac{\mathbb{1}_{\tilde{\boldsymbol{C}}_i}(\boldsymbol{c}_i)\mathbb{1}_{\tilde{N}_i}(n_i)}{f(\boldsymbol{c}_i,n_i)} - \frac{\mathbb{1}_{\tilde{N}_i}(n_i)}{f(n_i)}\right\}.$$

And, the last term,

$$\left.\frac{\mathrm{d}}{\mathrm{d}t}f_t(n_i)\right|_{t=0} = \mathbb{1}_{\tilde{N}_i}(n_i) - f(n_i).$$

Putting all things together,

$$\begin{aligned}
&\left.\frac{\mathrm{d}}{\mathrm{d}t}\Psi_{C,a,a}(\mathcal{P}_t)\right|_{t=0}\\
&= \frac{\mathbb{1}(\tilde{A}_i=a)}{\pi^a(1-\pi)^{1-a}}\left[\mathbb{E}\left\{\overline{w}(\tilde{\mathbf{Y}}_i^o,\mathbf{Y}_k^o)\middle|A_i=a\right\} - \mathbb{E}\left\{\overline{w}(\mathbf{Y}_i^o,\mathbf{Y}_k^o)\middle|\tilde{\mathbf{X}}_i^o,\tilde{M}_i,\tilde{C}_i,\tilde{N}_i,A_i=a\right\}\right]\\
&\quad+\frac{\mathbb{P}(\tilde{M}_i|\tilde{\boldsymbol{C}}_i,\tilde{N}_i,A_i=a)}{\mathbb{P}(\tilde{M}_i|\tilde{\boldsymbol{C}}_i,\tilde{N}_i)}\left[\mathbb{E}\left\{\overline{w}(\mathbf{Y}_i^o,\mathbf{Y}_k^o)\middle|\tilde{\mathbf{X}}_i^o,\tilde{M}_i,\tilde{\boldsymbol{C}}_i,\tilde{N}_i,A_i=a\right\} - \mathbb{E}\left\{\overline{w}(\mathbf{Y}_i^o,\mathbf{Y}_k^o)\middle|\tilde{M}_i,\tilde{\boldsymbol{C}}_i,\tilde{N}_i,A_i=a\right\}\right]\\
&\quad+\frac{\mathbb{1}(\tilde{A}_i=a)}{\pi^a(1-\pi)^{1-a}}\left[\mathbb{E}\left\{\overline{w}(\mathbf{Y}_i^o,\mathbf{Y}_k^o)\middle|\tilde{M}_i,\tilde{\boldsymbol{C}}_i,\tilde{N}_i,A_i=a\right\} - \mathbb{E}\left\{\overline{w}(\mathbf{Y}_i^o,\mathbf{Y}_k^o)\middle|\tilde{\boldsymbol{C}}_i,\tilde{N}_i,A_i=a\right\}\right]\\
&\quad+\mathbb{E}\left\{\overline{w}(\mathbf{Y}_i^o,\mathbf{Y}_k^o)\middle|\tilde{\boldsymbol{C}}_i,\tilde{N}_i,A_i=a\right\} - \Psi_{C,a,a}(\mathcal{P}),
\end{aligned}$$

where the expectation over $\mathbf{Y}_k^o$ is taken with respect to the distribution $p_{\mathbf{Y}^o|A=1-a}(\mathbf{y}^o|1-a)$, and

$$\begin{aligned}
\frac{\mathbb{P}(M_i|\boldsymbol{C}_i,N_i,A_i=a)}{\mathbb{P}(M_i|\boldsymbol{C}_i,N_i)} &= \frac{\mathbb{P}(M_i,\boldsymbol{C}_i,N_i,A_i=a)}{\mathbb{P}(M_i,\boldsymbol{C}_i,N_i)}\times\frac{\mathbb{P}(\boldsymbol{C}_i,N_i)}{\mathbb{P}(A_i=a,\boldsymbol{C}_i,N_i)}\\
=\frac{\mathbb{P}(A_i=a|M_i,\boldsymbol{C}_i,N_i)}{\mathbb{P}(A_i=a|\boldsymbol{C}_i,N_i)} &= \frac{\mathbb{P}(A_i=a|M_i,\boldsymbol{C}_i,N_i)}{\pi^a(1-\pi)^{1-a}}.
\end{aligned}$$

Similarly,

$$\begin{aligned}
&\left.\frac{\mathrm{d}}{\mathrm{d}t}\Psi_{C,a,1-a}(\mathcal{P}_t)\right|_{t=0}\\
&= \frac{\mathbb{1}(\tilde{A}_i=1-a)}{\pi^{1-a}(1-\pi)^{a}}\left[\mathbb{E}\left\{\overline{w}(\mathbf{Y}_k^o,\tilde{\mathbf{Y}}_i^o)\middle|A_i=1-a\right\} - \mathbb{E}\left\{\overline{w}(\mathbf{Y}_k^o,\mathbf{Y}_i^o)\middle|\tilde{\mathbf{X}}_i^o,\tilde{M}_i,\tilde{\boldsymbol{C}}_i,\tilde{N}_i,A_i=1-a\right\}\right]\\
&\quad+\frac{\mathbb{P}(\tilde{M}_i|\tilde{\boldsymbol{C}}_i,\tilde{N}_i,A_i=1-a)}{\mathbb{P}(\tilde{M}_i|\tilde{\boldsymbol{C}}_i,\tilde{N}_i)}\left[\mathbb{E}\left\{\overline{w}(\mathbf{Y}_k^o,\mathbf{Y}_i^o)\middle|\tilde{\mathbf{X}}_i^o,\tilde{M}_i,\tilde{\boldsymbol{C}}_i,\tilde{N}_i,A_i=1-a\right\}\right.\\
&\qquad\qquad\left.-\mathbb{E}\left\{\overline{w}(\mathbf{Y}_k^o,\mathbf{Y}_i^o)\middle|\tilde{M}_i,\tilde{\boldsymbol{C}}_i,\tilde{N}_i,A_i=1-a\right\}\right]
\end{aligned}$$

$$+\frac{\mathbb{1}(\tilde{A}_i=1-a)}{\pi^{1-a}(1-\pi)^a}\left[\mathbb{E}\left\{\overline{w}(\mathbf{Y}_k^o,\mathbf{Y}_i^o)\middle|\tilde{M}_i,\tilde{\boldsymbol{C}}_i,\tilde{N}_i,A_i=1-a\right\}-\mathbb{E}\left\{\overline{w}(\mathbf{Y}_k^o,\mathbf{Y}_i^o)\middle|\tilde{\boldsymbol{C}}_i,\tilde{N}_i,A_i=1-a\right\}\right]$$
$$+\mathbb{E}\left\{\overline{w}(\mathbf{Y}_k^o,\mathbf{Y}_i^o)\middle|\tilde{\boldsymbol{C}}_i,\tilde{N}_i,A_i=1-a\right\}-\Psi_{C,a,1-a}(\mathcal{P}),$$

where the expectation over $\mathbf{Y}_k^o$ is taken with respect to the distribution $p_{\mathbf{Y}^o|A=a}(\mathbf{y}^o|a)$, and

$$\frac{\mathbb{P}(M_i|\boldsymbol{C}_i,N_i,A_i=1-a)}{\mathbb{P}(M_i|\boldsymbol{C}_i,N_i)}=\frac{\mathbb{P}(A_i=1-a|M_i,\boldsymbol{C}_i,N_i)}{\pi^{1-a}(1-\pi)^a}.$$

Then, define

$$\mathfrak{w}_{C,a,a}(\mathbf{y})=\mathbb{E}\left\{\overline{w}(\mathbf{y},\mathbf{Y}_k^o)|A_k=1-a\right\}\quad\text{and}\quad\mathfrak{w}_{C,a,1-a}(\mathbf{y})=\mathbb{E}\left\{\overline{w}(\mathbf{Y}_k^o,\mathbf{y})|A_k=a\right\},$$

and the EIF for $\lambda_{C,a}$ is

$$\begin{aligned}
&\varphi_{C,a}^{\text{eff}}(\mathcal{O})\\
&=\frac{\mathbb{1}(A=a)}{\pi^a(1-\pi)^{1-a}}\left[\mathfrak{w}_{C,a,a}(\mathbf{Y}^o)-\mathbb{E}\left\{\mathfrak{w}_{C,a,a}(\mathbf{Y}^o)|\mathbf{X}^o,M,\boldsymbol{C},N,A=a\right\}\right]\\
&\quad+\frac{\mathbb{1}(A=1-a)}{\pi^{1-a}(1-\pi)^a}\left[\mathfrak{w}_{C,a,1-a}(\mathbf{Y}^o)-\mathbb{E}\left\{\mathfrak{w}_{C,a,1-a}(\mathbf{Y}^o)|\mathbf{X}^o,M,\boldsymbol{C},N,A=1-a\right\}\right]\\
&\quad+\frac{\mathbb{P}(A=a|M,\boldsymbol{C},N)}{\pi^a(1-\pi)^{1-a}}\left[\mathbb{E}\left\{\mathfrak{w}_{C,a,a}(\mathbf{Y}^o)|\mathbf{X}^o,M,\boldsymbol{C},N,A=a\right\}-\mathbb{E}\left\{\mathfrak{w}_{C,a,a}(\mathbf{Y}^o)|M,\boldsymbol{C},N,A=a\right\}\right]\\
&\quad+\frac{\mathbb{P}(A=1-a|M,\boldsymbol{C},N)}{\pi^{1-a}(1-\pi)^a}\left[\mathbb{E}\left\{\mathfrak{w}_{C,a,1-a}(\mathbf{Y}^o)|\mathbf{X}^o,M,\boldsymbol{C},N,A=1-a\right\}-\mathbb{E}\left\{\mathfrak{w}_{C,a,1-a}(\mathbf{Y}^o)|M,\boldsymbol{C},N,A=1-a\right\}\right]\\
&\quad+\frac{\mathbb{1}(A=a)}{\pi^a(1-\pi)^{1-a}}\left[\mathbb{E}\left\{\mathfrak{w}_{C,a,a}(\mathbf{Y}^o)|M,\boldsymbol{C},N,A=a\right\}-\mathbb{E}\left\{\mathfrak{w}_{C,a,a}(\mathbf{Y}^o)|\boldsymbol{C},N,A=a\right\}\right]\\
&\quad+\frac{\mathbb{1}(A=1-a)}{\pi^{1-a}(1-\pi)^a}\left[\mathbb{E}\left\{\mathfrak{w}_{C,a,1-a}(\mathbf{Y}^o)|M,\boldsymbol{C},N,A=1-a\right\}-\mathbb{E}\left\{\mathfrak{w}_{C,a,1-a}(\mathbf{Y}^o)|\boldsymbol{C},N,A=1-a\right\}\right]\\
&\quad+\mathbb{E}\left\{\mathfrak{w}_{C,a,a}(\mathbf{Y}^o)|\boldsymbol{C},N,A=a\right\}+\mathbb{E}\left\{\mathfrak{w}_{C,a,1-a}(\mathbf{Y}^o)|\boldsymbol{C},N,A=a\right\}-2\lambda_{C,a},
\end{aligned}$$

which reduces to the EIF in Mao (2017) when $M_i=M_k=N_i=N_k=1$. By Lemma S3,

$$\mathbb{E}\left\{\mathfrak{w}_{C,a,a}(\mathbf{Y}^o)|M,\boldsymbol{C},N,A=a\right\}=\mathbb{E}\left\{\mathfrak{w}_{C,a,a}(\mathbf{Y}^o)|\boldsymbol{C},N,A=a\right\},$$

and

$$\mathbb{E}\left\{\mathfrak{w}_{C,a,1-a}(\mathbf{Y}^o)|\mathbf{X}^o,M,\boldsymbol{C},N,A=1-a\right\}=\mathbb{E}\left\{\mathfrak{w}_{C,a,1-a}(\mathbf{Y}^o)|M,\boldsymbol{C},N,A=1-a\right\}.$$

Then, the EIF can be simplified into

$$\begin{aligned}
&\varphi_{C,a}^{\text{eff}}(\mathcal{O})\\
&=\frac{\mathbb{1}(A=a)}{\pi^a(1-\pi)^{1-a}}\left[\mathfrak{w}_{C,a,a}(\mathbf{Y}^o)-\mathbb{E}\left\{\mathfrak{w}_{C,a,a}(\mathbf{Y}^o)|\mathbf{X}^o,M,\boldsymbol{C},N,A=a\right\}\right]\\
&\quad+\frac{\mathbb{1}(A=1-a)}{\pi^{1-a}(1-\pi)^a}\left[\mathfrak{w}_{C,a,1-a}(\mathbf{Y}^o)-\mathbb{E}\left\{\mathfrak{w}_{C,a,1-a}(\mathbf{Y}^o)|\mathbf{X}^o,M,\boldsymbol{C},N,A=1-a\right\}\right]
\end{aligned}$$

$$+\frac{\mathbb{P}(A=a|M,\boldsymbol{C},N)}{\pi^a(1-\pi)^{1-a}}\left[\mathbb{E}\left\{\mathfrak{w}_{C,a,a}(\mathbf{Y}^o)|\mathbf{X}^o,M,\boldsymbol{C},N,A=a\right\}-\mathbb{E}\left\{\mathfrak{w}_{C,a,a}(\mathbf{Y}^o)|\boldsymbol{C},N,A=a\right\}\right]$$
$$+\frac{\mathbb{P}(A=1-a|M,\boldsymbol{C},N)}{\pi^{1-a}(1-\pi)^{a}}\left[\mathbb{E}\left\{\mathfrak{w}_{C,a,1-a}(\mathbf{Y}^o)|\mathbf{X}^o,M,\boldsymbol{C},N,A=1-a\right\}-\mathbb{E}\left\{\mathfrak{w}_{C,a,1-a}(\mathbf{Y}^o)|\boldsymbol{C},N,A=1-a\right\}\right]$$
$$+\mathbb{E}\left\{\mathfrak{w}_{C,a,a}(\mathbf{Y}^o)|\boldsymbol{C},N,A=a\right\}+\mathbb{E}\left\{\mathfrak{w}_{C,a,1-a}(\mathbf{Y}^o)|\boldsymbol{C},N,A=a\right\}-2\lambda_{C,a}.$$

We then derive the EIF for the ip-GCE

$$\lambda_{I,a}=\frac{\mathbb{E}[N_iN_k\overline{w}\{\mathbf{Y}_i^o(a),\mathbf{Y}_k^o(1-a)\}]}{\mathbb{E}(N_iN_k)},$$

where $\lambda_{I,a}=\lambda_{I,a}^{\text{num}}/\lambda_I^{\text{den}}$, with $\lambda_{I,a}^{\text{num}}=\mathbb{E}[N_iN_k\overline{w}\{\mathbf{Y}_i^o(a),\mathbf{Y}_k^o(1-a)\}]$ and $\lambda_I^{\text{den}}=\mathbb{E}(N_iN_k)$. The EIF for $\lambda_{I,a}$ is in the form of

$$\varphi_{I,a}^{\text{eff}}(\mathcal{O})=\frac{1}{\lambda_I^{\text{den}}}\varphi_{I,a}^{\text{eff-num}}(\mathcal{O})-\frac{\lambda_{I,a}}{\lambda_I^{\text{den}}}\varphi_I^{\text{eff-den}}(\mathcal{O}),$$

where $\varphi_{I,1}^{\text{eff-num}}(\mathcal{O})$ is the EIF for $\lambda_{I,a}^{\text{num}}$ and $\varphi_I^{\text{eff-den}}(\mathcal{O})$ is the EIF for $\lambda_I^{\text{den}}$. Similar to the derivations for the cp-GCE, define

$$\begin{aligned}&\Psi_{I,a,a}(\mathcal{P})\\&=\int_n\int_{\boldsymbol{c}}\int_m\int_{\mathbf{x}^o}\int_{\mathbf{y}^o}n_in_k\overline{w}(\mathbf{y}_i^o,\mathbf{y}_k^o)f(\mathbf{y}_i^o|\mathbf{x}_i^o,m_i,\boldsymbol{c}_i,n_i,a)f(\mathbf{y}_k^o|\mathbf{x}_k^o,m_k,\boldsymbol{c}_k,n_k,1-a)f(\mathbf{x}_i^o|m_i,\boldsymbol{c}_i,n_i)f(\mathbf{x}_k^o|m_k,\boldsymbol{c}_k,n_k)\\&\qquad\times f(m_i|\boldsymbol{c}_i,n_i,a)f(m_k|\boldsymbol{c}_k,n_k,1-a)f(\boldsymbol{c}_i|n_i)f(\boldsymbol{c}_k|n_k)f(n_i)f(n_k)\mathrm{d}\mathbf{y}^o\mathrm{d}\mathbf{x}^o\mathrm{d}m\mathrm{d}\boldsymbol{c}\mathrm{d}n,\end{aligned}$$

and

$$\begin{aligned}&\Psi_{I,a,1-a}(\mathcal{P})\\&=\int_n\int_{\boldsymbol{c}}\int_m\int_{\mathbf{x}^o}\int_{\mathbf{y}^o}n_in_k\overline{w}(\mathbf{y}_k^o,\mathbf{y}_i^o)f(\mathbf{y}_i^o|\mathbf{x}_i^o,m_i,\boldsymbol{c}_i,n_i,1-a)f(\mathbf{y}_k^o|\mathbf{x}_k^o,m_k,\boldsymbol{c}_k,n_k,a)f(\mathbf{x}_i^o|m_i,\boldsymbol{c}_i,n_i)f(\mathbf{x}_k^o|m_k,\boldsymbol{c}_k,n_k)\\&\qquad\times f(m_i|\boldsymbol{c}_i,n_i,1-a)f(m_k|\boldsymbol{c}_k,n_k,a)f(\boldsymbol{c}_i|n_i)f(\boldsymbol{c}_k|n_k)f(n_i)f(n_k)\mathrm{d}\mathbf{y}^o\mathrm{d}\mathbf{x}^o\mathrm{d}m\mathrm{d}\boldsymbol{c}\mathrm{d}n,\end{aligned}$$

with

$$\begin{aligned}&\Psi_{I,a,a}(\mathcal{P}_t)\\&=\int_n\int_{\boldsymbol{c}}\int_m\int_{\mathbf{x}^o}\int_{\mathbf{y}^o}n_in_k\overline{w}(\mathbf{y}_i^o,\mathbf{y}_k^o)f_t(\mathbf{y}_i^o|\mathbf{x}_i^o,m_i,\boldsymbol{c}_i,n_i,a)f(\mathbf{y}_k^o|\mathbf{x}_k^o,m_k,\boldsymbol{c}_k,n_k,1-a)f_t(\mathbf{x}_i^o|m_i,\boldsymbol{c}_i,n_i)f(\mathbf{x}_k^o|m_k,\boldsymbol{c}_k,n_k)\\&\qquad\times f_t(m_i|\boldsymbol{c}_i,n_i,a)f(m_k|\boldsymbol{c}_k,n_k,1-a)f_t(\boldsymbol{c}_i|n_i)f(\boldsymbol{c}_k|n_k)f_t(n_i)f(n_k)\mathrm{d}\mathbf{y}^o\mathrm{d}\mathbf{x}^o\mathrm{d}m\mathrm{d}\boldsymbol{c}\mathrm{d}n,\end{aligned}$$

and

$$\begin{aligned}&\Psi_{I,a,1-a}(\mathcal{P}_t)\\&=\int_n\int_{\boldsymbol{c}}\int_m\int_{\mathbf{x}^o}\int_{\mathbf{y}^o}n_in_k\overline{w}(\mathbf{y}_k^o,\mathbf{y}_i^o)f_t(\mathbf{y}_i^o|\mathbf{x}_i^o,m_i,\boldsymbol{c}_i,n_i,1-a)f(\mathbf{y}_k^o|\mathbf{x}_k^o,m_k,\boldsymbol{c}_k,n_k,a)f_t(\mathbf{x}_i^o|m_i,\boldsymbol{c}_i,n_i)f(\mathbf{x}_k^o|m_k,\boldsymbol{c}_k,n_k)\\&\qquad\times f_t(m_i|\boldsymbol{c}_i,n_i,1-a)f(m_k|\boldsymbol{c}_k,n_k,a)f_t(\boldsymbol{c}_i|n_i)f(\boldsymbol{c}_k|n_k)f_t(n_i)f(n_k)\mathrm{d}\mathbf{y}^o\mathrm{d}\mathbf{x}^o\mathrm{d}m\mathrm{d}\boldsymbol{c}\mathrm{d}n.\end{aligned}$$

The EIF for $\lambda_{I,a}^{\text{num}}$ is

$$\varphi_{I,a}^{\text{eff-num}}(\mathcal{O}) = \frac{\mathrm{d}}{\mathrm{d}t}\Psi_{I,a,a}(\mathcal{P}_t)\Big|_{t=0} + \frac{\mathrm{d}}{\mathrm{d}t}\Psi_{I,a,1-a}(\mathcal{P}_t)\Big|_{t=0},$$

which, via similar derivations, is

$$\begin{aligned}
&\varphi_{I,a}^{\text{eff-num}}(\mathcal{O}) \\
&= \frac{\mathbb{1}(A=a)N}{\pi^a(1-\pi)^{1-a}}\left[\mathfrak{w}_{I,a,a}(\mathbf{Y}^o) - \mathbb{E}\left\{\mathfrak{w}_{I,a,a}(\mathbf{Y}^o)|\mathbf{X}^o, M, \boldsymbol{C}, N, A=a\right\}\right] \\
&\quad + \frac{\mathbb{1}(A=1-a)N}{\pi^{1-a}(1-\pi)^a}\left[\mathfrak{w}_{I,a,1-a}(Y^o) - \mathbb{E}\left\{\mathfrak{w}_{I,a,1-a}(\mathbf{Y}^o)|\mathbf{X}^o, M, \boldsymbol{C}, N, A=1-a\right\}\right] \\
&\quad + \frac{\mathbb{P}(A=a|M,\boldsymbol{C},N)N}{\pi^a(1-\pi)^{1-a}}\left[\mathbb{E}\left\{\mathfrak{w}_{I,a,a}(\mathbf{Y}^o)|\mathbf{X}^o, M, \boldsymbol{C}, N, A=a\right\} - \mathbb{E}\left\{\mathfrak{w}_{I,a,a}(\mathbf{Y}^o)|M, \boldsymbol{C}, N, A=a\right\}\right] \\
&\quad + \frac{\mathbb{P}(A=1-a|M,\boldsymbol{C},N)N}{\pi^{1-a}(1-\pi)^a}\left[\mathbb{E}\left\{\mathfrak{w}_{I,a,1-a}(\mathbf{Y}^o)|\mathbf{X}^o, M, \boldsymbol{C}, N, A=1-a\right\} - \mathbb{E}\left\{\mathfrak{w}_{I,a,1-a}(Y^o)|M, \boldsymbol{C}, N, A=1-a\right\}\right] \\
&\quad + \frac{\mathbb{1}(A=a)N}{\pi^a(1-\pi)^{1-a}}\left[\mathbb{E}\left\{\mathfrak{w}_{I,a,a}(\mathbf{Y}^o)|M, \boldsymbol{C}, N, A=a\right\} - \mathbb{E}\left\{\mathfrak{w}_{I,a,a}(\mathbf{Y}^o)|\boldsymbol{C}, N, A=a\right\}\right] \\
&\quad + \frac{\mathbb{1}(A=1-a)N}{\pi^{1-a}(1-\pi)^a}\left[\mathbb{E}\left\{\mathfrak{w}_{I,a,1-a}(\mathbf{Y}^o)|M, \boldsymbol{C}, N, A=1-a\right\} - \mathbb{E}\left\{\mathfrak{w}_{I,a,1-a}(\mathbf{Y}^o)|\boldsymbol{C}, N, A=1-a\right\}\right] \\
&\quad + N\mathbb{E}\left\{\mathfrak{w}_{I,a,a}(\mathbf{Y}^o)|\boldsymbol{C}, N, A=a\right\} + N\mathbb{E}\left\{\mathfrak{w}_{I,a,1-a}(\mathbf{Y}^o)|\boldsymbol{C}, N, A=1-a\right\} - 2\lambda_{I,a}^{\text{num}},
\end{aligned}$$

with

$$\mathfrak{w}_{I,a,a}(\mathbf{y}) = \mathbb{E}\left\{N_k\overline{w}(\mathbf{y}, \mathbf{Y}_k^o)|A_k=1-a\right\} \quad \text{and} \quad \mathfrak{w}_{I,a,1-a}(\mathbf{y}) = \mathbb{E}\left\{N_k\overline{w}(\mathbf{Y}_k^o, \mathbf{y})|A_k=a\right\}.$$

The EIF for $\lambda_I^{\text{den}}$ is

$$\varphi_I^{\text{eff-den}}(\mathcal{O}) = 2N\mathbb{E}(N) - 2\lambda_I^{\text{den}}.$$

Putting all things together,

$$\begin{aligned}
&\varphi_{I,a}^{\text{eff}}(\mathcal{O}) \\
&= \frac{\mathbb{1}(A=a)N}{\pi^a(1-\pi)^{1-a}\{\mathbb{E}(N)\}^2}\left[\mathfrak{w}_{I,a,a}(\mathbf{Y}^o) - \mathbb{E}\left\{\mathfrak{w}_{I,a,a}(\mathbf{Y}^o)|\mathbf{X}^o, M, \boldsymbol{C}, N, A=a\right\}\right] \\
&\quad + \frac{\mathbb{1}(A=1-a)N}{\pi^{1-a}(1-\pi)^a\{\mathbb{E}(N)\}^2}\left[\mathfrak{w}_{I,a,1-a}(\mathbf{Y}^o) - \mathbb{E}\left\{\mathfrak{w}_{I,a,1-a}(\mathbf{Y}^o)|\mathbf{X}^o, M, \boldsymbol{C}, N, A=1-a\right\}\right] \\
&\quad + \frac{\mathbb{P}(A=a|M,\boldsymbol{C},N)N}{\pi^a(1-\pi)^{1-a}\{\mathbb{E}(N)\}^2}\left[\mathbb{E}\left\{\mathfrak{w}_{I,a,a}(\mathbf{Y}^o)|\mathbf{X}^o, M, \boldsymbol{C}, N, A=a\right\} - \mathbb{E}\left\{\mathfrak{w}_{I,a,a}(\mathbf{Y}^o)|M, \boldsymbol{C}, N, A=a\right\}\right] \\
&\quad + \frac{\mathbb{P}(A=1-a|M,\boldsymbol{C},N)N}{\pi^{1-a}(1-\pi)^a\{\mathbb{E}(N)\}^2}\left[\mathbb{E}\left\{\mathfrak{w}_{I,a,1-a}(\mathbf{Y}^o)|\mathbf{X}^o, M, \boldsymbol{C}, N, A=1-a\right\}\right. \\
&\qquad\qquad \left. - \mathbb{E}\left\{\mathfrak{w}_{I,a,1-a}(\mathbf{Y}^o)|M, \boldsymbol{C}, N, A=1-a\right\}\right] \\
&\quad + \frac{\mathbb{1}(A=a)N}{\pi^a(1-\pi)^{1-a}\{\mathbb{E}(N)\}^2}\left[\mathbb{E}\left\{\mathfrak{w}_{I,a,a}(\mathbf{Y}^o)|M, \boldsymbol{C}, N, A=a\right\} - \mathbb{E}\left\{\mathfrak{w}_{I,a,a}(\mathbf{Y}^o)|\boldsymbol{C}, N, A=a\right\}\right]
\end{aligned}$$

$$+ \frac{\mathbb{1}(A = 1-a)N}{\pi^{1-a}(1-\pi)^a\{\mathbb{E}(N)\}^2} \left[\mathbb{E}\left\{\mathfrak{w}_{I,a,1-a}(\mathbf{Y}^o)|M,\boldsymbol{C},N,A=1-a\right\} - \mathbb{E}\left\{\mathfrak{w}_{I,a,1-a}(\mathbf{Y}^o)|\boldsymbol{C},N,A=1-a\right\}\right]$$
$$+ \frac{N}{\{\mathbb{E}(N)\}^2}\mathbb{E}\left\{\mathfrak{w}_{I,a,a}(\mathbf{Y}^o)|\boldsymbol{C},N,A=a\right\} + \frac{N}{\{\mathbb{E}(N)\}^2}\mathbb{E}\left\{\mathfrak{w}_{I,a,1-a}(\mathbf{Y}^o)|\boldsymbol{C},N,A=1-a\right\} - \frac{2N\lambda_{I,a}}{\mathbb{E}(N)},$$

which also reduces to the EIF in Mao (2017) when $M_i = M_k = N_i = N_k = 1$. Similar to $\varphi^{\text{eff}}_{C,a}(\mathcal{O})$, by Lemma S3,

$$\begin{aligned}
&\varphi^{\text{eff}}_{I,a}(\mathcal{O}) \\
&= \frac{\mathbb{1}(A=a)N}{\pi^a(1-\pi)^{1-a}\{\mathbb{E}(N)\}^2}\left[\mathfrak{w}_{I,a,a}(\mathbf{Y}^o) - \mathbb{E}\left\{\mathfrak{w}_{I,a,a}(\mathbf{Y}^o)|\mathbf{X}^o,M,\boldsymbol{C},N,A=a\right\}\right] \\
&\quad + \frac{\mathbb{1}(A=1-a)N}{\pi^{1-a}(1-\pi)^a\{\mathbb{E}(N)\}^2}\left[\mathfrak{w}_{I,a,1-a}(\mathbf{Y}^o) - \mathbb{E}\left\{\mathfrak{w}_{I,a,1-a}(\mathbf{Y}^o)|\mathbf{X}^o,M,\boldsymbol{C},N,A=1-a\right\}\right] \\
&\quad + \frac{\mathbb{P}(A=a|M,\boldsymbol{C},N)N}{\pi^a(1-\pi)^{1-a}\{\mathbb{E}(N)\}^2}\left[\mathbb{E}\left\{\mathfrak{w}_{I,a,a}(\mathbf{Y}^o)|\mathbf{X}^o,M,\boldsymbol{C},N,A=a\right\} - \mathbb{E}\left\{\mathfrak{w}_{I,a,a}(\mathbf{Y}^o)|\boldsymbol{C},N,A=a\right\}\right] \\
&\quad + \frac{\mathbb{P}(A=1-a|M,\boldsymbol{C},N)N}{\pi^{1-a}(1-\pi)^a\{\mathbb{E}(N)\}^2}\left[\mathbb{E}\left\{\mathfrak{w}_{I,a,1-a}(\mathbf{Y}^o)|\mathbf{X}^o,M,\boldsymbol{C},N,A=1-a\right\} - \mathbb{E}\left\{\mathfrak{w}_{I,a,1-a}(\mathbf{Y}^o)|\boldsymbol{C},N,A=1-a\right\}\right] \\
&\quad + \frac{N}{\{\mathbb{E}(N)\}^2}\mathbb{E}\left\{\mathfrak{w}_{I,a,a}(\mathbf{Y}^o)|\boldsymbol{C},N,A=a\right\} + \frac{N}{\{\mathbb{E}(N)\}^2}\mathbb{E}\left\{\mathfrak{w}_{I,a,1-a}(\mathbf{Y}^o)|\boldsymbol{C},N,A=1-a\right\} - \frac{2N\lambda_{I,a}}{\mathbb{E}(N)}.
\end{aligned}$$

After the derivations, we verify that $\varphi^{\text{eff}}_{C,a}(\mathcal{O}), \varphi^{\text{eff}}_{I,a}(\mathcal{O}) \in \mathcal{T}$, the tangent space of the observed data constrained by Assumptions 1-3 in the main article and Assumption S1. Recall that the observed data distribution is

$$\mathcal{P}(\mathcal{O}) = \mathcal{P}(\mathbf{Y}^o|\mathbf{X}^o,M,A,N,\boldsymbol{C})\mathcal{P}(\mathbf{X}^o|M,N,\boldsymbol{C})\mathcal{P}(M|A,N,\boldsymbol{C})\mathcal{P}(\boldsymbol{C}|N)\mathcal{P}(N)\mathcal{P}(A),$$

where $\mathcal{P}(A)$ is known. Let $\mathcal{L}_{2,0}(\mathcal{O})$ denote the set of functions of a random variable $\mathcal{O}$ that have zero mean and a finite variance, i.e.,

$$\mathcal{L}_{2,0}(\mathcal{O}) = \left\{L(\mathcal{O})\middle|\mathbb{E}\{L(\mathcal{O})\} = 0,\ \mathbb{E}[\{L(\mathcal{O})\}^2] < \infty\right\}.$$

Then, the tangent space of the model constrained by Assumptions 1-3 and S1 is

$$\mathcal{T} = \left\{ L(\mathcal{O}) \in \mathcal{L}_{2,0}(\mathcal{O}) \,\middle|\, \begin{array}{c} L(\mathcal{O}) = L_{\mathbf{Y}^o}(\mathbf{Y}^o,\mathbf{X}^o,M,A,N,\boldsymbol{C}) + L_{\mathbf{X}^o}(\mathbf{X}^o,M,A,N,\boldsymbol{C}) \\ +L_M(M,N,\boldsymbol{C},A) + L_{\boldsymbol{C}}(\boldsymbol{C},N) + L_N(N) \end{array} \right\},$$

where

$$\begin{aligned}
&\mathbb{E}\{L_{\mathbf{Y}^o}(\mathbf{Y}^o,\mathbf{X}^o,M,A,N,\boldsymbol{C})|\mathbf{X}^o,M,A,N,\boldsymbol{C}\} = \mathbb{E}\{L_{\mathbf{X}^o}(\mathbf{X}^o,M,A,N,\boldsymbol{C})|M,N,\boldsymbol{C}\} \\
&= \mathbb{E}\{L_M(M,N,\boldsymbol{C},A)|A,\boldsymbol{C},N\} = \mathbb{E}\{L_{\boldsymbol{C}}(\boldsymbol{C},N)|N\} = \mathbb{E}\{L_N(N)\} = 0.
\end{aligned}$$

The uniform subsampling assumption in Assumption S1, i.e.,

$$\mathbb{P}\{\boldsymbol{S}(a) = \boldsymbol{s}|\mathbf{Y}(a),M(a),\mathbf{X},N,\boldsymbol{C}\} = \binom{N}{M(a)}^{-1},$$

does not restrict the observed data tangent space since no parametric assumption is made on $(\mathbf{Y},\mathbf{X})$ and the vector $\boldsymbol{S}$ is unobserved. Therefore, Assumption S1 does not constrain the choice of parametric submodels for the distribution

$\mathcal{P}(\mathbf{Y}^o|\mathbf{X}^o, M, A, N, \boldsymbol{C}) \times \mathcal{P}(\mathbf{X}^o|M, N, \boldsymbol{C})$. We then decompose $\varphi^{\text{eff}}_{C,a}(\mathcal{O})$ as

$$\begin{aligned}\varphi^{\text{eff}}_{C,a}(\mathcal{O}) = \varphi^{\text{eff}}_{C,a,\mathbf{Y}^o}(\mathbf{Y}^o, \mathbf{X}^o, M, A, N, \boldsymbol{C}) + \varphi^{\text{eff}}_{C,a,\mathbf{X}^o}(\mathbf{X}^o, M, A, N, \boldsymbol{C}) + \varphi^{\text{eff}}_{C,a,M}(M, N, \boldsymbol{C}, A) \\ + \varphi^{\text{eff}}_{C,a,M}(M, N, \boldsymbol{C}, A) + \varphi^{\text{eff}}_{C,a,\boldsymbol{C}}(\boldsymbol{C}, N) + \varphi^{\text{eff}}_{C,a,N}(N),\end{aligned}$$

where

$$\begin{aligned}
\varphi^{\text{eff}}_{C,a,\mathbf{Y}^o}(\mathbf{Y}^o, \mathbf{X}^o, M, A, N, \boldsymbol{C}) &= \frac{\mathbb{1}(A=a)}{\pi^a(1-\pi)^{1-a}} \left[\mathfrak{w}_{C,a,a}(\mathbf{Y}^o) - \mathbb{E}\left\{\mathfrak{w}_{C,a,a}(\mathbf{Y}^o)|\mathbf{X}^o, M, \boldsymbol{C}, N, A=a\right\}\right] \\
&\quad + \frac{\mathbb{1}(A=1-a)}{\pi^{1-a}(1-\pi)^{a}} \left[\mathfrak{w}_{C,a,1-a}(\mathbf{Y}^o) - \mathbb{E}\left\{\mathfrak{w}_{C,a,1-a}(\mathbf{Y}^o)|\mathbf{X}^o, M, \boldsymbol{C}, N, A=1-a\right\}\right], \\
\varphi^{\text{eff}}_{C,a,\mathbf{X}^o}(\mathbf{X}^o, M, A, N, \boldsymbol{C}) &= \frac{\mathbb{P}(A=a|M, \boldsymbol{C}, N)}{\pi^a(1-\pi)^{1-a}} \left[\mathbb{E}\left\{\mathfrak{w}_{C,a,a}(\mathbf{Y}^o)|\mathbf{X}^o, M, \boldsymbol{C}, N, A=a\right\}\right. \\
&\qquad \left. -\mathbb{E}\left\{\mathfrak{w}_{C,a,a}(\mathbf{Y}^o)|M, \boldsymbol{C}, N, A=a\right\}\right] \\
&\quad + \frac{\mathbb{P}(A=1-a|M, \boldsymbol{C}, N)}{\pi^{1-a}(1-\pi)^{a}} \left[\mathbb{E}\left\{\mathfrak{w}_{C,a,1-a}(\mathbf{Y}^o)|\mathbf{X}^o, M, \boldsymbol{C}, N, A=1-a\right\}\right. \\
&\qquad \left. -\mathbb{E}\left\{\mathfrak{w}_{C,a,1-a}(\mathbf{Y}^o)|M, \boldsymbol{C}, N, A=1-a\right\}\right], \\
\varphi^{\text{eff}}_{C,a,M}(M, N, \boldsymbol{C}, A) &= \frac{\mathbb{1}(A=a)}{\pi^a(1-\pi)^{1-a}} \left[\mathbb{E}\left\{\mathfrak{w}_{C,a,a}(\mathbf{Y}^o)|M, \boldsymbol{C}, N, A=a\right\} - \mathbb{E}\left\{\mathfrak{w}_{C,a,a}(\mathbf{Y}^o)|\boldsymbol{C}, N, A=a\right\}\right] \\
&\quad + \frac{\mathbb{1}(A=1-a)}{\pi^{1-a}(1-\pi)^{a}} \left[\mathbb{E}\left\{\mathfrak{w}_{C,a,1-a}(\mathbf{Y}^o)|M, \boldsymbol{C}, N, A=1-a\right\}\right. \\
&\qquad \left. -\mathbb{E}\left\{\mathfrak{w}_{C,a,1-a}(\mathbf{Y}^o)|\boldsymbol{C}, N, A=1-a\right\}\right], \\
\varphi^{\text{eff}}_{C,a,\boldsymbol{C}}(\boldsymbol{C}, N) &= \mathbb{E}\left\{\mathfrak{w}_{C,a,a}(\mathbf{Y}^o)|\boldsymbol{C}, N, A=a\right\} + \mathbb{E}\left\{\mathfrak{w}_{C,a,1-a}(\mathbf{Y}^o)|\boldsymbol{C}, N, A=a\right\} \\
&\quad - \mathbb{E}\left\{\mathfrak{w}_{C,a,a}(\mathbf{Y}^o)|\boldsymbol{C}, A=a\right\} - \mathbb{E}\left\{\mathfrak{w}_{C,a,1-a}(\mathbf{Y}^o)|\boldsymbol{C}, A=a\right\}, \\
\varphi^{\text{eff}}_{C,a,N}(N) &= \mathbb{E}\left\{\mathfrak{w}_{C,a,a}(\mathbf{Y}^o)|\boldsymbol{C}, A=a\right\} + \mathbb{E}\left\{\mathfrak{w}_{C,a,1-a}(\mathbf{Y}^o)|\boldsymbol{C}, A=a\right\} - 2\lambda_{C,a}.
\end{aligned}$$

Some algebra gives us

$$\begin{aligned}&\mathbb{E}\left\{\varphi^{\text{eff}}_{C,a,\mathbf{Y}^o}(\mathbf{Y}^o, \mathbf{X}^o, M, A, N, \boldsymbol{C})|\mathbf{X}^o, M, A, N, \boldsymbol{C}\right\} = \mathbb{E}\left\{\varphi^{\text{eff}}_{C,a,\mathbf{X}^o}(\mathbf{X}^o, M, A, N, \boldsymbol{C})|M, N, \boldsymbol{C}\right\} \\ &= \mathbb{E}\left\{\varphi^{\text{eff}}_{C,a,M}(M, N, \boldsymbol{C}, A)|A, \boldsymbol{C}, N\right\} = \mathbb{E}\left\{\varphi^{\text{eff}}_{C,a,\boldsymbol{C}}(\boldsymbol{C}, N)|N\right\} = \mathbb{E}\left\{\varphi^{\text{eff}}_{C,a,N}(N)\right\} = 0,\end{aligned}$$

which implies that $\varphi^{\text{eff}}_{C,a}(\mathcal{O}) \in \mathcal{T}$, completing the verification. The verification of $\varphi^{\text{eff}}_{I,a}(\mathcal{O}) \in \mathcal{T}$ follows the same process, and is thus omitted. □

### S8.3.4 The triply robust estimators

*Proof of Theorem S3.* By definition, $\widehat{\boldsymbol{\vartheta}} = (\widehat{\boldsymbol{\vartheta}}_1, \widehat{\boldsymbol{\vartheta}}_0)$ is obtained by solving estimating equations

$$\sum_{1 \le i < k \le m} \boldsymbol{\psi}_{\boldsymbol{\vartheta}}(\mathcal{O}_i, \mathcal{O}_k; \boldsymbol{\vartheta}) = \sum_{1 \le i < k \le m} \left\{ \begin{array}{c} \boldsymbol{\psi}_{\boldsymbol{\vartheta},1}(\mathcal{O}_i, \mathcal{O}_k; \boldsymbol{\vartheta}_1) \\ \boldsymbol{\psi}_{\boldsymbol{\vartheta},0}(\mathcal{O}_i, \mathcal{O}_k; \boldsymbol{\vartheta}_0) \end{array} \right\} = \mathbf{0}.$$

Therefore, the joint estimating equations for $(\widehat{\boldsymbol{\vartheta}}, \widehat{\boldsymbol{\lambda}}_C)$ are

$$\sum_{1\le i<k\le m} \boldsymbol{\psi}_C^{\rm eff}(\mathcal{O}_i, \mathcal{O}_k; \boldsymbol{\vartheta}, \boldsymbol{\lambda}) = \sum_{1\le i<k\le m} \left\{ \begin{array}{l} \boldsymbol{\psi}_{\boldsymbol{\vartheta},1}(\mathcal{O}_i, \mathcal{O}_k; \boldsymbol{\vartheta}_1) \\ \boldsymbol{\psi}_{\boldsymbol{\vartheta},0}(\mathcal{O}_i, \mathcal{O}_k; \boldsymbol{\vartheta}_0) \\ \psi^{\rm eff}_{C,\boldsymbol{\lambda},1}(\mathcal{O}_i, \mathcal{O}_k; \boldsymbol{\vartheta}, \lambda_1) \\ \psi^{\rm eff}_{C,\boldsymbol{\lambda},0}(\mathcal{O}_i, \mathcal{O}_k; \boldsymbol{\vartheta}, \lambda_0) \end{array} \right\} = \mathbf{0},$$

where, for $a \in \{0,1\}$,

$$\begin{aligned}
\psi^{\rm eff}_{C,\boldsymbol{\lambda},a}(\mathcal{O}_i, \mathcal{O}_k; \boldsymbol{\vartheta}, \lambda_a) &= 2^{-1}\left[\frac{\mathbb{1}(A_i=a)\mathbb{1}(A_k=1-a)}{\pi(1-\pi)}\left\{\overline{w}(\mathbf{Y}_i^o, \mathbf{Y}_k^o) - \zeta^{\rm m1}_{ik,a}(\boldsymbol{\vartheta}^{\rm m1}_a)\right\}\right.\\
&+\frac{\mathbb{1}(A_k=a)\mathbb{1}(A_i=1-a)}{\pi(1-\pi)}\left\{\overline{w}(\mathbf{Y}_k^o, \mathbf{Y}_i^o) - \zeta^{\rm m1}_{ki,a}(\boldsymbol{\vartheta}^{\rm m1}_a)\right\} + \frac{\zeta^{\rm p}_{i,a}(\boldsymbol{\vartheta}^{\rm p}_a)\zeta^{\rm p}_{k,1-a}(\boldsymbol{\vartheta}^{\rm p}_{1-a})}{\pi(1-\pi)}\left\{\zeta^{\rm m1}_{ik,a}(\boldsymbol{\vartheta}^{\rm m1}_a) - \zeta^{\rm m2}_{ik,a}(\boldsymbol{\vartheta}^{\rm m2}_a)\right\}\\
&\left.+\frac{\zeta^{\rm p}_{i,1-a}(\boldsymbol{\vartheta}^{\rm p}_{1-a})\zeta^{\rm p}_{k,a}(\boldsymbol{\vartheta}^{\rm p}_a)}{\pi(1-\pi)}\left\{\zeta^{\rm m1}_{ki,a}(\boldsymbol{\vartheta}^{\rm m1}_a) - \zeta^{\rm m2}_{ki,a}(\boldsymbol{\vartheta}^{\rm m2}_a)\right\} + \zeta^{\rm m2}_{ik,a}(\boldsymbol{\vartheta}^{\rm m2}_a) + \zeta^{\rm m2}_{ki,a}(\boldsymbol{\vartheta}^{\rm m2}_a) - 2\lambda_a\right].
\end{aligned}$$

Under the regularity conditions in Section S1, we have $(\widehat{\boldsymbol{\vartheta}}, \widehat{\boldsymbol{\lambda}}^{\rm tr}_C) \xrightarrow{p} (\underline{\boldsymbol{\vartheta}}, \underline{\boldsymbol{\lambda}}^{\rm tr}_C)$ by Lemma S1, where $\underline{\boldsymbol{\lambda}}^{\rm tr}_C$ satisfies

$$\mathbb{E}\left\{\boldsymbol{\psi}^{\rm eff}_C(\mathcal{O}_i, \mathcal{O}_k; \underline{\boldsymbol{\vartheta}}, \underline{\boldsymbol{\lambda}}^{\rm tr}_C)\right\} = \mathbf{0}.$$

To see when $\underline{\lambda}^{\rm tr}_{C,a} = \lambda_{C,a}$, we have, by Lemma S3 and $A \perp (N, \boldsymbol{C})$,

$$\begin{aligned}
&\mathbb{E}\left\{\psi^{\rm eff}_{C,a}(\mathcal{O}_i, \mathcal{O}_k; \underline{\boldsymbol{\vartheta}}, \underline{\lambda}^{\rm tr}_{C,a})\right\}\\
&= \mathbb{E}\left[2^{-1}\left\{\frac{\mathbb{1}(A_i=a)\mathbb{1}(A_k=1-a)}{\pi(1-\pi)}\overline{w}(\mathbf{Y}_i^o, \mathbf{Y}_k^o) + \frac{\mathbb{1}(A_k=a)\mathbb{1}(A_i=1-a)}{\pi(1-\pi)}\overline{w}(\mathbf{Y}_k^o, \mathbf{Y}_i^o)\right\}\right]\\
&\quad - \mathbb{E}\left[2^{-1}\left\{\frac{\mathbb{1}(A_i=a)\mathbb{1}(A_k=1-a) - \zeta^{\rm p}_{i,a}(\underline{\boldsymbol{\vartheta}}^{\rm p}_a)\zeta^{\rm p}_{k,1-a}(\underline{\boldsymbol{\vartheta}}^{\rm p}_{1-a})}{\pi(1-\pi)}\zeta^{\rm m1}_{ik,a}(\underline{\boldsymbol{\vartheta}}^{\rm m1}_a)\right.\right.\\
&\qquad\qquad \left.\left.+\frac{\mathbb{1}(A_k=a)\mathbb{1}(A_i=1-a) - \zeta^{\rm p}_{i,1-a}(\underline{\boldsymbol{\vartheta}}^{\rm p}_{1-a})\zeta^{\rm p}_{k,a}(\underline{\boldsymbol{\vartheta}}^{\rm p}_a)}{\pi(1-\pi)}\zeta^{\rm m1}_{ki,a}(\underline{\boldsymbol{\vartheta}}^{\rm m1}_a)\right\}\right]\\
&\quad - \mathbb{E}\left(2^{-1}\left[\left\{\frac{\zeta^{\rm p}_{i,a}(\underline{\boldsymbol{\vartheta}}^{\rm p}_a)\zeta^{\rm p}_{k,1-a}(\underline{\boldsymbol{\vartheta}}^{\rm p}_{1-a})}{\pi(1-\pi)} - 1\right\}\zeta^{\rm m1}_{ik,a}(\underline{\boldsymbol{\vartheta}}^{\rm m1}_a) + \left\{\frac{\zeta^{\rm p}_{i,1-a}(\underline{\boldsymbol{\vartheta}}^{\rm p}_{1-a})\zeta^{\rm p}_{k,a}(\underline{\boldsymbol{\vartheta}}^{\rm p}_a)}{\pi(1-\pi)} - 1\right\}\zeta^{\rm m1}_{ki,a}(\underline{\boldsymbol{\vartheta}}^{\rm m1}_a)\right]\right) - \underline{\lambda}^{\rm tr}_{C,a}\\
&= \lambda_{C,a} - \mathbb{E}\left\{2^{-1}\left[\frac{\zeta^{\rm p,0}_{i,a}\zeta^{\rm p,0}_{k,1-a} - \zeta_{i,a}(\underline{\boldsymbol{\vartheta}}^{\rm p}_a)\zeta^{\rm p}_{k,1-a}(\underline{\boldsymbol{\vartheta}}^{\rm p}_{1-a})}{\pi(1-\pi)}\left\{\zeta^{\rm m1}_{ik,a}(\underline{\boldsymbol{\vartheta}}^{\rm m1}_a) - \zeta^{\rm m2}_{ik,a}(\underline{\boldsymbol{\vartheta}}^{\rm m2}_a)\right\}\right.\right.\\
&\qquad\qquad \left.\left.+\frac{\zeta^{\rm p,0}_{i,1-a}\zeta^{\rm p,0}_{k,a} - \zeta^{\rm p}_{i,1-a}(\underline{\boldsymbol{\vartheta}}^{\rm p}_{1-a})\zeta^{\rm p}_{k,a}(\underline{\boldsymbol{\vartheta}}^{\rm p}_a)}{\pi(1-\pi)}\left\{\zeta^{\rm m1}_{ki,a}(\underline{\boldsymbol{\vartheta}}^{\rm m1}_a) - \zeta^{\rm m2}_{ki,a}(\underline{\boldsymbol{\vartheta}}^{\rm m2}_a)\right\}\right]\right\} - \underline{\lambda}^{\rm tr}_{C,a}.
\end{aligned}$$

Given the condition that (i) $\zeta^{\rm p}_a(\underline{\boldsymbol{\vartheta}}^{\rm p}_a) = \zeta^{\rm p,0}_a$ or (ii) $\mathbb{E}\{\zeta^{\rm m1}_a(\underline{\boldsymbol{\vartheta}}^{\rm m1}_a)|M_i, M_k, N_i, N_k, \boldsymbol{C}_i, \boldsymbol{C}_k\} = \zeta^{\rm m2}_a(\underline{\boldsymbol{\vartheta}}^{\rm m2}_a)$, we obtain $\underline{\lambda}^{\rm tr}_{C,a} = \lambda_{C,a}$. To briefly verify the triple robustness property of $\widehat{\lambda}^{\rm tr}_C$, it suffices to discuss the case where $\widehat{\zeta}^{\rm m1}_a$ and $\widehat{\zeta}^{\rm m2}_a$ are consistent, whereas $\widehat{\zeta}^{\rm p}_a$ may not be. In fact, this case satisfies condition (ii), since $\mathbb{E}\{\zeta^{\rm m1}_a(\underline{\boldsymbol{\vartheta}}^{\rm m1}_a)|M_i, M_k, N_i, N_k, \boldsymbol{C}_i, \boldsymbol{C}_k\} = \mathbb{E}(\zeta^{\rm m1,0}_a|M_i, M_k, N_i, N_k, \boldsymbol{C}_i, \boldsymbol{C}_k) = \zeta^{\rm m2,0}_a = \zeta^{\rm m2}_a(\underline{\boldsymbol{\vartheta}}^{\rm m2}_a)$. Therefore, if at least two nuisance functions are correctly specified by the parametric working models, $\widehat{\lambda}^{\rm tr}_C$ is consistent.

We next prove the asymptotic normality. By the regularity conditions, Lemma S1 implies that

$$m^{1/2}(\widehat{\boldsymbol{\theta}}_C^{\text{tr}} - \underline{\boldsymbol{\theta}}_C^{\text{tr}}) = \frac{2}{\sqrt{m}} \sum_{i=1}^{m} \left(\underline{\boldsymbol{B}}_{C,\boldsymbol{\theta}}^{\text{tr}}\right)^{-1} \overline{\boldsymbol{\psi}}_C^{\text{eff}}(\mathcal{O}_i; \underline{\boldsymbol{\theta}}_C^{\text{tr}}) + \boldsymbol{o}_{\mathbb{P}}(1),$$

where $\widehat{\boldsymbol{\theta}}_C^{\text{tr}} = (\widehat{\boldsymbol{\vartheta}}^\top, \widehat{\boldsymbol{\lambda}}_C^{\text{tr}\prime})^\top$ and $\underline{\boldsymbol{B}}_{C,\boldsymbol{\theta}}^{\text{tr}} = \mathbb{E}\{\nabla_{\boldsymbol{\theta}} \boldsymbol{\psi}_C^{\text{eff}}(\mathcal{O}_i, \mathcal{O}_k; \underline{\boldsymbol{\theta}}_C^{\text{tr}})\}$. Thus, the asymptotic normality of $\widehat{\boldsymbol{\theta}}_C$ is obtained by the CLT. The asymptotic covariance matrix of $m^{1/2}\widehat{\boldsymbol{\theta}}_C^{\text{tr}}$ is $\underline{\boldsymbol{V}}_{C,\boldsymbol{\theta}}^{\text{tr}} = (\underline{\boldsymbol{B}}_{C,\boldsymbol{\theta}}^{\text{tr}})^{-1} \underline{\boldsymbol{\Sigma}}_{C,\boldsymbol{\theta}}^{\text{tr}} \{(\underline{\boldsymbol{B}}_{C,\boldsymbol{\theta}}^{\text{tr}})^{-1}\}^\top$, where $\underline{\boldsymbol{\Sigma}}_{C,\boldsymbol{\theta}}^{\text{tr}} = 4\mathbb{V}\text{ar}\{\overline{\boldsymbol{\psi}}_C^{\text{eff}}(\mathcal{O}_i; \underline{\boldsymbol{\theta}}_C^{\text{tr}})\}$ and $\overline{\boldsymbol{\psi}}_C^{\text{eff}}(\mathcal{O}_i; \underline{\boldsymbol{\theta}}_C^{\text{tr}}) = \mathbb{E}\{\boldsymbol{\psi}_C^{\text{eff}}(\mathcal{O}_i, \mathcal{O}_k; \underline{\boldsymbol{\theta}}_C^{\text{tr}}) | \mathcal{O}_i\}$. We further investigate the influence function of $\widehat{\boldsymbol{\lambda}}_C^{\text{tr}}$ to obtain explicit expressions of the asymptotic covariance matrix and covariance estimator. Specifically, we have

$$\underline{\boldsymbol{B}}_{C,\boldsymbol{\theta}}^{\text{tr}} = \begin{pmatrix} \underline{\boldsymbol{B}}_{\boldsymbol{\vartheta}\boldsymbol{\vartheta}} & \underline{\boldsymbol{B}}_{\boldsymbol{\vartheta}\boldsymbol{\lambda}} \\ \underline{\boldsymbol{B}}_{C,\boldsymbol{\lambda}\boldsymbol{\vartheta}}^{\text{tr}} & \underline{\boldsymbol{B}}_{C,\boldsymbol{\lambda}\boldsymbol{\lambda}}^{\text{tr}} \end{pmatrix} = \begin{pmatrix} \underline{\boldsymbol{B}}_{\boldsymbol{\vartheta}\boldsymbol{\vartheta}} & \mathbf{0} \\ \underline{\boldsymbol{B}}_{C,\boldsymbol{\lambda}\boldsymbol{\vartheta}}^{\text{tr}} & \underline{\boldsymbol{B}}_{C,\boldsymbol{\lambda}\boldsymbol{\lambda}}^{\text{tr}} \end{pmatrix},$$

where $\underline{\boldsymbol{B}}_{\boldsymbol{\vartheta}\boldsymbol{\vartheta}} = \mathbb{E}\{\nabla_{\boldsymbol{\vartheta}} \boldsymbol{\psi}_{\boldsymbol{\vartheta}}(\mathcal{O}_i, \mathcal{O}_k; \underline{\boldsymbol{\vartheta}})\}$, $\underline{\boldsymbol{B}}_{\boldsymbol{\vartheta}\boldsymbol{\lambda}} = \mathbb{E}\{\nabla_{\boldsymbol{\lambda}} \boldsymbol{\psi}_{\boldsymbol{\vartheta}}(\mathcal{O}_i, \mathcal{O}_k; \underline{\boldsymbol{\vartheta}})\} = \mathbf{0}$, $\underline{\boldsymbol{B}}_{C,\boldsymbol{\lambda}\boldsymbol{\vartheta}}^{\text{tr}} = \mathbb{E}\{\nabla_{\boldsymbol{\vartheta}} \boldsymbol{\psi}_{C,\boldsymbol{\lambda}}^{\text{eff}}(\mathcal{O}_i, \mathcal{O}_k; \underline{\boldsymbol{\vartheta}}, \underline{\boldsymbol{\lambda}}_C^{\text{tr}})\}$, and $\underline{\boldsymbol{B}}_{C,\boldsymbol{\lambda}\boldsymbol{\lambda}}^{\text{tr}} = \mathbb{E}\{\nabla_{\boldsymbol{\lambda}} \boldsymbol{\psi}_{C,\boldsymbol{\lambda}}^{\text{eff}}(\mathcal{O}_i, \mathcal{O}_k; \underline{\boldsymbol{\vartheta}}, \underline{\boldsymbol{\lambda}}_C^{\text{tr}})\}$. Then, the inverse of the block lower-triangular matrix gives us

$$\left(\underline{\boldsymbol{B}}_{C,\boldsymbol{\theta}}^{\text{tr}}\right)^{-1} = \begin{pmatrix} \underline{\boldsymbol{B}}_{\boldsymbol{\vartheta}\boldsymbol{\vartheta}}^{-1} & \mathbf{0} \\ -\left(\underline{\boldsymbol{B}}_{C,\boldsymbol{\lambda}\boldsymbol{\lambda}}^{\text{tr}}\right)^{-1} \underline{\boldsymbol{B}}_{C,\boldsymbol{\lambda}\boldsymbol{\vartheta}}^{\text{tr}} \underline{\boldsymbol{B}}_{\boldsymbol{\vartheta}\boldsymbol{\vartheta}}^{-1} & \left(\underline{\boldsymbol{B}}_{C,\boldsymbol{\lambda}\boldsymbol{\lambda}}^{\text{tr}}\right)^{-1} \end{pmatrix}.$$

Since,

$$\overline{\boldsymbol{\psi}}_C^{\text{eff}}(\mathcal{O}_i; \boldsymbol{\theta}_C^{\text{tr}}) = \begin{pmatrix} \overline{\boldsymbol{\psi}}_{\boldsymbol{\vartheta}}(\mathcal{O}_i; \boldsymbol{\vartheta}) \\ \overline{\boldsymbol{\psi}}_{C,\boldsymbol{\lambda}}^{\text{eff}}(\mathcal{O}_i; \boldsymbol{\vartheta}, \boldsymbol{\lambda}_C^{\text{tr}}) \end{pmatrix},$$

by (S4), the influence function for $\widehat{\boldsymbol{\lambda}}_C^{\text{tr}}$ is

$$\boldsymbol{\varphi}_C^{\text{tr}}(\mathcal{O}_i; \boldsymbol{\vartheta}, \boldsymbol{\lambda}_C^{\text{tr}}) = -2\left(\boldsymbol{B}_{C,\boldsymbol{\lambda}\boldsymbol{\lambda}}^{\text{tr}}\right)^{-1} \left\{\overline{\boldsymbol{\psi}}_{C,\boldsymbol{\lambda}}^{\text{eff}}(\mathcal{O}_i; \boldsymbol{\vartheta}, \boldsymbol{\lambda}_C^{\text{tr}}) - \boldsymbol{B}_{C,\boldsymbol{\lambda}\boldsymbol{\vartheta}}^{\text{tr}} \boldsymbol{B}_{\boldsymbol{\vartheta}\boldsymbol{\vartheta}}^{-1} \overline{\boldsymbol{\psi}}_{\boldsymbol{\vartheta}}(\mathcal{O}_i; \boldsymbol{\vartheta})\right\}.$$

The asymptotic covariance matrix of $m^{1/2}\widehat{\boldsymbol{\lambda}}_C^{\text{tr}}$ is $\underline{\boldsymbol{V}}_C^{\text{tr}} = \mathbb{V}\text{ar}\{\boldsymbol{\varphi}_C^{\text{tr}}(\mathcal{O}_i; \underline{\boldsymbol{\vartheta}}, \underline{\boldsymbol{\lambda}}_C^{\text{tr}})\}$. The covariance matrix estimator $\widehat{\boldsymbol{V}}_C^{\text{tr}} = (m-1)^{-1}\sum_{i=1}^m \widehat{\boldsymbol{\varphi}}_C^{\text{tr}}(\mathcal{O}_i; \widehat{\boldsymbol{\vartheta}}, \widehat{\boldsymbol{\lambda}}_C^{\text{tr}}) \widehat{\boldsymbol{\varphi}}_C^{\text{tr}}(\mathcal{O}_i; \widehat{\boldsymbol{\vartheta}}, \widehat{\boldsymbol{\lambda}}_C^{\text{tr}})^\top$, where

$$\widehat{\boldsymbol{\varphi}}_C^{\text{tr}}(\mathcal{O}_i; \widehat{\boldsymbol{\vartheta}}, \widehat{\boldsymbol{\lambda}}_C^{\text{tr}}) = -2\left(\widehat{\boldsymbol{B}}_{C,\boldsymbol{\lambda}\boldsymbol{\lambda}}^{\text{tr}}\right)^{-1} \left\{\widehat{\boldsymbol{\psi}}_{C,\boldsymbol{\lambda}}^{\text{eff}}(\mathcal{O}_i; \widehat{\boldsymbol{\vartheta}}, \widehat{\boldsymbol{\lambda}}_C^{\text{tr}}) - \widehat{\boldsymbol{B}}_{C,\boldsymbol{\lambda}\boldsymbol{\vartheta}}^{\text{tr}} \widehat{\boldsymbol{B}}_{\boldsymbol{\vartheta}\boldsymbol{\vartheta}}^{-1} \widehat{\boldsymbol{\psi}}_{\boldsymbol{\vartheta}}(\mathcal{O}_i; \widehat{\boldsymbol{\vartheta}})\right\},$$

with

$$\widehat{\boldsymbol{B}}_{C,\boldsymbol{\lambda}\boldsymbol{\lambda}}^{\text{tr}} = \binom{m}{2}^{-1} \sum_{1 \le i < k \le m} \nabla_{\boldsymbol{\lambda}} \boldsymbol{\psi}_{C,\boldsymbol{\lambda}}^{\text{eff}}(\mathcal{O}_i, \mathcal{O}_k; \widehat{\boldsymbol{\vartheta}}, \widehat{\boldsymbol{\lambda}}_C^{\text{tr}}), \quad \widehat{\boldsymbol{B}}_{C,\boldsymbol{\lambda}\boldsymbol{\vartheta}}^{\text{tr}} = \binom{m}{2}^{-1} \sum_{1 \le i < k \le m} \nabla_{\boldsymbol{\vartheta}} \boldsymbol{\psi}_{C,\boldsymbol{\lambda}}^{\text{eff}}(\mathcal{O}_i, \mathcal{O}_k; \widehat{\boldsymbol{\vartheta}}, \widehat{\boldsymbol{\lambda}}_C^{\text{tr}}),$$

$$\widehat{\boldsymbol{B}}_{\boldsymbol{\vartheta}\boldsymbol{\vartheta}} = \binom{m}{2}^{-1} \sum_{1 \le i < k \le m} \nabla_{\boldsymbol{\vartheta}} \boldsymbol{\psi}_{\boldsymbol{\vartheta}}(\mathcal{O}_i, \mathcal{O}_k; \widehat{\boldsymbol{\vartheta}}), \quad \widehat{\boldsymbol{\psi}}_{C,\boldsymbol{\lambda}}^{\text{eff}}(\mathcal{O}_i; \widehat{\boldsymbol{\vartheta}}, \widehat{\boldsymbol{\lambda}}_C^{\text{tr}}) = \frac{1}{m-1} \sum_{k: k \ne i} \boldsymbol{\psi}_{C,\boldsymbol{\lambda}}^{\text{eff}}(\mathcal{O}_i, \mathcal{O}_k; \widehat{\boldsymbol{\vartheta}}, \widehat{\boldsymbol{\lambda}}_C^{\text{tr}}),$$

$$\widehat{\boldsymbol{\psi}}_{\boldsymbol{\vartheta}}(\mathcal{O}_i; \widehat{\boldsymbol{\vartheta}}) = \frac{1}{m-1} \sum_{k: k \ne i} \boldsymbol{\psi}_{\boldsymbol{\vartheta}}(\mathcal{O}_i, \mathcal{O}_k; \widehat{\boldsymbol{\vartheta}}).$$

The consistency and asymptotic normality of $\widehat{\Lambda}_C^{\text{tr}}$ are obtained via the continuous mapping theorem. The asymptotic variance estimators of $m^{1/2}\widehat{\Lambda}_C^{\text{tr}}$, $\widehat{V}_C^{\text{tr}}$, can be obtained by applying the Delta method to $\widehat{\boldsymbol{V}}_C^{\text{tr}}$. Lemma S1 implies that

$\widehat{V}_I^{\rm tr} \xrightarrow{p} \underline{V}_I^{\rm tr}$. Slutsky's theorem implies the result in the theorem statement.

For the semiparametric efficiency statement, note that

$$\underline{\boldsymbol{B}}_{C,\boldsymbol{\lambda}\boldsymbol{\vartheta}}^{\rm tr} = \mathbb{E}\left\{\nabla_{\boldsymbol{\vartheta}}\boldsymbol{\psi}_{C,\boldsymbol{\lambda}}^{\rm eff}(\mathcal{O}_i,\mathcal{O}_k;\underline{\boldsymbol{\vartheta}},\underline{\boldsymbol{\lambda}}_C^{\rm tr})\right\} = \mathbb{E}\left[\nabla_{\boldsymbol{\vartheta}}\mathbb{E}\left\{\boldsymbol{\psi}_{C,\boldsymbol{\lambda}}^{\rm eff}(\mathcal{O}_i,\mathcal{O}_k;\underline{\boldsymbol{\vartheta}},\underline{\boldsymbol{\lambda}}_C^{\rm tr})\Big|\mathcal{O}_i\right\}\right]$$
$$= \mathbb{E}\left\{2^{-1}\nabla_{\boldsymbol{\vartheta}}\boldsymbol{\varphi}_C^{\rm eff}(\mathcal{O}_i;\underline{\boldsymbol{\vartheta}},\underline{\boldsymbol{\lambda}}_C^{\rm tr})\right\},$$

which is equal to zero if the parametric working models correctly specify the nuisance functions, i.e., $\{\zeta^{\rm m1}(\underline{\boldsymbol{\vartheta}}^{\rm m1}), \zeta^{\rm m2}(\underline{\boldsymbol{\vartheta}}^{\rm m2}), \zeta^{\rm p}(\underline{\boldsymbol{\vartheta}}^{\rm p})\} = (\zeta^{\rm m1,0},\zeta^{\rm m2,0},\zeta^{\rm p,0})$, because of the Neyman orthogonality of the EIF. Therefore, if the parametric working models correctly specify the nuisance functions, $\underline{\boldsymbol{\lambda}}_C^{\rm tr} = \boldsymbol{\lambda}_C^0$, and

$$\boldsymbol{\varphi}_C^{\rm tr}(\mathcal{O}_i;\underline{\boldsymbol{\vartheta}},\boldsymbol{\lambda}_C^0) = -2\left(\underline{\boldsymbol{B}}_{C,\boldsymbol{\lambda}\boldsymbol{\lambda}}^{\rm tr}\right)^{-1}\mathbb{E}\left\{\boldsymbol{\psi}_{C,\boldsymbol{\lambda}}^{\rm eff}(\mathcal{O}_i,\mathcal{O}_k;\underline{\boldsymbol{\vartheta}},\boldsymbol{\lambda}_C^0)\Big|\mathcal{O}_i\right\} = \boldsymbol{\varphi}_C^{\rm eff}(\mathcal{O}_i;\underline{\boldsymbol{\vartheta}},\boldsymbol{\lambda}_C^0),$$

because $\underline{\boldsymbol{B}}_{C,\boldsymbol{\lambda}\boldsymbol{\lambda}}^{\rm tr} = -\boldsymbol{I}_2$, which proves the semiparametric efficient lower bound. The algebra is omitted.

Results for $\widehat{\boldsymbol{\lambda}}_I^{\rm tr}$, $\widehat{\Lambda}_I^{\rm tr}$, and their variance estimators, $\widehat{\boldsymbol{V}}_I^{\rm tr}$ and $\widehat{V}_I^{\rm tr}$, can be obtained following the same procedure. Here, we check the semiparametric efficiency lower bound. When the parametric working models correctly specify the nuisance functions, $\underline{\boldsymbol{B}}_{I,\boldsymbol{\lambda}\boldsymbol{\vartheta}}^{\rm tr} = \mathbb{E}\{\nabla_{\boldsymbol{\vartheta}}\boldsymbol{\psi}_{I,\boldsymbol{\lambda}}^{\rm eff}(\mathcal{O}_i,\mathcal{O}_k;\underline{\boldsymbol{\vartheta}},\boldsymbol{\lambda}_I^0)\} = \mathbb{E}[\nabla_{\boldsymbol{\vartheta}}\mathbb{E}\{\boldsymbol{\psi}_{I,\boldsymbol{\lambda}}^{\rm eff}(\mathcal{O}_i,\mathcal{O}_k;\underline{\boldsymbol{\vartheta}},\boldsymbol{\lambda}_I^0)|\mathcal{O}_i\}] = \mathbb{E}\{2^{-1}\nabla_{\boldsymbol{\vartheta}}\boldsymbol{\varphi}_I^{\text{eff-num}}(\mathcal{O}_i;\underline{\boldsymbol{\vartheta}},\boldsymbol{\lambda}_I^0)\} = \boldsymbol{0}$ because of the Neyman orthogonality of the EIF. Therefore,

$$\boldsymbol{\varphi}_I^{\rm tr}(\mathcal{O}_i;\underline{\boldsymbol{\vartheta}},\boldsymbol{\lambda}_I^0) = -2\left(\underline{\boldsymbol{B}}_{I,\boldsymbol{\lambda}\boldsymbol{\lambda}}^{\rm tr}\right)^{-1}\mathbb{E}\left\{\boldsymbol{\psi}_{I,\boldsymbol{\lambda}}^{\rm eff}(\mathcal{O}_i,\mathcal{O}_k;\underline{\boldsymbol{\vartheta}},\boldsymbol{\lambda}_I^0)\Big|\mathcal{O}_i\right\} = \boldsymbol{\varphi}_I^{\rm eff}(\mathcal{O}_i;\underline{\boldsymbol{\vartheta}},\boldsymbol{\lambda}_I^0),$$

since $\underline{\boldsymbol{B}}_{I,\boldsymbol{\lambda}\boldsymbol{\lambda}}^{\rm tr} = \mathbb{E}\{\nabla_{\boldsymbol{\lambda}}\boldsymbol{\psi}_{I,\boldsymbol{\lambda}}^{\rm eff}(\mathcal{O}_i,\mathcal{O}_k;\underline{\boldsymbol{\vartheta}},\boldsymbol{\lambda}_I^0)\} = -\mathbb{E}(N_iN_k)\times\boldsymbol{I}_2$. □

# References


Blom, G. (1976), "Some properties of incomplete U-statistics," *Biometrika*, 573–580.

Bugni, F., Canay, I. A., Shaikh, A. M., and Tabord-Meehan, M. (2025), "Inference for cluster randomized experiments with nonignorable cluster sizes," *Journal of Political Economy Microeconomics*, 3, 255–288.

Chow, Y. S. and Teicher, H. (1997), *Probability Theory: Independence, Interchangeability, Martingales*, Springer.

Durrett, R. and Durrett, R. (2019), *Probability: Theory and Examples*, Cambridge Series in Statistical and Probabilistic Mathematics, Cambridge, UK: Cambridge University Press.

Hines, O., Dukes, O., Diaz-Ordaz, K., and Vansteelandt, S. (2022), "Demystifying statistical learning based on efficient influence functions," *The American Statistician*, 76, 292–304.

Li, P. and Redden, D. T. (2015), "Small sample performance of bias-corrected sandwich estimators for cluster-randomized trials with binary outcomes," *Statistics in Medicine*, 34, 281–296.

Loève, M. (1977), *Probability Theory I*, Springer.

MacKinnon, J. G. and White, H. (1985), "Some heteroskedasticity-consistent covariance matrix estimators with improved finite sample properties," *Journal of Econometrics*, 29, 305–325.

Mao, L. (2017), "On causal estimation using U-statistics," *Biometrika*, 105, 215–220.

Newey, W. K. (1991), "Uniform convergence in probability and stochastic equicontinuity," *Econometrica*, 59, 1161–1167.

Smith, E. D., Jairath, V., and Zou, G. (2025), "Rank-based estimators of global treatment effects for cluster randomized trials with multiple endpoints on different scales," *Statistical Methods in Medical Research*, 34, 1267–1289. PMID: 40368381.

van der Vaart, A. (1998), *Asymptotic Statistics*, Cambridge, UK: Cambridge University Press.

Wang, B., Park, C., Small, D. S., and Li, F. (2024), "Model-robust and efficient covariate adjustment for cluster-randomized experiments," *Journal of the American Statistical Association*, 1–13. Published online ahead of print.
